# Supplementary material for: Search for effective Lorentz and CPT violation using ZEUS data
Source: arXiv:2212.12750 ancillary file (2022-12-24)
Supplement: Supplementary file 1 [file ZEUS_LV_supplemental.pdf]

DESY-22-107  
December 2022

Supplemental material for  
“Search for effective Lorentz and CPT violation  
using ZEUS data”

ZEUS Collaboration

| bin                    | 100    | 75     | 50     | 25     | 16     | 12     | 8      | 4      |
|------------------------|--------|--------|--------|--------|--------|--------|--------|--------|
| $\sigma_{\text{stat}}$ | 0.32%  | 0.27%  | 0.22%  | 0.16%  | 0.13%  | 0.11%  | 0.089% | 0.063% |
| 1                      | 1.0021 | 0.9975 | 0.9997 | 0.9995 | 0.9990 | 0.9985 | 0.9975 | 0.9983 |
| 2                      | 0.9974 | 1.0028 | 0.9994 | 0.9976 | 0.9960 | 0.9958 | 0.9991 | 0.9996 |
| 3                      | 1.0013 | 0.9982 | 0.9984 | 0.9956 | 0.9977 | 1.0006 | 1.0007 | 1.0003 |
| 4                      | 0.9974 | 0.9982 | 0.9968 | 0.9957 | 1.0005 | 1.0009 | 0.9985 | 1.0020 |
| 5                      | 0.9981 | 0.9991 | 0.9960 | 0.9990 | 1.0012 | 0.9995 | 1.0002 |        |
| 6                      | 0.9988 | 0.9957 | 0.9952 | 1.0011 | 1.0001 | 0.9983 | 1.0004 |        |
| 7                      | 0.9973 | 0.9947 | 0.9940 | 1.0002 | 0.9985 | 1.0010 | 1.0031 |        |
| 8                      | 0.9964 | 0.9988 | 0.9973 | 1.0019 | 0.9984 | 0.9988 | 1.0007 |        |
| 9                      | 0.9950 | 0.9933 | 0.9992 | 1.0011 | 1.0009 | 1.0010 |        |        |
| 10                     | 0.9970 | 0.9914 | 0.9988 | 0.9999 | 0.9995 | 1.0016 |        |        |
| 11                     | 0.9942 | 1.0002 | 0.9992 | 0.9975 | 0.9995 | 1.0045 |        |        |
| 12                     | 0.9963 | 0.9953 | 1.0029 | 0.9988 | 1.0012 | 0.9999 |        |        |
| 13                     | 0.9917 | 0.9996 | 1.0001 | 0.9982 | 1.0005 |        |        |        |
| 14                     | 0.9962 | 1.0019 | 1.0003 | 1.0021 | 1.0057 |        |        |        |
| 15                     | 0.9987 | 0.9955 | 1.0043 | 1.0015 | 1.0018 |        |        |        |
| 16                     | 0.9960 | 0.9972 | 0.9994 | 0.9970 | 0.9997 |        |        |        |
| 17                     | 0.9972 | 1.0041 | 1.0018 | 0.9985 |        |        |        |        |
| 18                     | 1.0012 | 1.0019 | 1.0003 | 0.9998 |        |        |        |        |
| 19                     | 1.0009 | 1.0025 | 1.0003 | 1.0027 |        |        |        |        |
| 20                     | 0.9966 | 0.9987 | 0.9995 | 1.0004 |        |        |        |        |
| 21                     | 0.9997 | 0.9995 | 0.9971 | 1.0043 |        |        |        |        |
| 22                     | 0.9988 | 1.0049 | 0.9979 | 1.0057 |        |        |        |        |
| 23                     | 1.0033 | 1.0024 | 0.9980 | 1.0023 |        |        |        |        |
| 24                     | 1.0025 | 0.9983 | 0.9996 | 1.0014 |        |        |        |        |
| 25                     | 1.0031 | 1.0015 | 0.9971 | 0.9983 |        |        |        |        |
| 26                     | 0.9971 | 1.0038 | 0.9994 |        |        |        |        |        |
| 27                     | 1.0014 | 0.9979 | 1.0017 |        |        |        |        |        |
| 28                     | 0.9993 | 0.9987 | 1.0025 |        |        |        |        |        |
| 29                     | 1.0048 | 1.0042 | 0.9992 |        |        |        |        |        |
| 30                     | 1.0038 | 0.9970 | 1.0039 |        |        |        |        |        |
| 31                     | 0.9994 | 0.9965 | 0.9976 |        |        |        |        |        |
| 32                     | 0.9995 | 0.9990 | 0.9964 |        |        |        |        |        |
| 33                     | 0.9999 | 0.9970 | 1.0006 |        |        |        |        |        |

**Table 1:** Central values for the ratio  $r(x_c)$  of normalised counts for  $x_c = 10^{-3}$  binned with the sidereal phase where  $N_{\text{bins}} = 4, 8, 12, 16, 25, 50, 75$  and  $100$ . In the top row, the statistical uncertainty per bin is presented.

| bin | 100    | 75     | 50     | 25 | 16 | 12 | 8 | 4 |
|-----|--------|--------|--------|----|----|----|---|---|
| 34  | 1.0038 | 0.9979 | 0.9964 |    |    |    |   |   |
| 35  | 1.0022 | 1.0003 | 0.9998 |    |    |    |   |   |
| 36  | 0.9985 | 0.9983 | 0.9998 |    |    |    |   |   |
| 37  | 0.9973 | 0.9960 | 1.0058 |    |    |    |   |   |
| 38  | 1.0034 | 0.9986 | 0.9994 |    |    |    |   |   |
| 39  | 1.0017 | 1.0002 | 1.0004 |    |    |    |   |   |
| 40  | 0.9973 | 1.0012 | 1.0004 |    |    |    |   |   |
| 41  | 0.9940 | 1.0015 | 1.0025 |    |    |    |   |   |
| 42  | 1.0004 | 1.0037 | 1.0062 |    |    |    |   |   |
| 43  | 1.0001 | 0.9983 | 1.0049 |    |    |    |   |   |
| 44  | 0.9956 | 1.0013 | 1.0066 |    |    |    |   |   |
| 45  | 0.9984 | 1.0051 | 0.9995 |    |    |    |   |   |
| 46  | 0.9977 | 0.9996 | 1.0051 |    |    |    |   |   |
| 47  | 1.0013 | 0.9912 | 1.0022 |    |    |    |   |   |
| 48  | 0.9979 | 1.0001 | 1.0005 |    |    |    |   |   |
| 49  | 0.9939 | 1.0033 | 0.9956 |    |    |    |   |   |
| 50  | 1.0005 | 0.9940 | 1.0011 |    |    |    |   |   |
| 51  | 0.9984 | 0.9981 |        |    |    |    |   |   |
| 52  | 1.0005 | 1.0012 |        |    |    |    |   |   |
| 53  | 1.0015 | 0.9988 |        |    |    |    |   |   |
| 54  | 1.0020 | 0.9995 |        |    |    |    |   |   |
| 55  | 1.0012 | 1.0088 |        |    |    |    |   |   |
| 56  | 1.0038 | 0.9998 |        |    |    |    |   |   |
| 57  | 1.0020 | 0.9993 |        |    |    |    |   |   |
| 58  | 0.9963 | 1.0017 |        |    |    |    |   |   |
| 59  | 1.0015 | 0.9963 |        |    |    |    |   |   |
| 60  | 1.0064 | 1.0031 |        |    |    |    |   |   |
| 61  | 0.9982 | 1.0013 |        |    |    |    |   |   |
| 62  | 0.9971 | 1.0067 |        |    |    |    |   |   |
| 63  | 0.9921 | 1.0048 |        |    |    |    |   |   |
| 64  | 1.0006 | 1.0055 |        |    |    |    |   |   |
| 65  | 1.0076 | 1.0045 |        |    |    |    |   |   |
| 66  | 0.9934 | 1.0073 |        |    |    |    |   |   |

**Table 2:** *Continued from Table 1.*

| bin | 100    | 75     | 50 | 25 | 16 | 12 | 8 | 4 |
|-----|--------|--------|----|----|----|----|---|---|
| 67  | 0.9952 | 0.9997 |    |    |    |    |   |   |
| 68  | 0.9976 | 1.0022 |    |    |    |    |   |   |
| 69  | 1.0038 | 1.0049 |    |    |    |    |   |   |
| 70  | 0.9960 | 0.9981 |    |    |    |    |   |   |
| 71  | 0.9979 | 1.0048 |    |    |    |    |   |   |
| 72  | 1.0017 | 1.0012 |    |    |    |    |   |   |
| 73  | 1.0099 | 0.9983 |    |    |    |    |   |   |
| 74  | 1.0018 | 0.9962 |    |    |    |    |   |   |
| 75  | 0.9999 | 1.0006 |    |    |    |    |   |   |
| 76  | 0.9990 |        |    |    |    |    |   |   |
| 77  | 1.0006 |        |    |    |    |    |   |   |
| 78  | 1.0003 |        |    |    |    |    |   |   |
| 79  | 0.9965 |        |    |    |    |    |   |   |
| 80  | 1.0041 |        |    |    |    |    |   |   |
| 81  | 0.9998 |        |    |    |    |    |   |   |
| 82  | 1.0051 |        |    |    |    |    |   |   |
| 83  | 1.0063 |        |    |    |    |    |   |   |
| 84  | 1.0061 |        |    |    |    |    |   |   |
| 85  | 1.0047 |        |    |    |    |    |   |   |
| 86  | 1.0051 |        |    |    |    |    |   |   |
| 87  | 1.0084 |        |    |    |    |    |   |   |
| 88  | 1.0048 |        |    |    |    |    |   |   |
| 89  | 1.0022 |        |    |    |    |    |   |   |
| 90  | 0.9966 |        |    |    |    |    |   |   |
| 91  | 1.0056 |        |    |    |    |    |   |   |
| 92  | 1.0046 |        |    |    |    |    |   |   |
| 93  | 0.9957 |        |    |    |    |    |   |   |
| 94  | 1.0087 |        |    |    |    |    |   |   |
| 95  | 0.9990 |        |    |    |    |    |   |   |
| 96  | 1.0021 |        |    |    |    |    |   |   |
| 97  | 0.9996 |        |    |    |    |    |   |   |
| 98  | 0.9918 |        |    |    |    |    |   |   |
| 99  | 0.9991 |        |    |    |    |    |   |   |
| 100 | 1.0030 |        |    |    |    |    |   |   |

**Table 3:** *Continued from Table 1.*

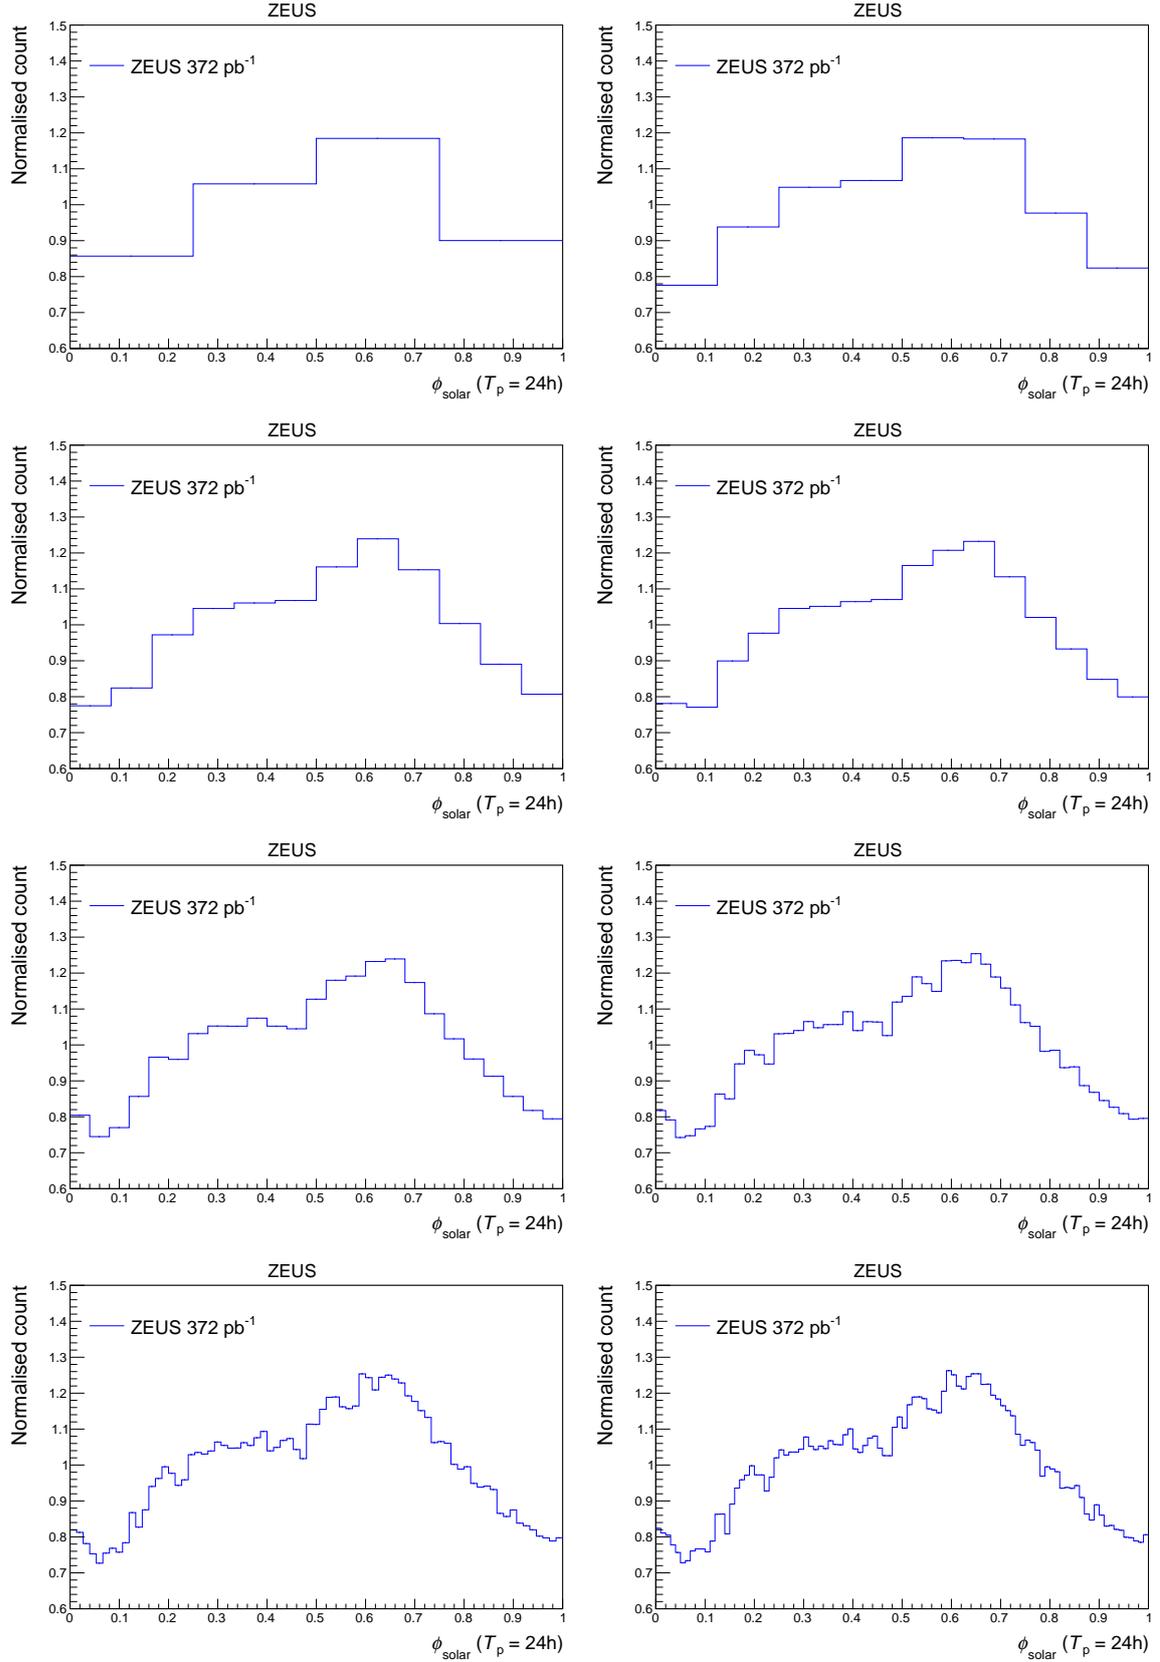

**Figure 1:** Solar phase dependence of the normalised counts in 4, 8, 12, 16, 25, 50, 75 and 100 bins for the kinematic region considered. The vertical axis displays the number of events per bin normalised to the total number of events times the bin width. Only statistical uncertainties are displayed.

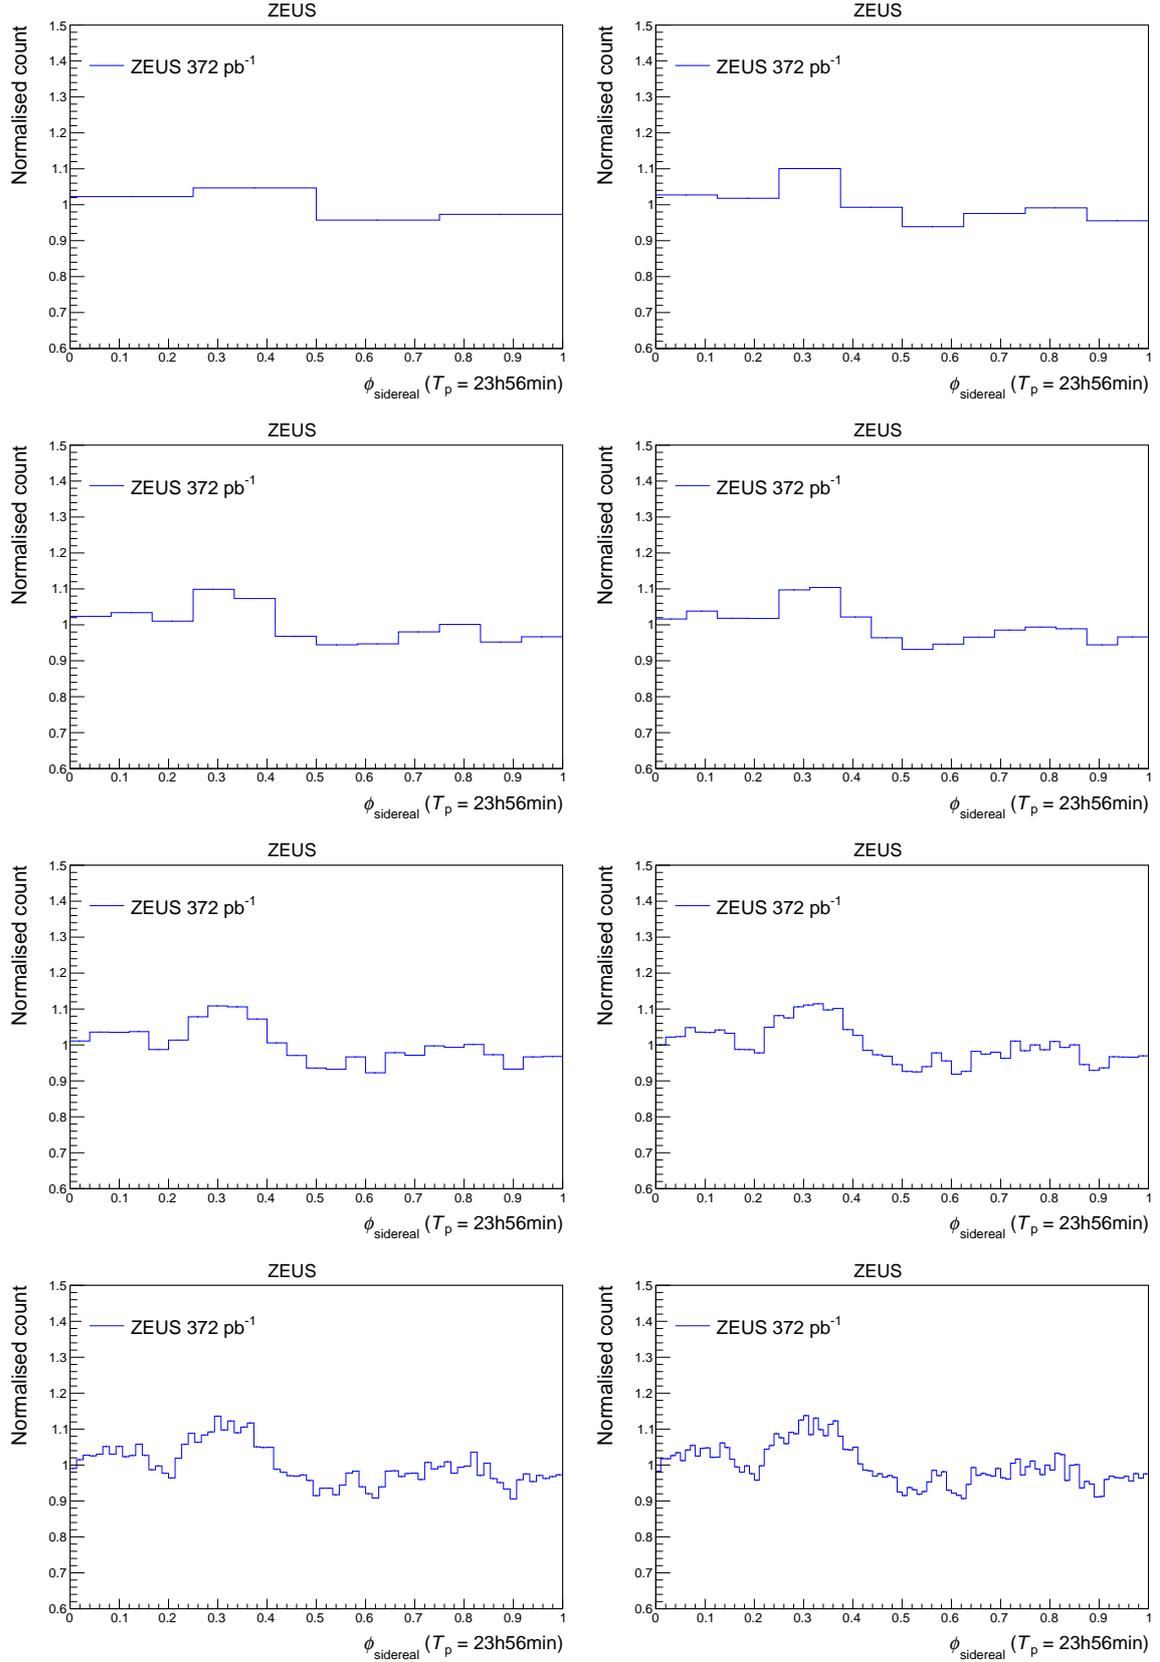

**Figure 2:** Sidereal phase dependence of the normalised counts in 4, 8, 12, 16, 25, 50, 75 and 100 bins for the kinematic range considered. The vertical axis displays the number of events per bin normalised to the total number of events times the bin width. Only statistical uncertainties are displayed.

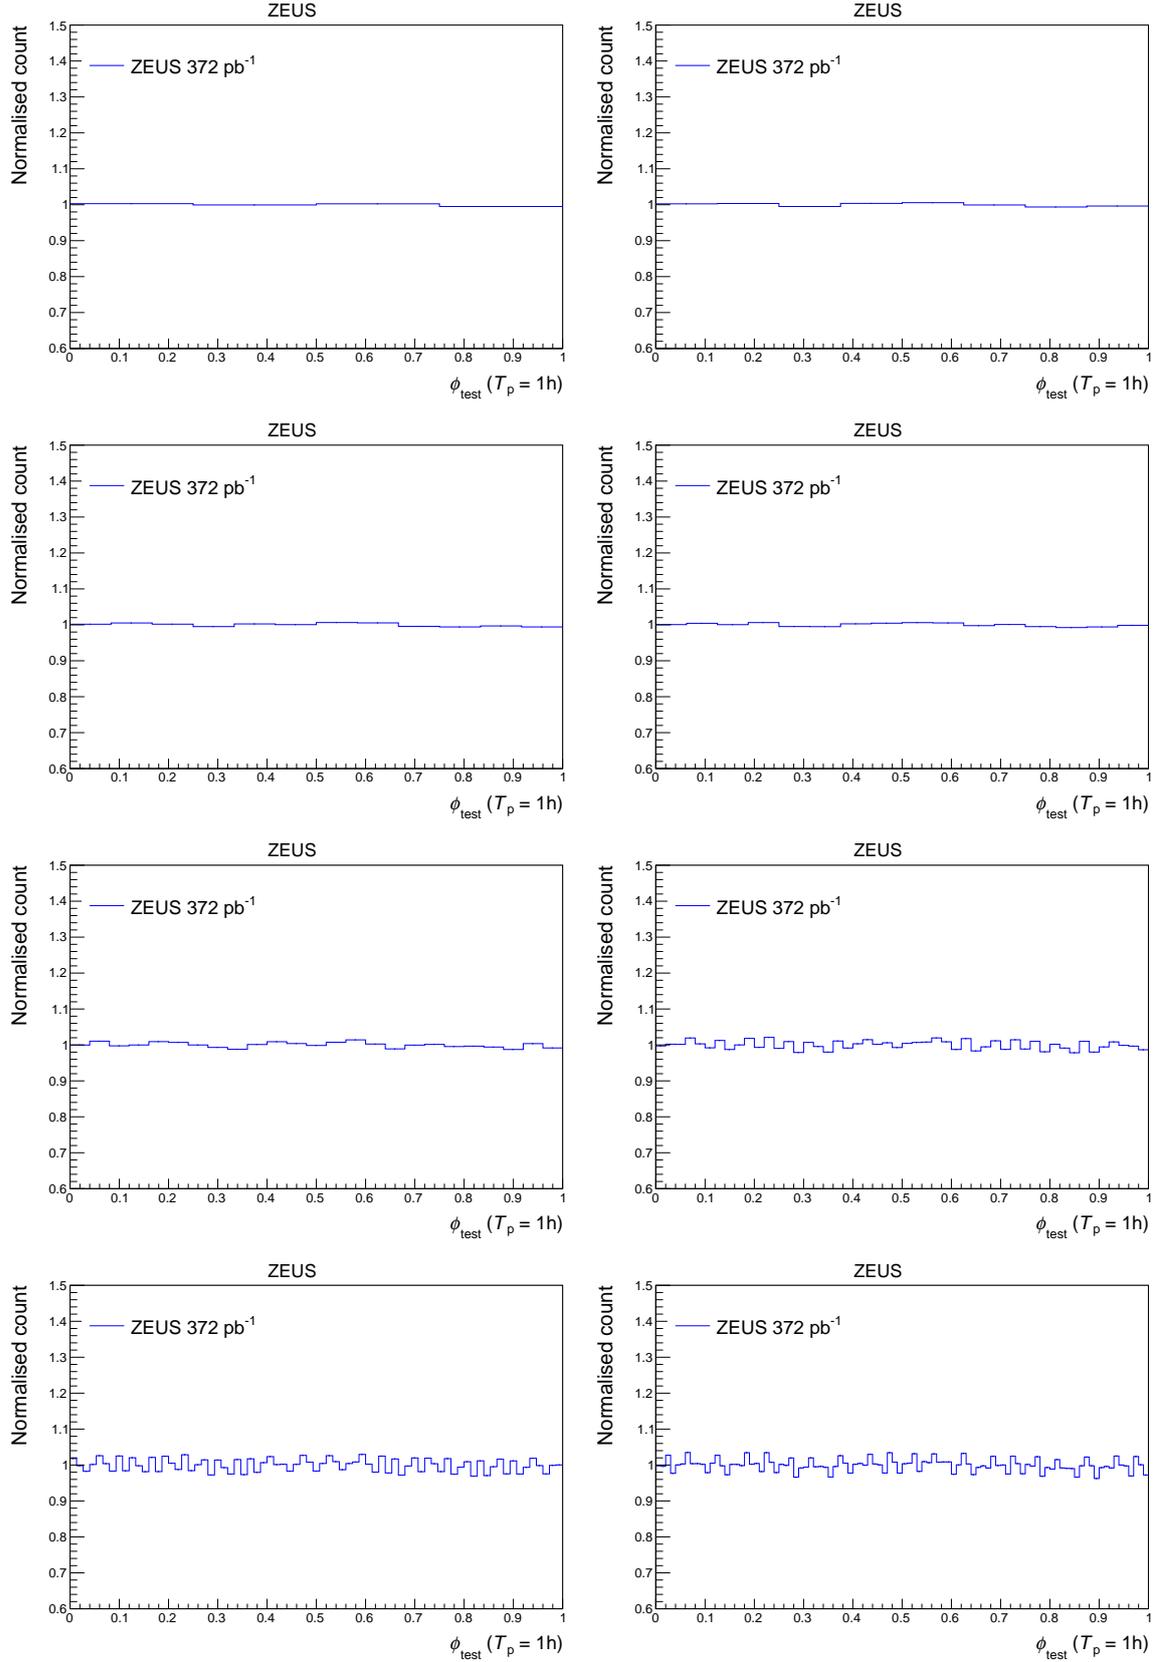

**Figure 3:**  $T_p = 1$  h phase dependence of the normalised counts in 4, 8, 12, 16, 25, 50, 75 and 100 bins for the kinematic region considered. The vertical axis displays the number of events per bin normalised to the total number of events times the bin width. Only statistical uncertainties are displayed.

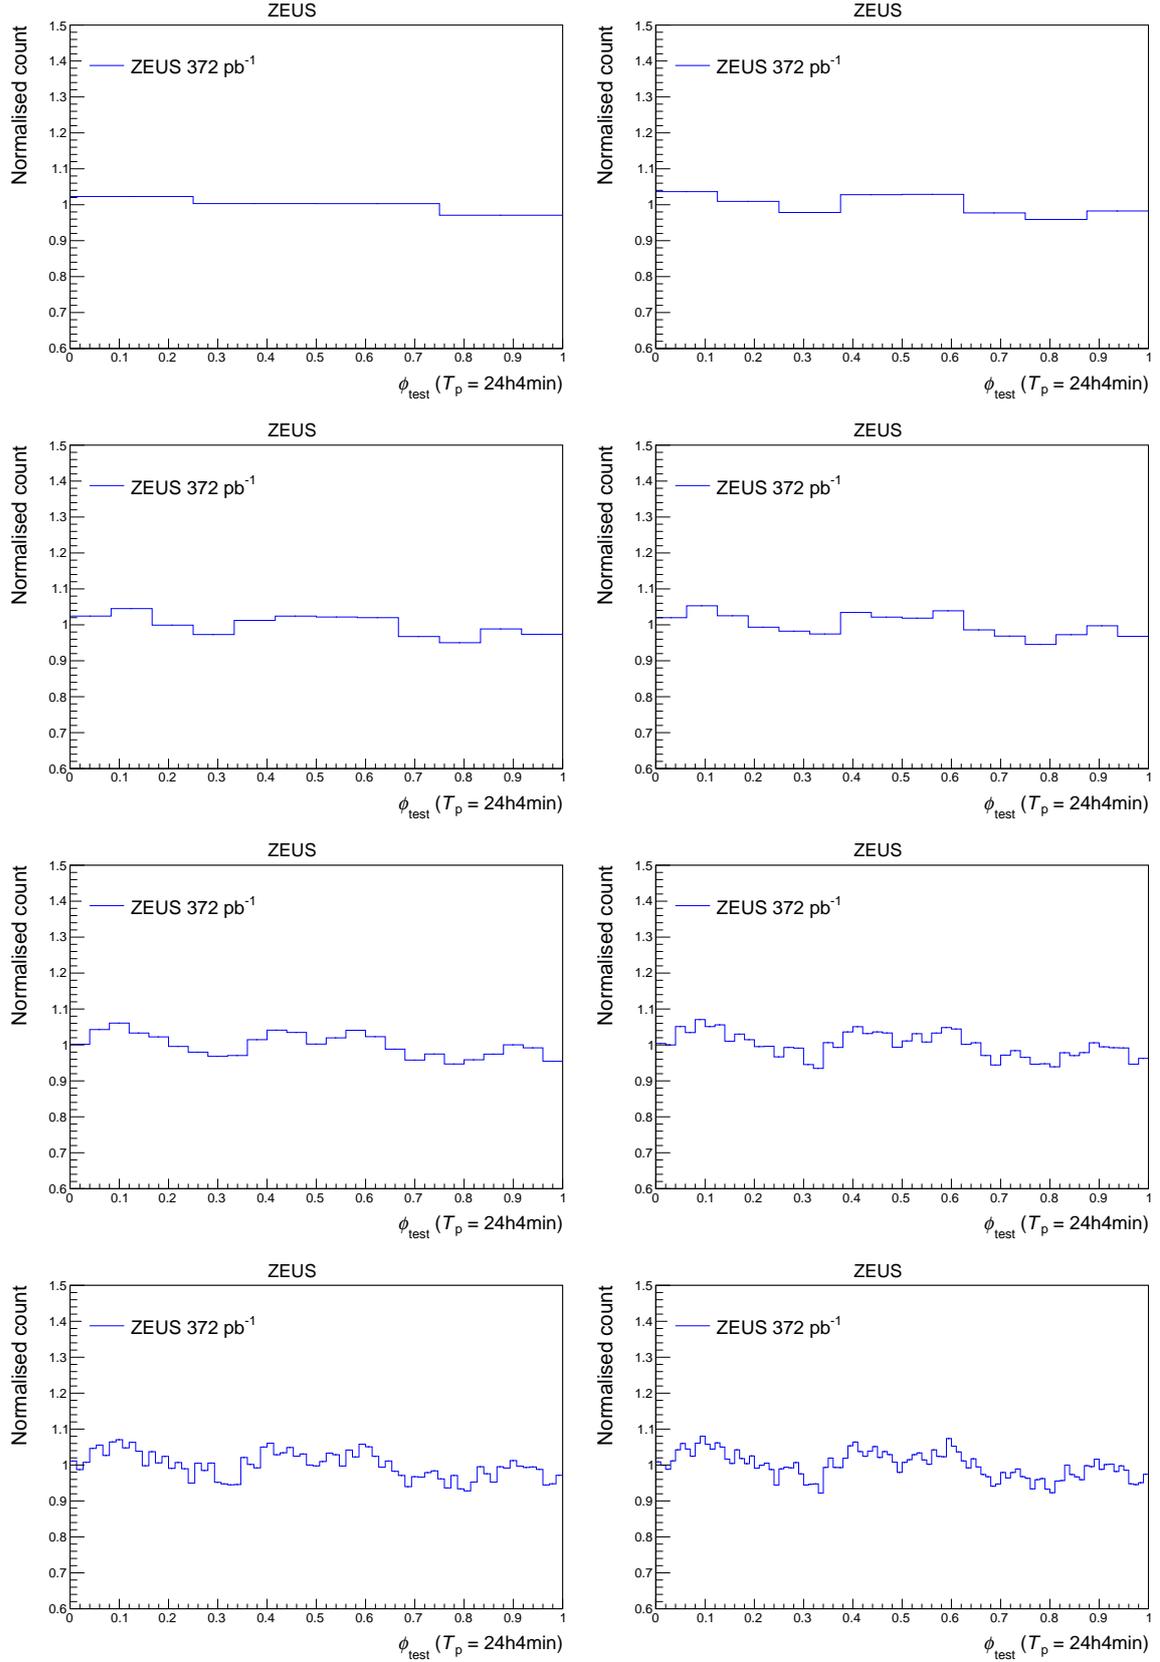

**Figure 4:**  $T_p = 24$  h 4 min phase dependence of the normalised counts in 4, 8, 12, 16, 25, 50, 75 and 100 bins for the kinematic region considered. The vertical axis displays the number of events per bin normalised to the total number of events times the bin width. Only statistical uncertainties are displayed.

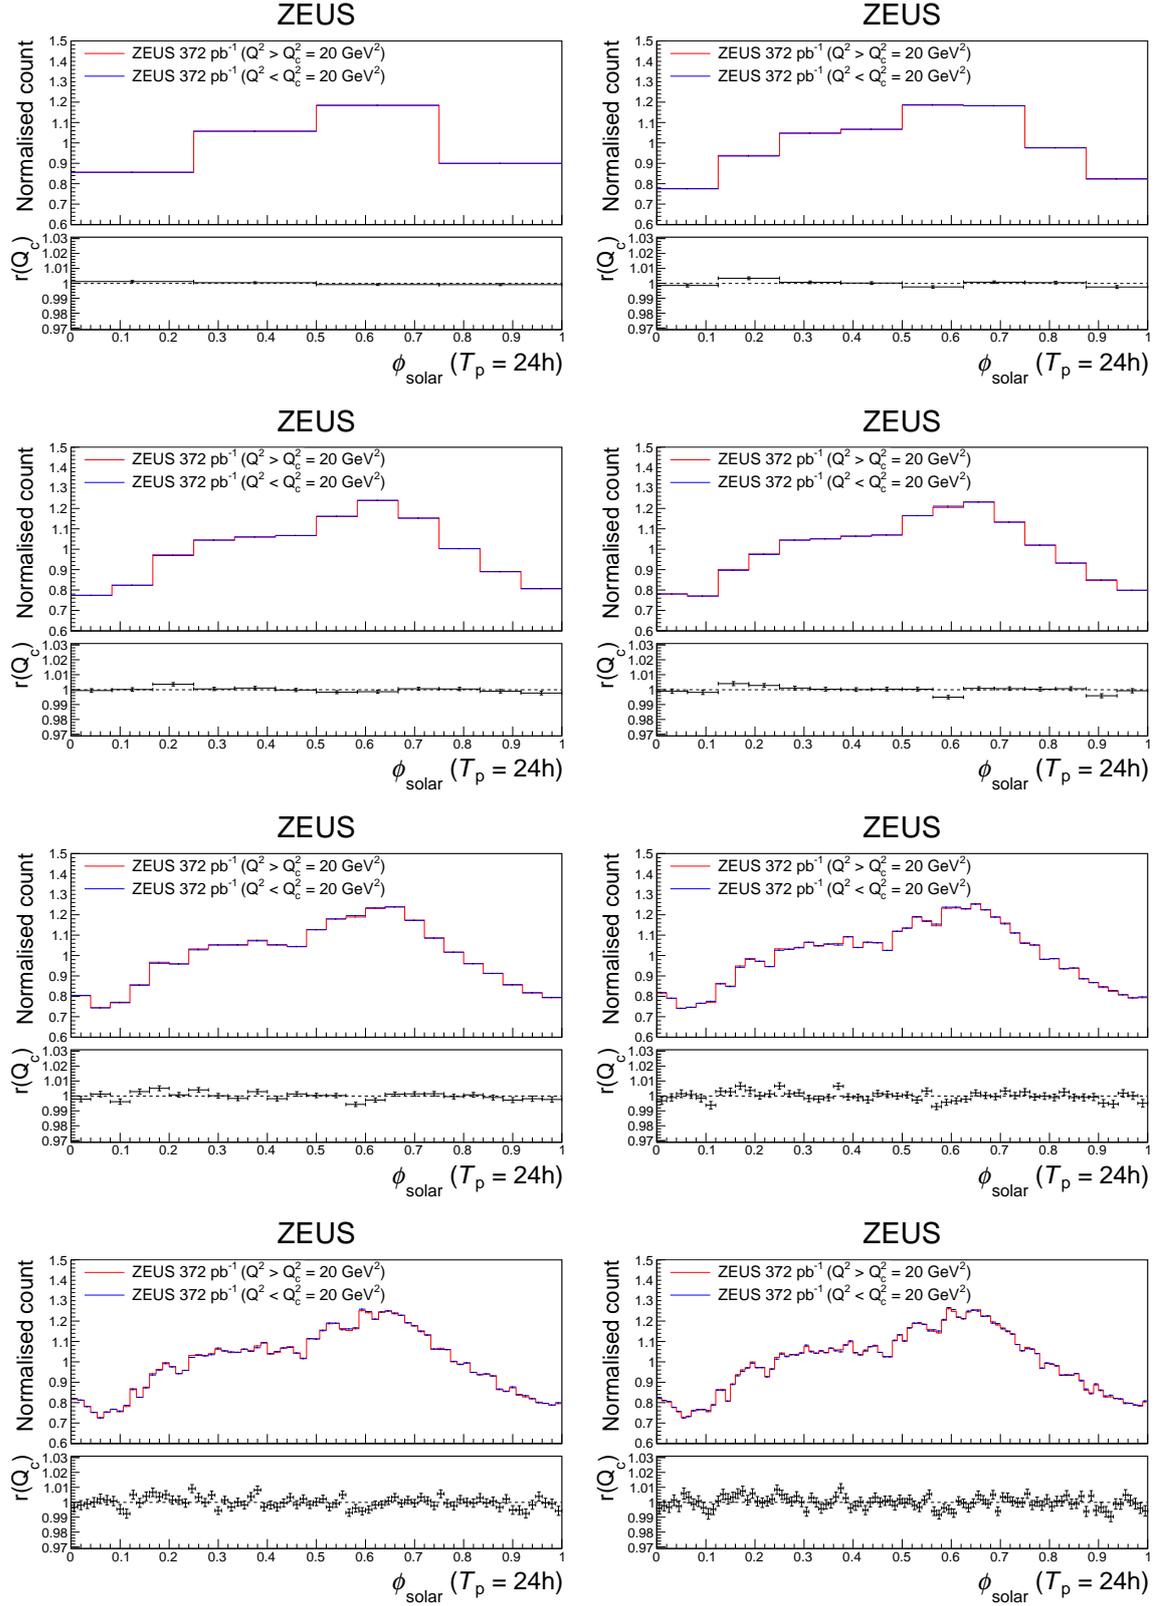

**Figure 5:** Solar phase dependence of the normalised counts in 4, 8, 12, 16, 25, 50, 75 and 100 bins with the kinematic region divided by  $Q_c^2 = 20 \text{ GeV}^2$ . The vertical axis displays the number of events per bin normalised to the total number of events times the bin width. The ratios of the counts  $r(Q_c)$  above and below  $Q_c^2$  are given in the bottom panels. For the solar phase,  $\phi_{\text{solar}} = 0$  is identified with 11:20 UTC. Only statistical uncertainties are displayed.

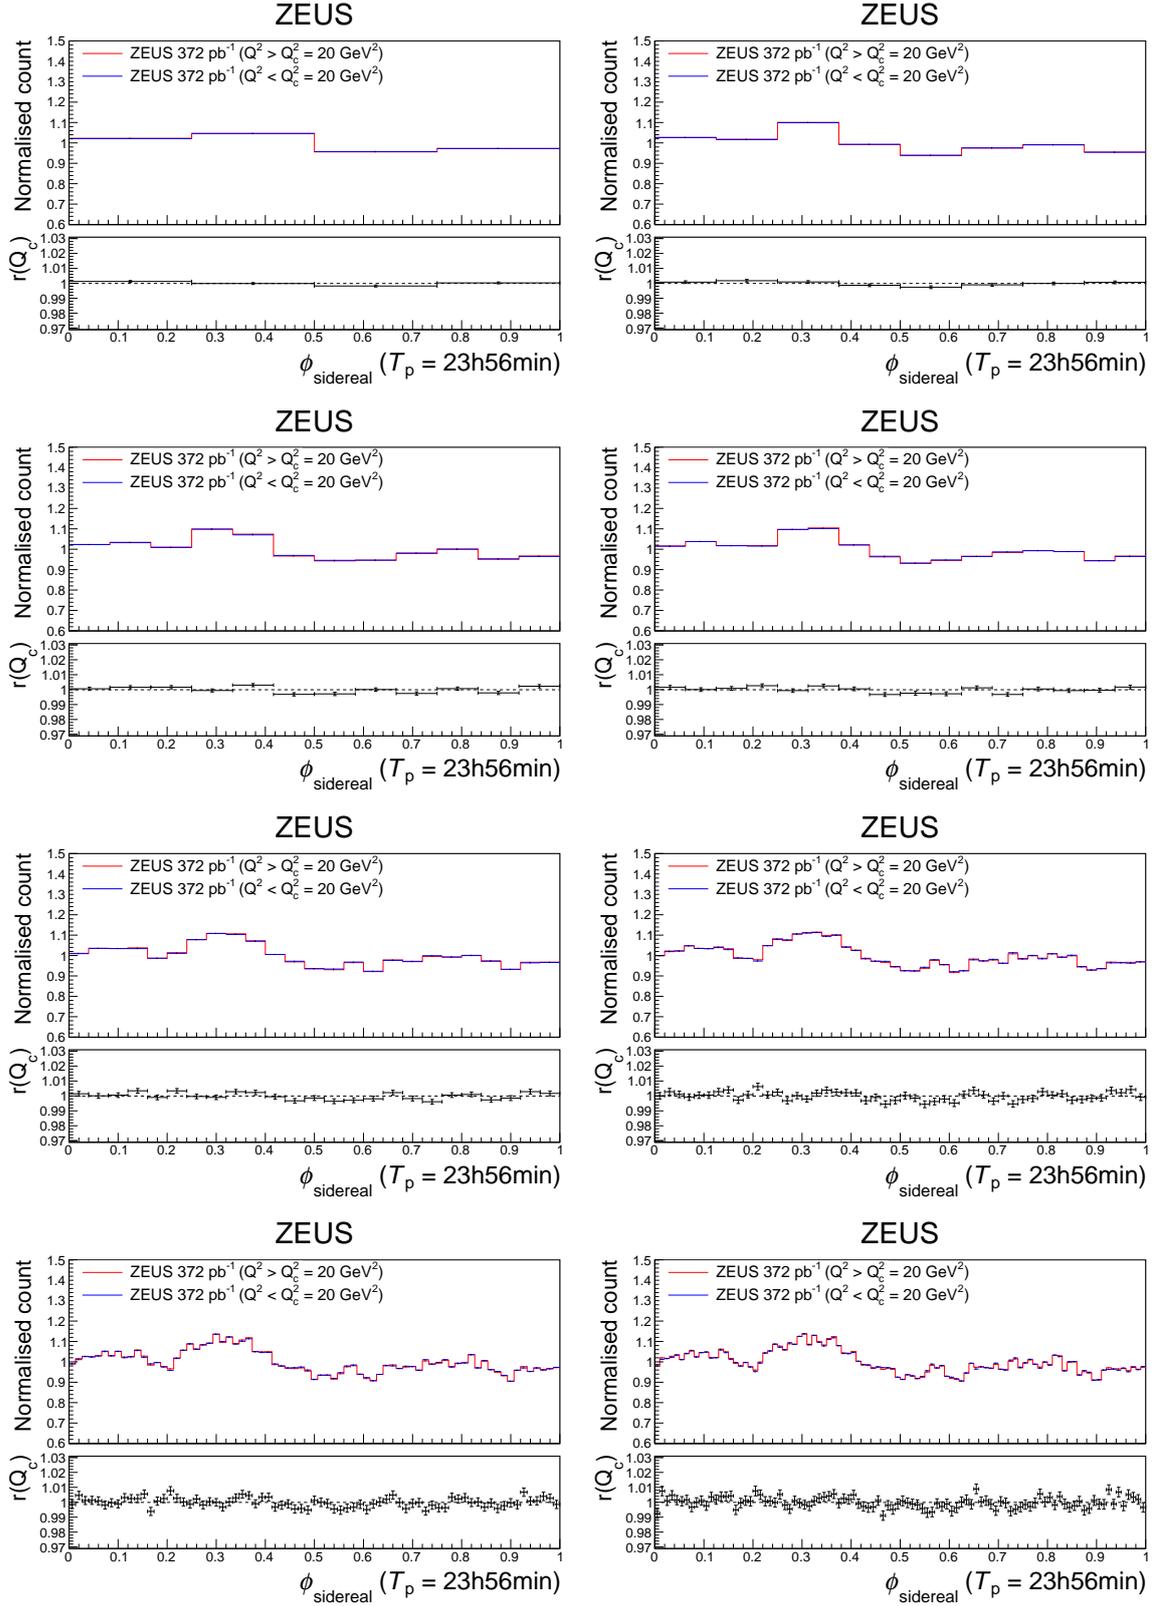

**Figure 6:** Sidereal phase dependence of the normalised counts in 4, 8, 12, 16, 25, 50, 75 and 100 bins with the kinematic region divided by  $Q_c^2 = 20 \text{ GeV}^2$ . The vertical axis displays the number of events per bin normalised to the total number of events times the bin width. The ratios of the counts  $r(Q_c)$  above and below  $Q_c^2$  are given in the bottom panels. Only statistical uncertainties are displayed.

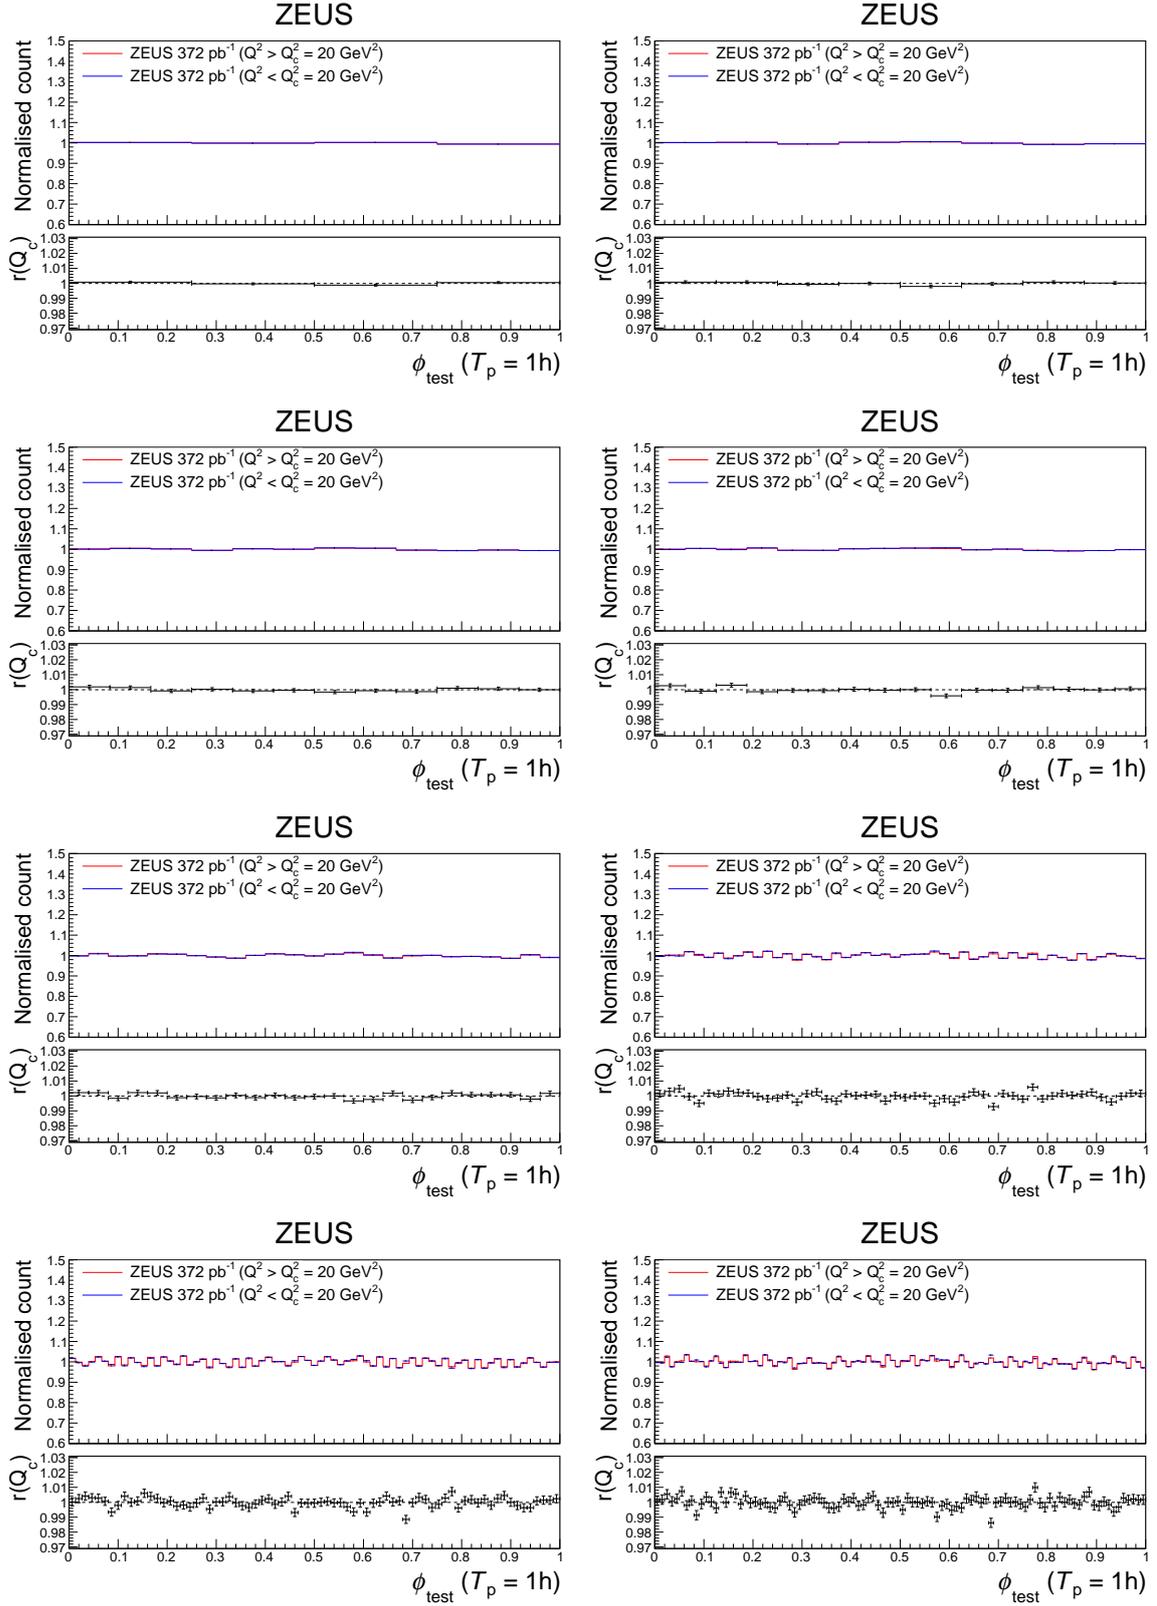

**Figure 7:**  $T_p = 1$  h phase dependence of the normalised counts in 4, 8, 12, 16, 25, 50, 75 and 100 bins with the kinematic region divided by  $Q_c^2 = 20 \text{ GeV}^2$ . The vertical axis displays the number of events per bin normalised to the total number of events times the bin width. The ratios of the counts  $r(Q_c)$  above and below  $Q_c^2$  are given in the bottom panels. Only statistical uncertainties are displayed.

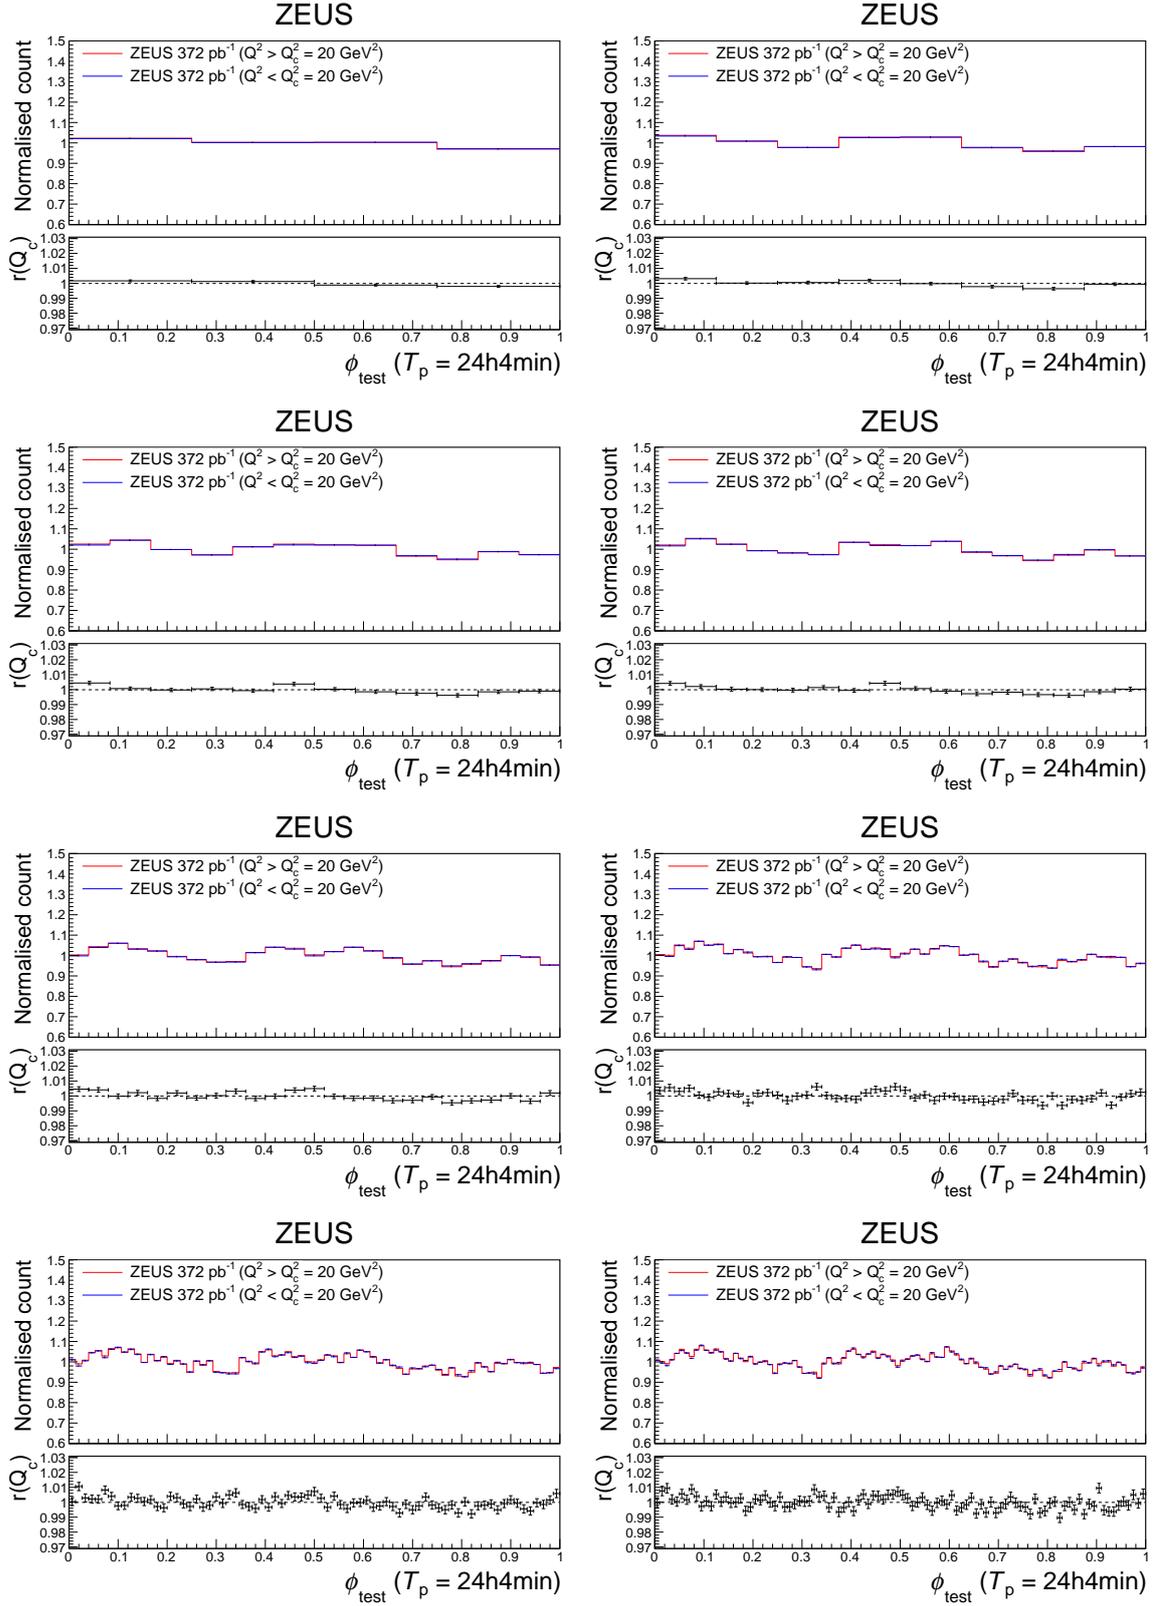

**Figure 8:**  $T_p = 24$  h 4 min phase dependence of the normalised counts in 4, 8, 12, 16, 25, 50, 75 and 100 bins with the kinematic region divided by  $Q_c^2 = 20$  GeV<sup>2</sup>. The vertical axis displays the number of events per bin normalised to the total number of events times the bin width. The ratios of the counts  $r(Q_c)$  above and below  $Q_c^2$  are given in the bottom panels. Only statistical uncertainties are displayed.

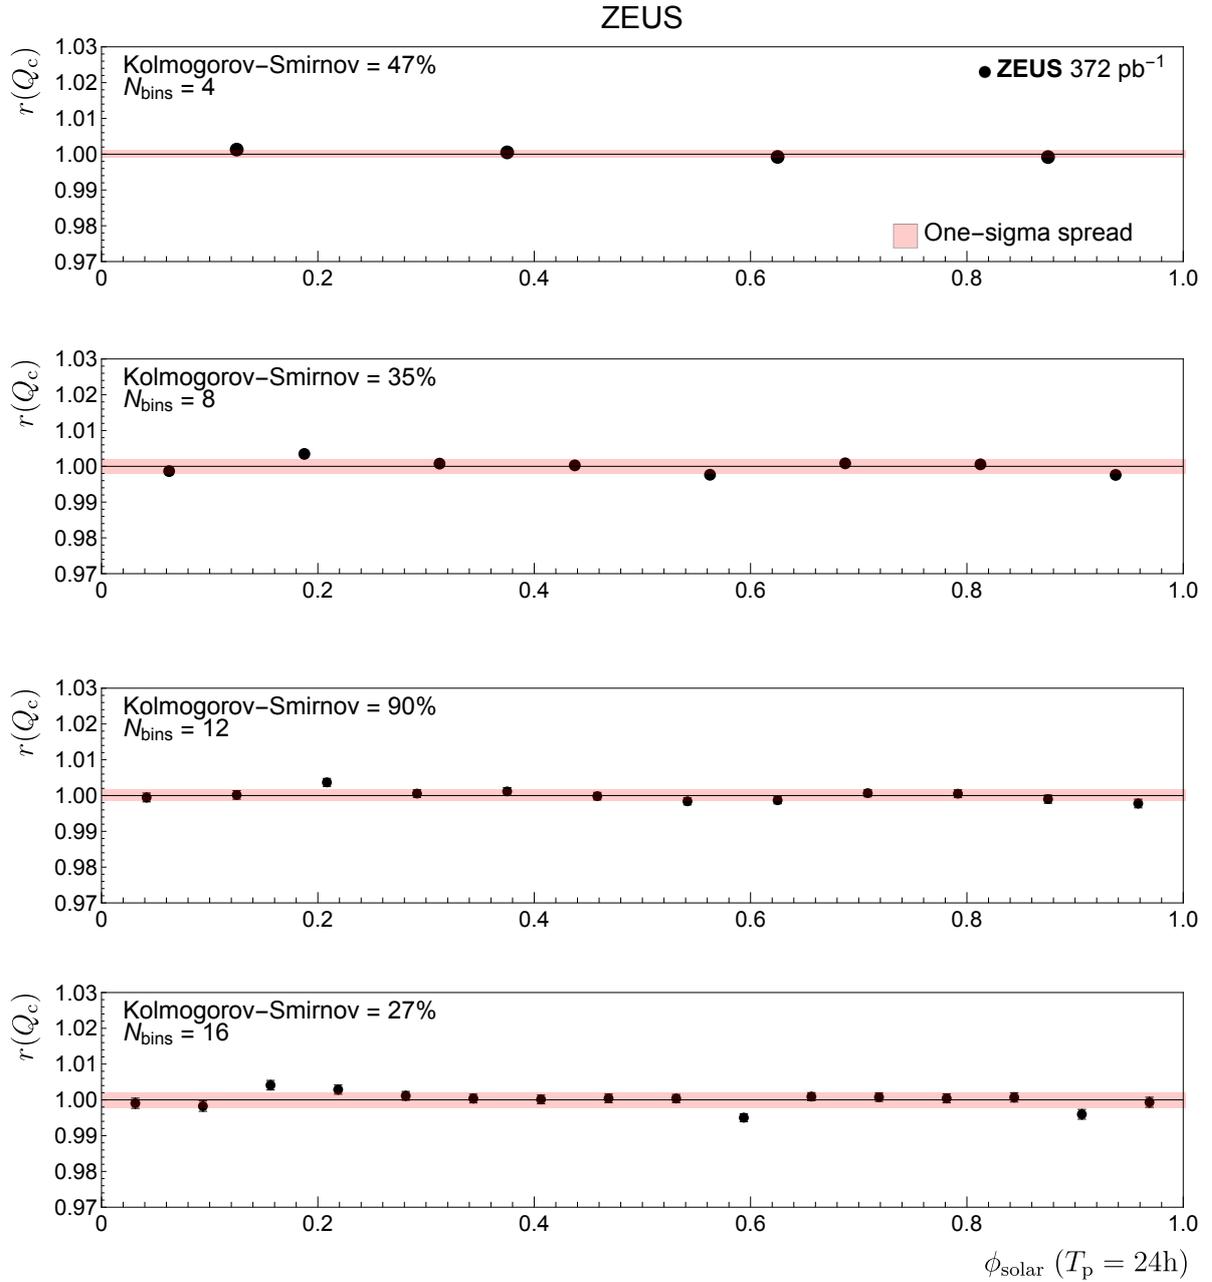

**Figure 9:** Ratio  $r(Q_c)$  of normalised counts for  $Q_c^2 = 20 \text{ GeV}^2$  binned with the solar phase where  $N_{\text{bins}} = 4, 8, 12$  and  $16$ . The displayed uncertainties include statistical uncertainties only and the one-sigma spreads (bands) are the standard deviations of the central values. The observed distributions are compared to a Gaussian distribution in which only statistical errors are included using a Kolmogorov-Smirnov test.

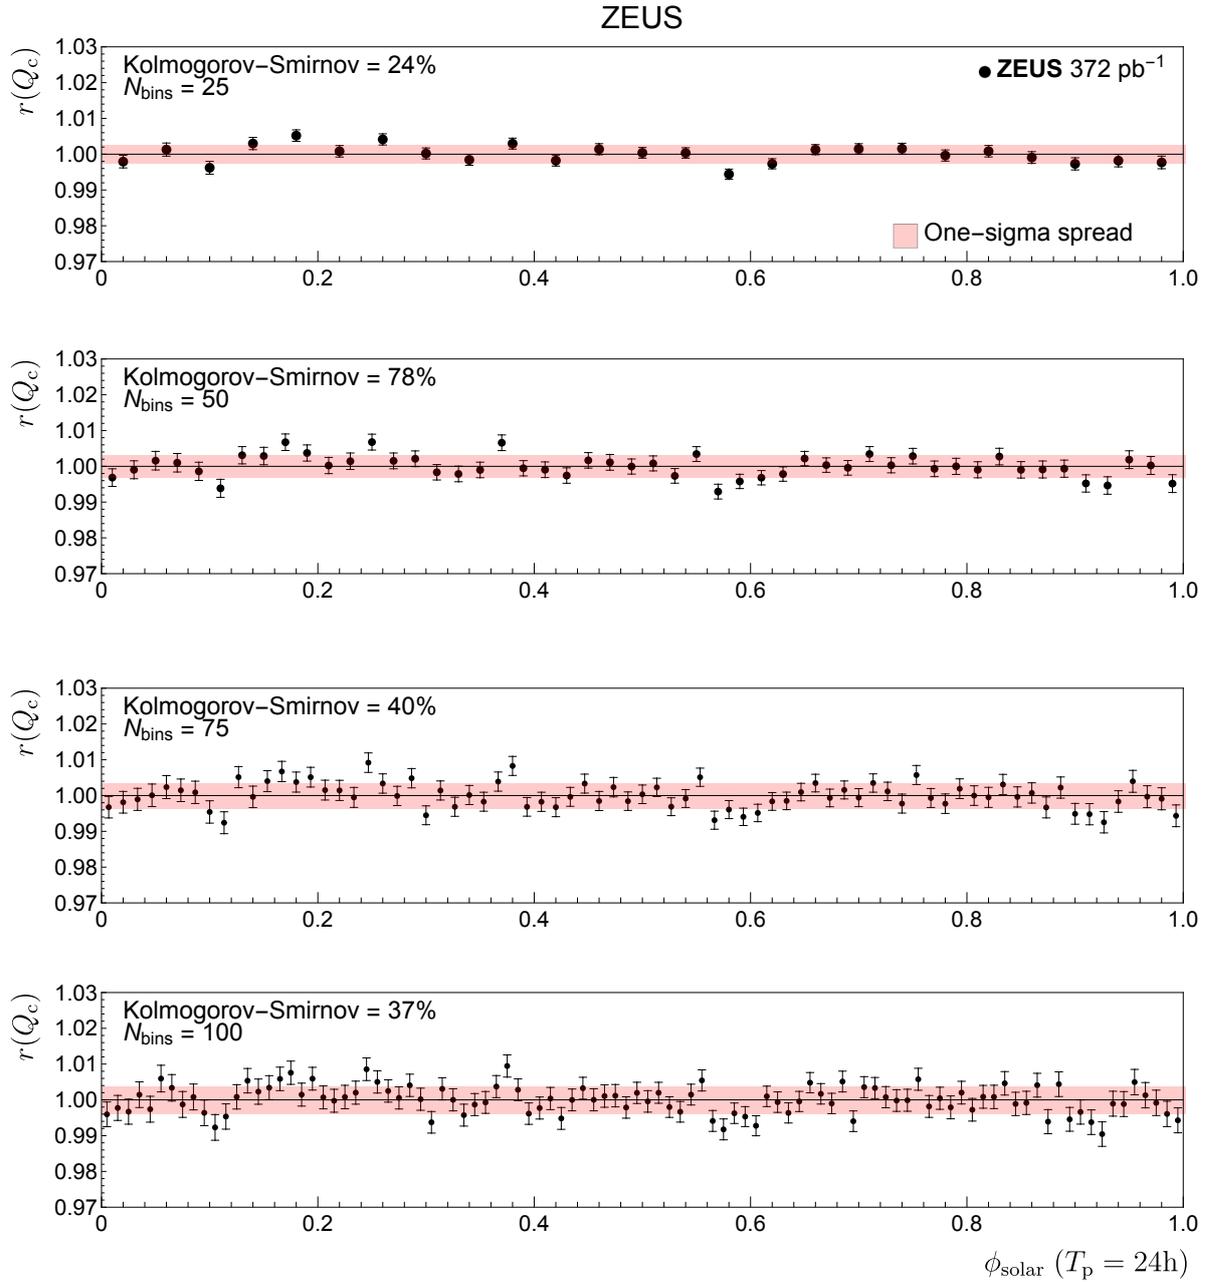

**Figure 10:** Ratio  $r(Q_c)$  of normalised counts for  $Q_c^2 = 20 \text{ GeV}^2$  binned with the solar phase where  $N_{\text{bins}} = 25, 50, 75$  and  $100$ . The displayed uncertainties include statistical uncertainties only and the one-sigma spreads (bands) are the standard deviations of the central values. The observed distributions are compared to a Gaussian distribution in which only statistical errors are included using a Kolmogorov-Smirnov test.

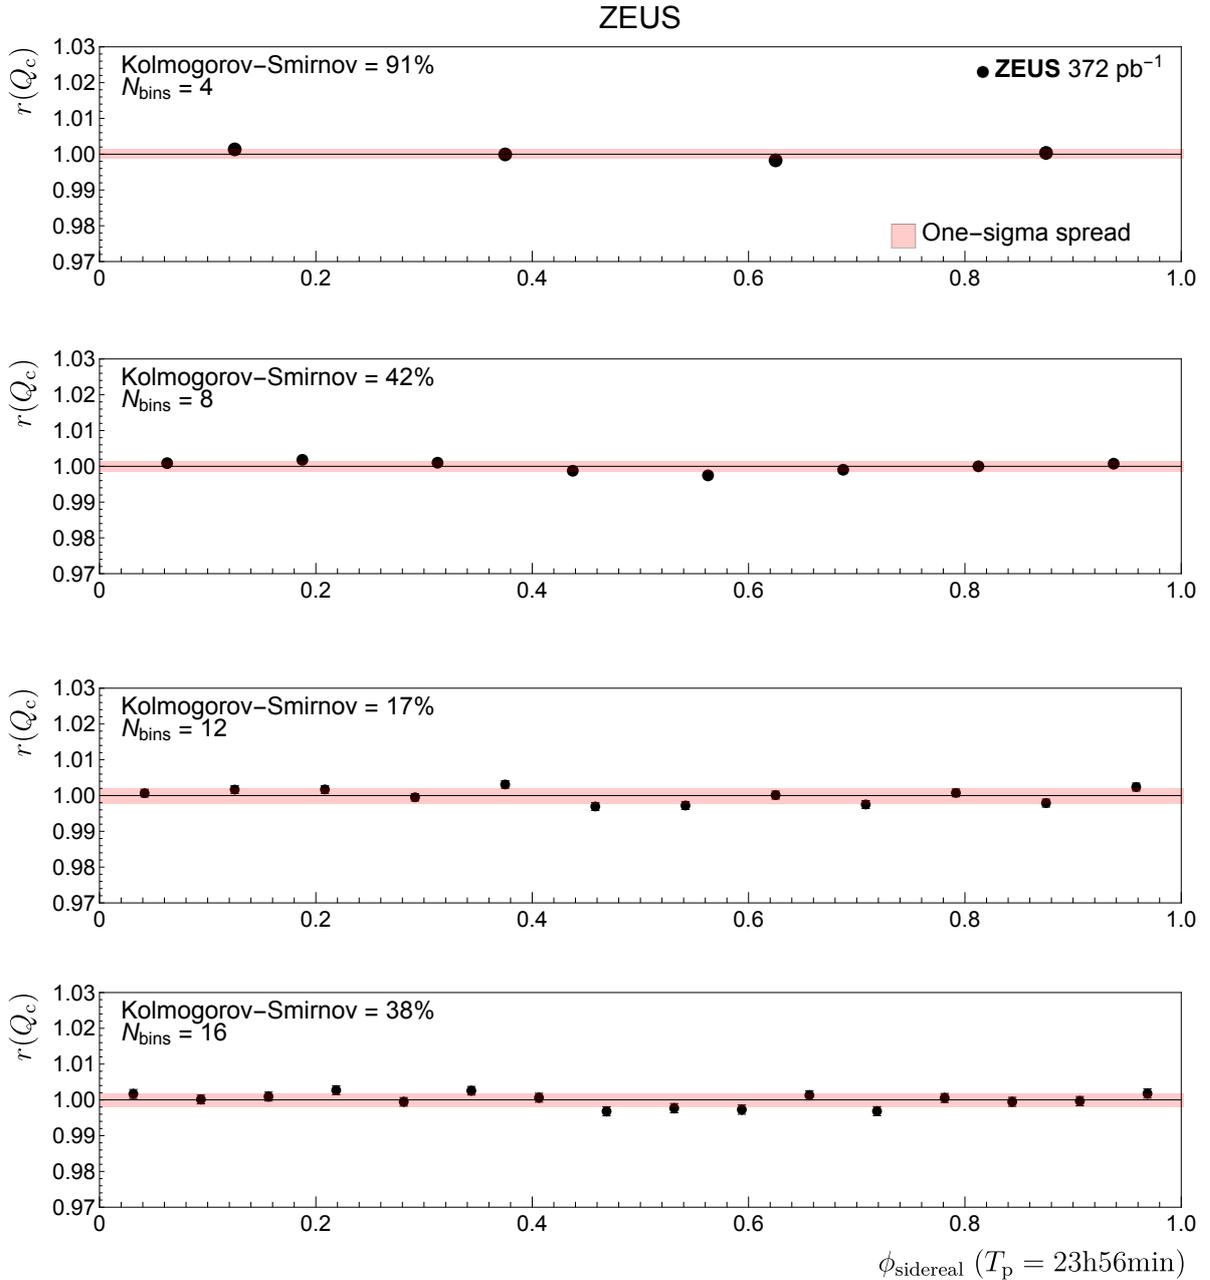

**Figure 11:** Ratio  $r(Q_c)$  of normalised counts for  $Q_c^2 = 20 \text{ GeV}^2$  binned with the sidereal phase where  $N_{\text{bins}} = 4, 8, 12$  and  $16$ . The displayed uncertainties include statistical uncertainties only and the one-sigma spreads (bands) are the standard deviations of the central values. The observed distributions are compared to a Gaussian distribution in which only statistical errors are included using a Kolmogorov-Smirnov test.

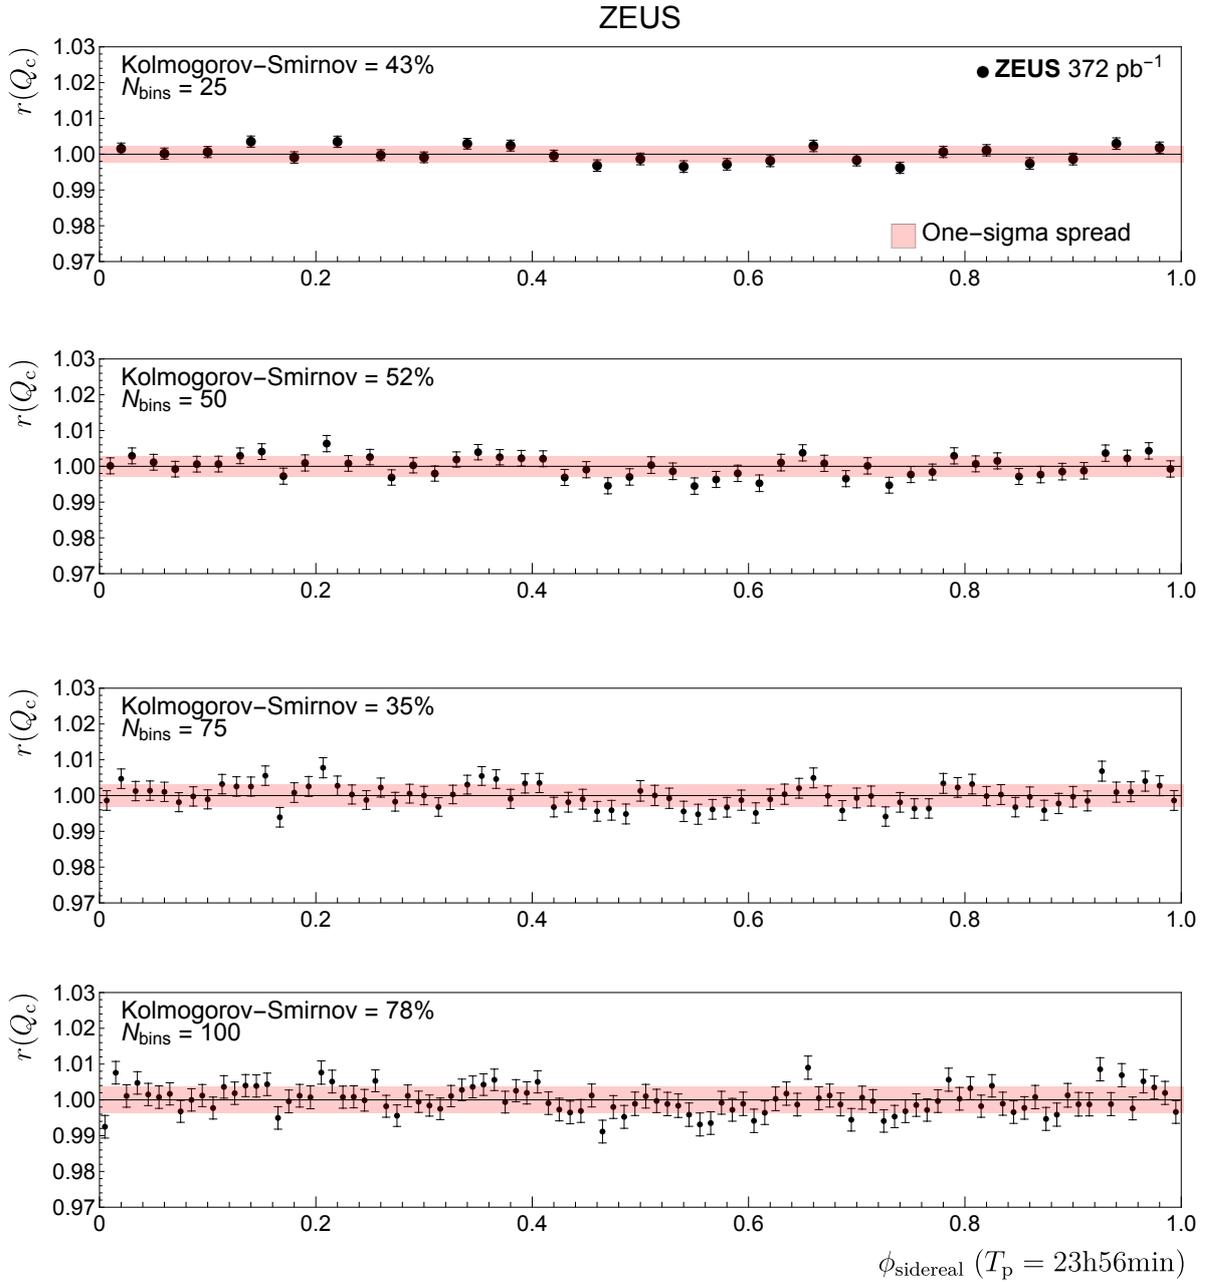

**Figure 12:** Ratio  $r(Q_c)$  of normalised counts for  $Q_c^2 = 20 \text{ GeV}^2$  binned with the sidereal phase where  $N_{\text{bins}} = 25, 50, 75$  and  $100$ . The displayed uncertainties include statistical uncertainties only and the one-sigma spreads (bands) are the standard deviations of the central values. The observed distributions are compared to a Gaussian distribution in which only statistical errors are included using a Kolmogorov–Smirnov test.

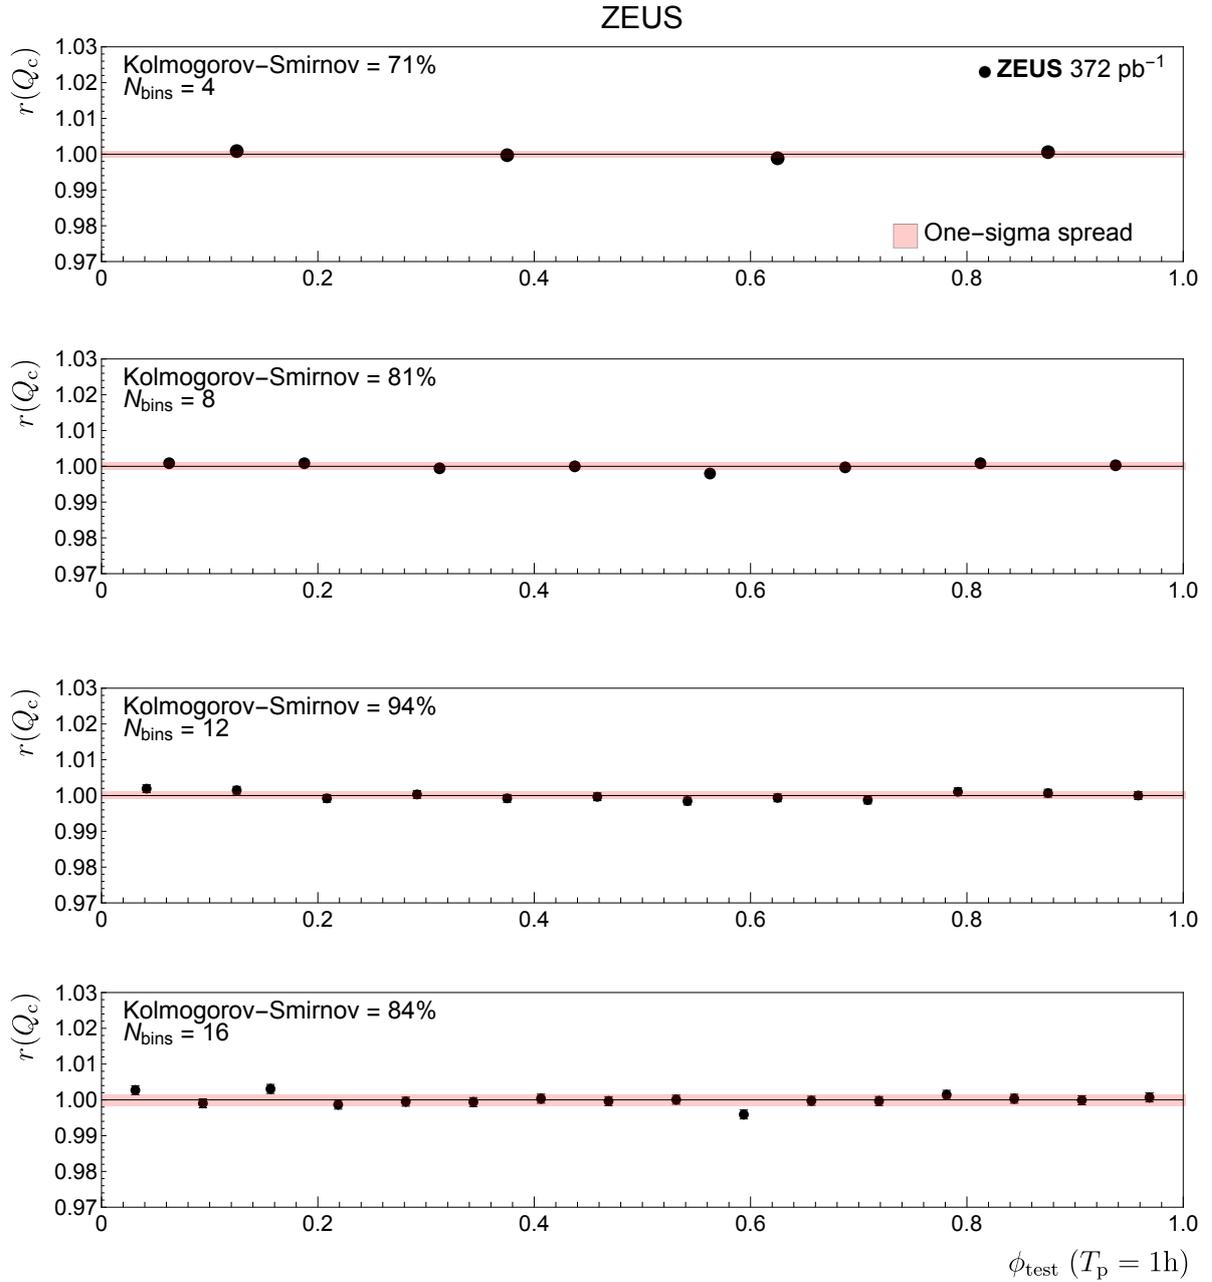

**Figure 13:** Ratio  $r(Q_c)$  of normalised counts for  $Q_c^2 = 20 \text{ GeV}^2$  binned with the test phase with  $T_p = 1 \text{ h}$  where  $N_{\text{bins}} = 4, 8, 12$  and  $16$ . The displayed uncertainties include statistical uncertainties only and the one-sigma spreads (bands) are the standard deviations of the central values. The observed distributions are compared to a Gaussian distribution in which only statistical errors are included using a Kolmogorov-Smirnov test.

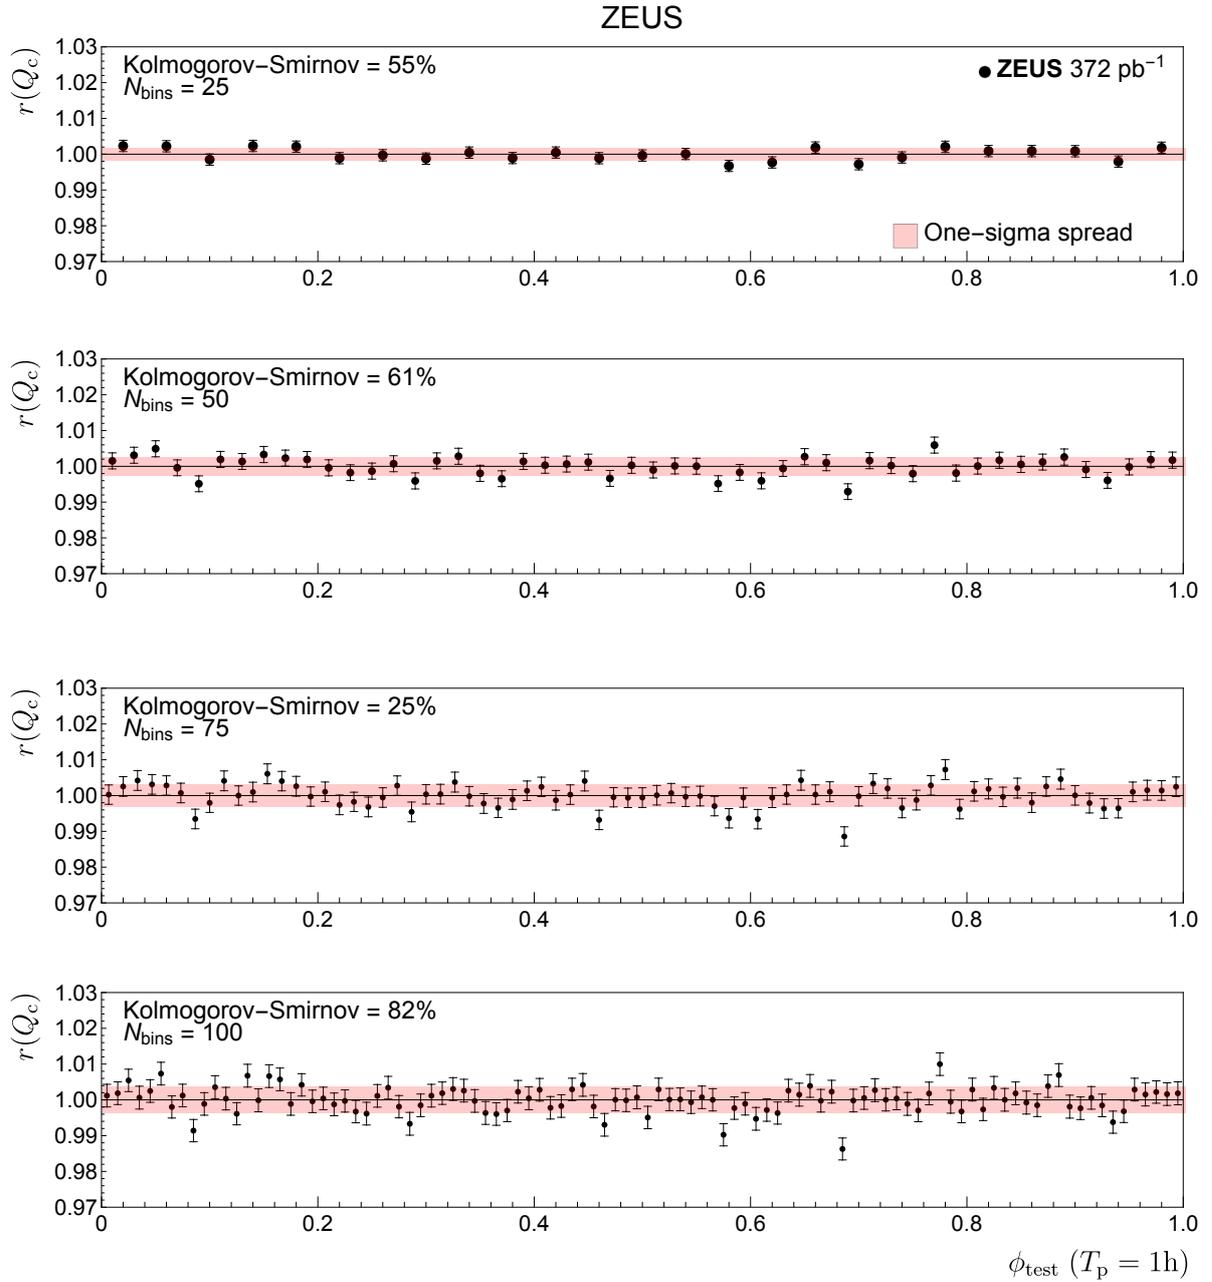

**Figure 14:** Ratio  $r(Q_c)$  of normalised counts for  $Q_c^2 = 20 \text{ GeV}^2$  binned with the test phase with  $T_p = 1 \text{ h}$  where  $N_{\text{bins}} = 25, 50, 75$  and  $100$ . The displayed uncertainties include statistical uncertainties only and the one-sigma spreads (bands) are the standard deviations of the central values. The observed distributions are compared to a Gaussian distribution in which only statistical errors are included using a Kolmogorov-Smirnov test.

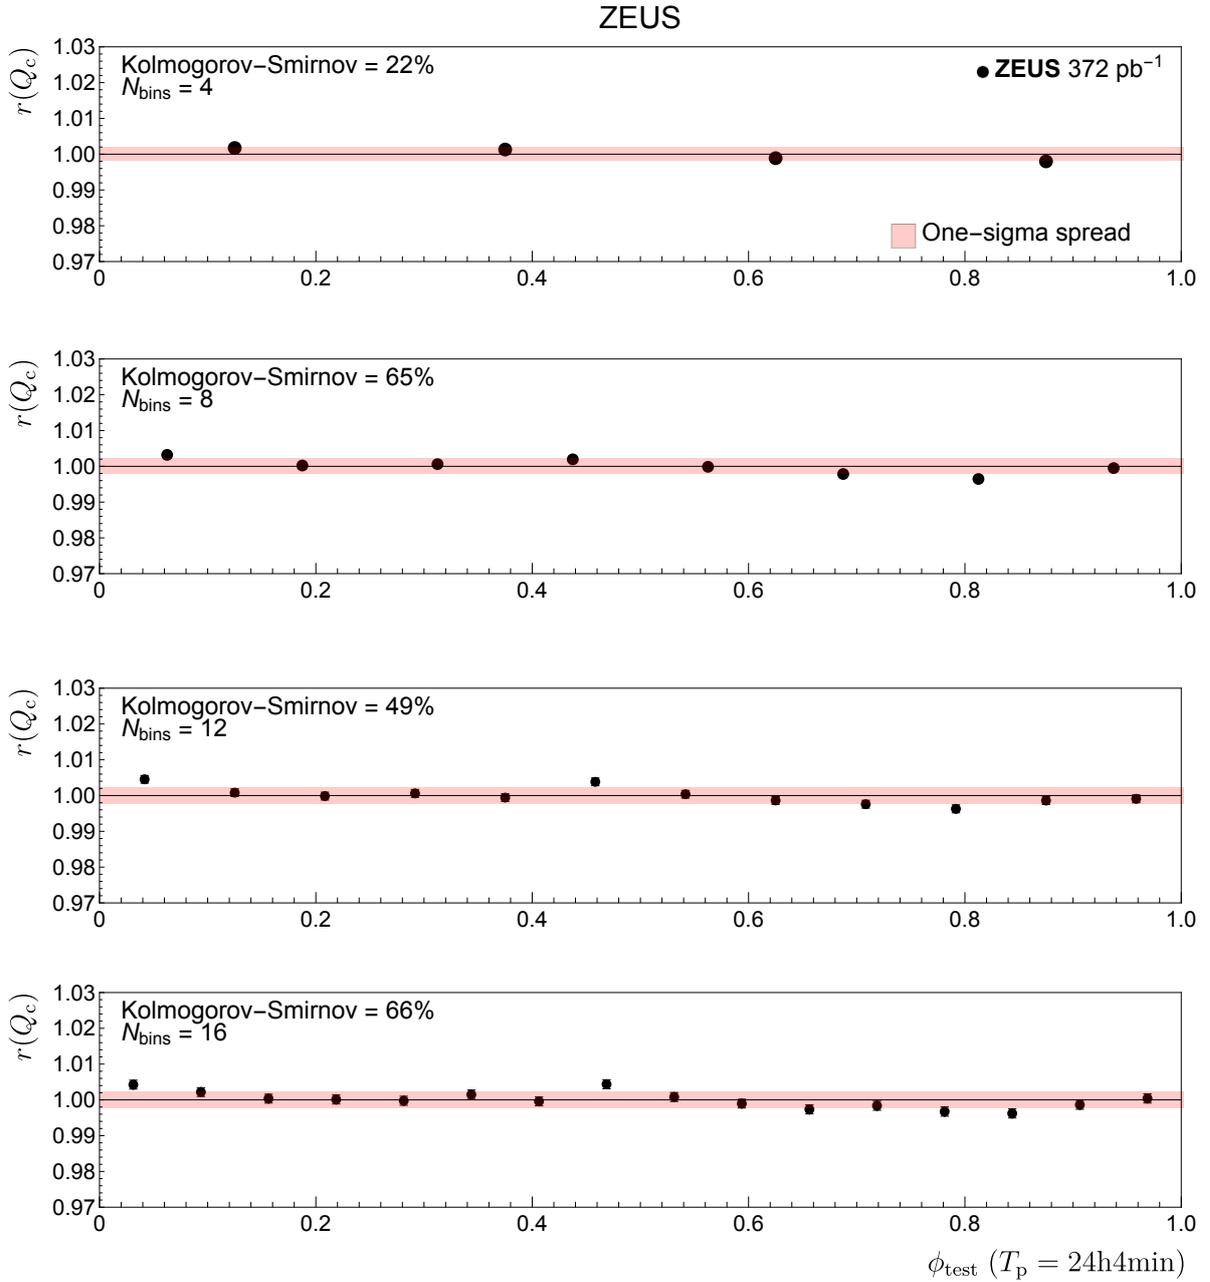

**Figure 15:** Ratio  $r(Q_c)$  of normalised counts for  $Q_c^2 = 20 \text{ GeV}^2$  binned with the test phase with  $T_p = 24 \text{ h } 4 \text{ min}$  where  $N_{\text{bins}} = 4, 8, 12$  and  $16$ . The displayed uncertainties include statistical uncertainties only and the one-sigma spreads (bands) are the standard deviations of the central values. The observed distributions are compared to a Gaussian distribution in which only statistical errors are included using a Kolmogorov-Smirnov test.

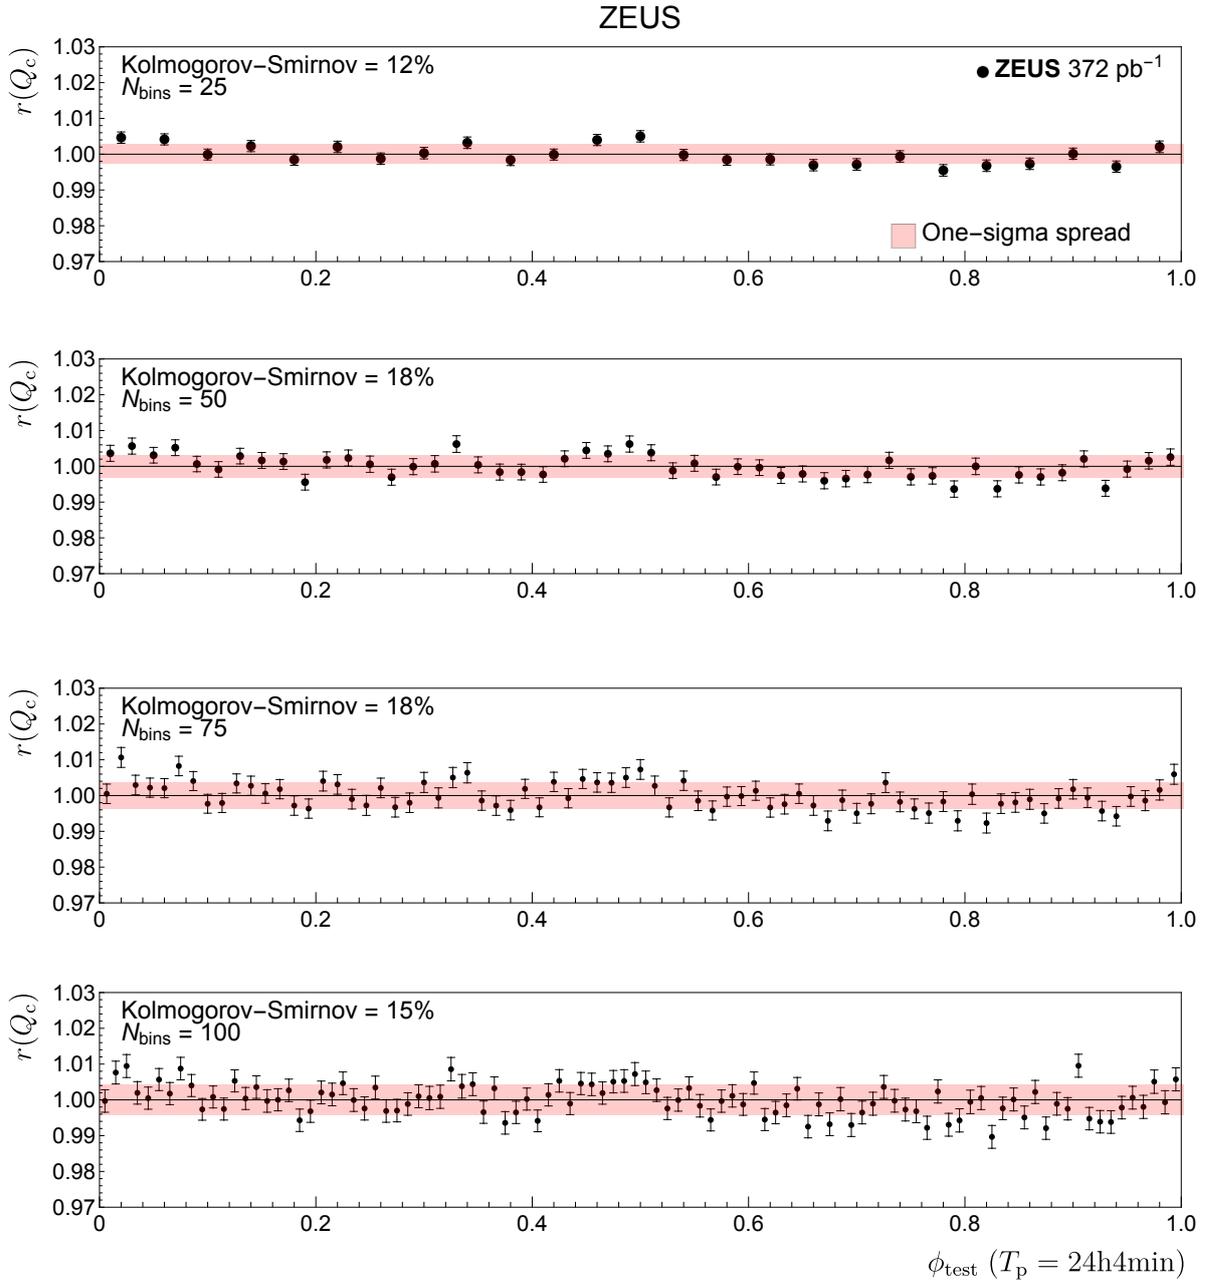

**Figure 16:** Ratio  $r(Q_c)$  of normalised counts for  $Q_c^2 = 20 \text{ GeV}^2$  binned with the test phase with  $T_p = 24 \text{ h } 4 \text{ min}$  where  $N_{\text{bins}} = 25, 50, 75$  and  $100$ . The displayed uncertainties include statistical uncertainties only and the one-sigma spreads (bands) are the standard deviations of the central values. The observed distributions are compared to a Gaussian distribution in which only statistical errors are included using a Kolmogorov-Smirnov test.

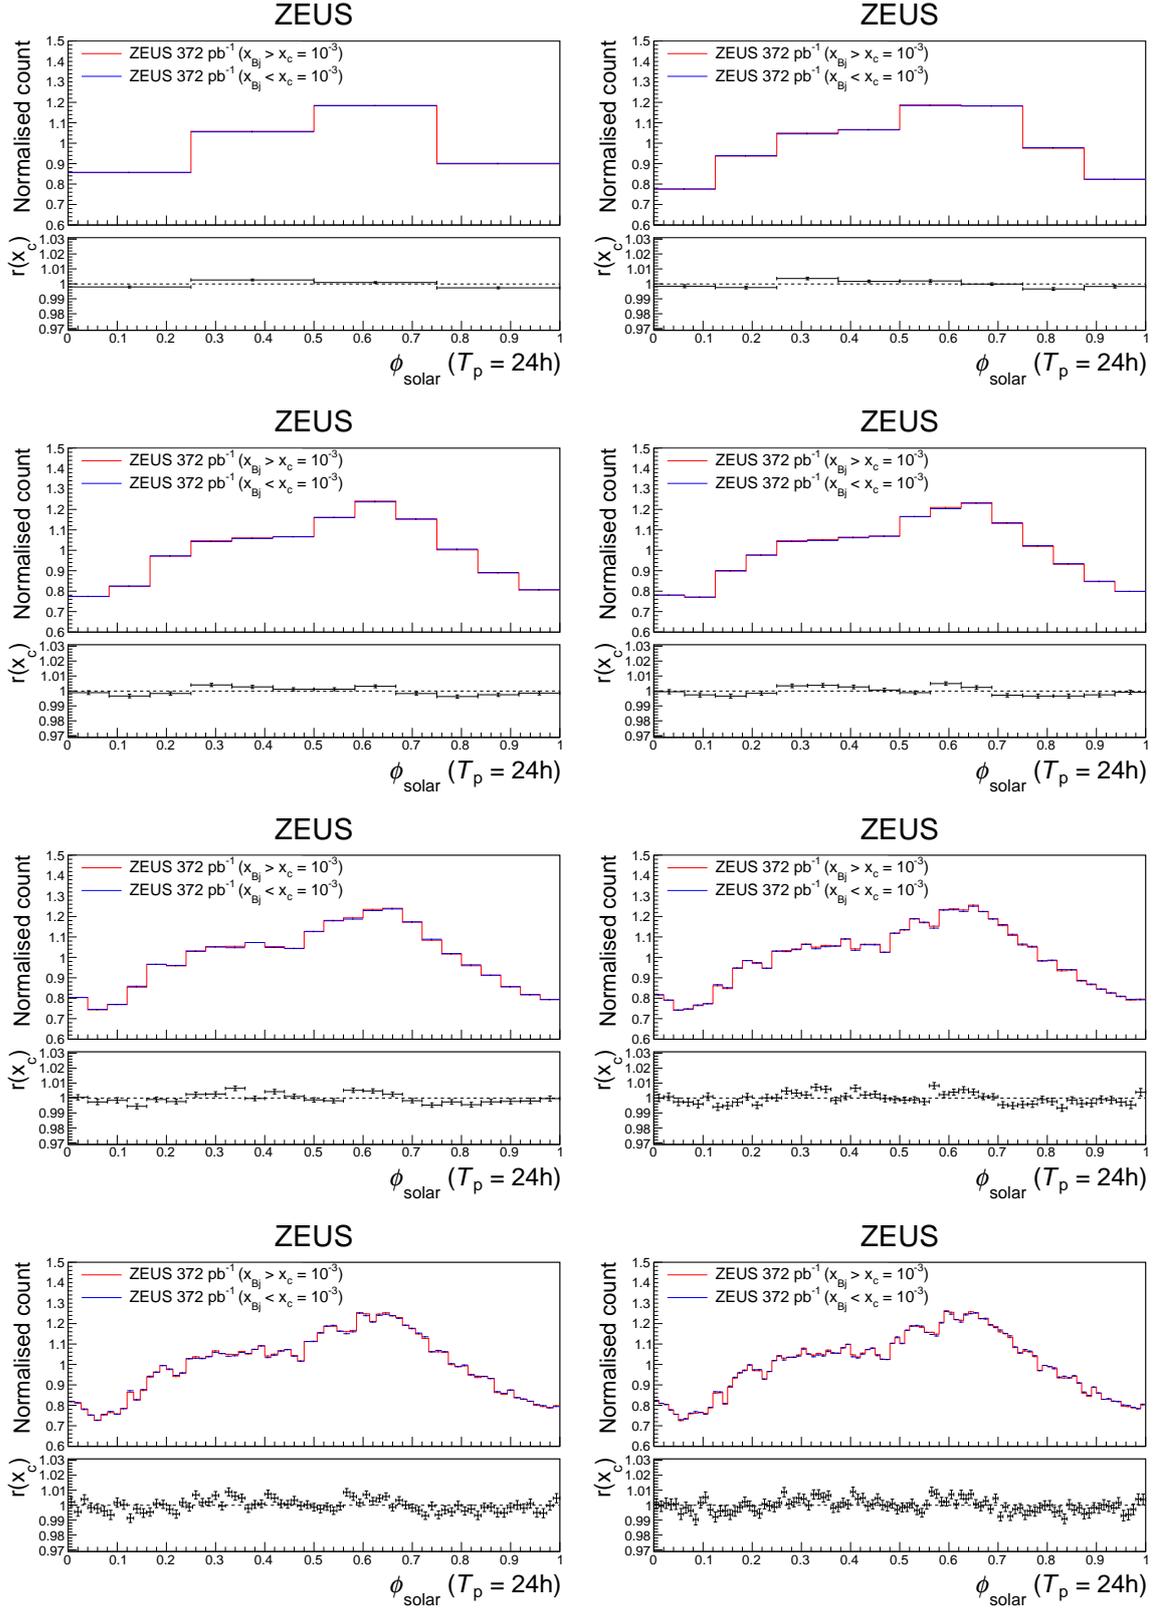

**Figure 17:** Solar phase dependence of the normalised counts in 4, 8, 12, 16, 25, 50, 75 and 100 bins with the kinematic region divided by  $x_c = 10^{-3}$ . The vertical axis displays the number of events per bin normalised to the total number of events times the bin width. The ratios of the counts  $r(x_c)$  above and below  $x_c$  are given in the bottom panels. For the solar phase,  $\phi_{\text{solar}} = 0$  is identified with 11:20 UTC. Only statistical uncertainties are displayed.

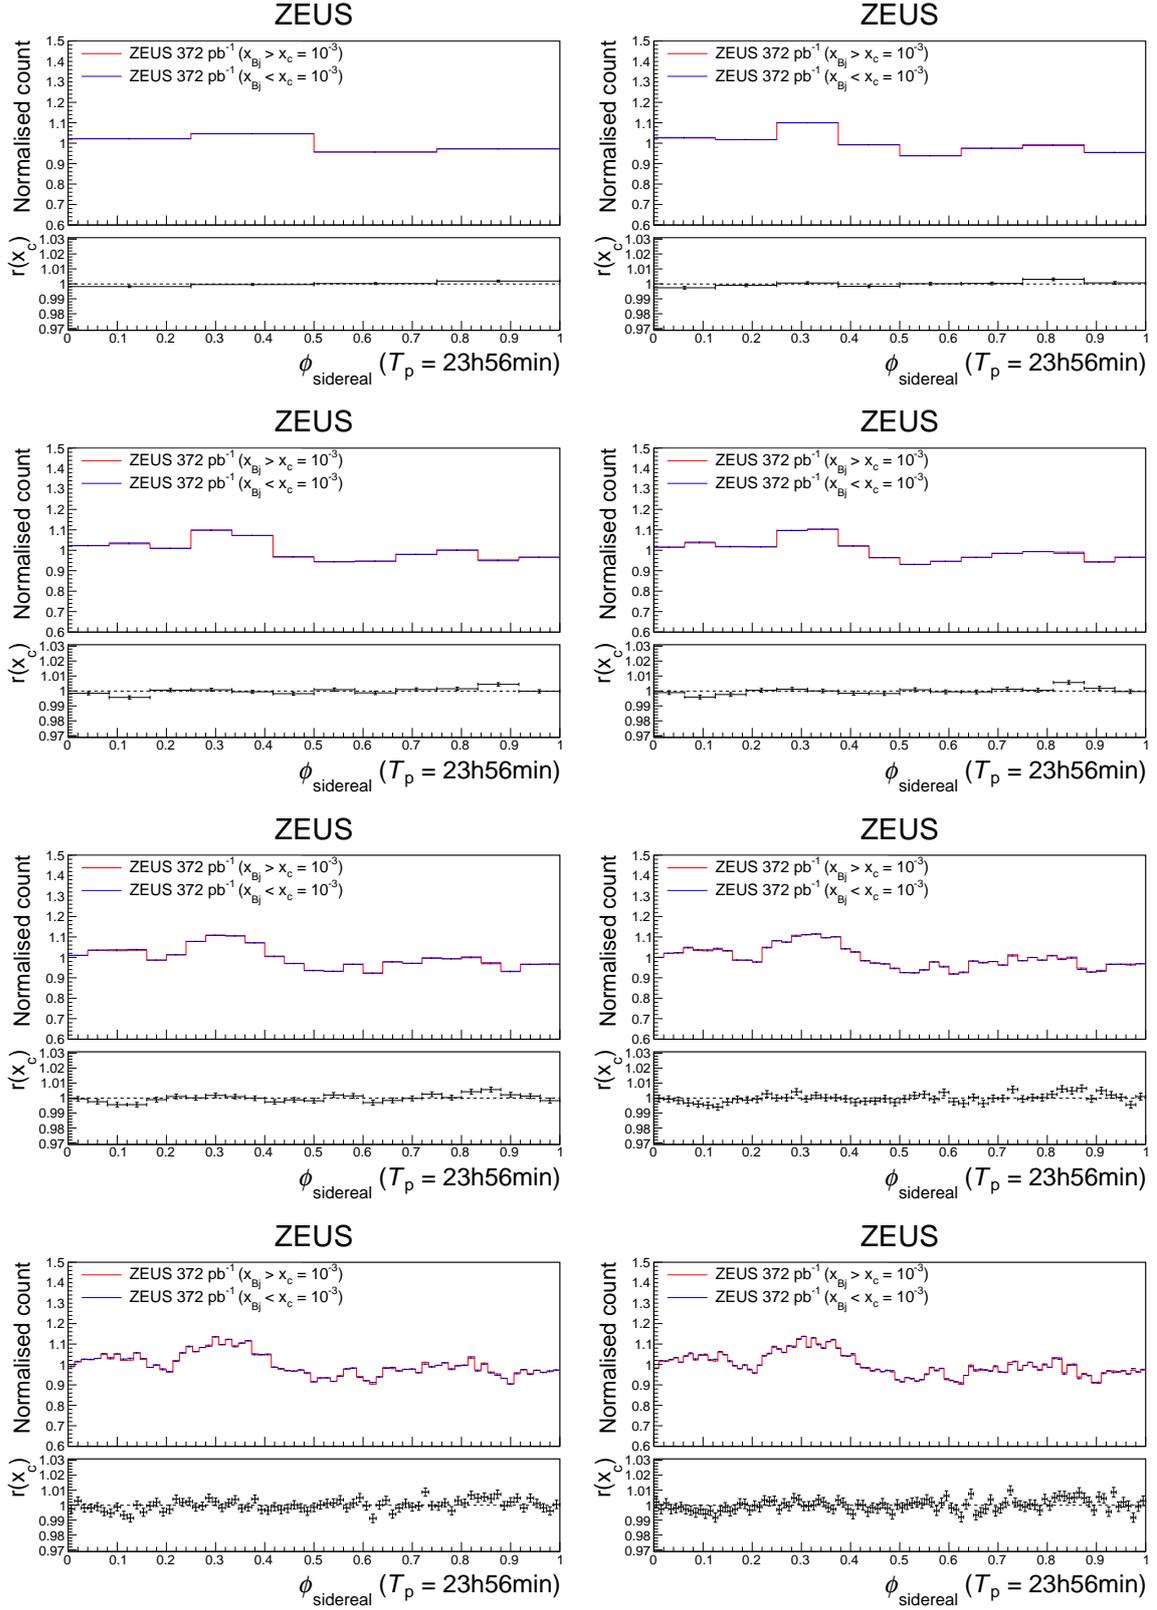

**Figure 18:** Sidereal phase dependence of the normalised counts in 4, 8, 12, 16, 25, 50, 75 and 100 bins with the kinematic region divided by  $x_c = 10^{-3}$ . The vertical axis displays the number of events per bin normalised to the total number of events times the bin width. The ratios of the counts  $r(x_c)$  above and below  $x_c$  are given in the bottom panels. Only statistical uncertainties are displayed.

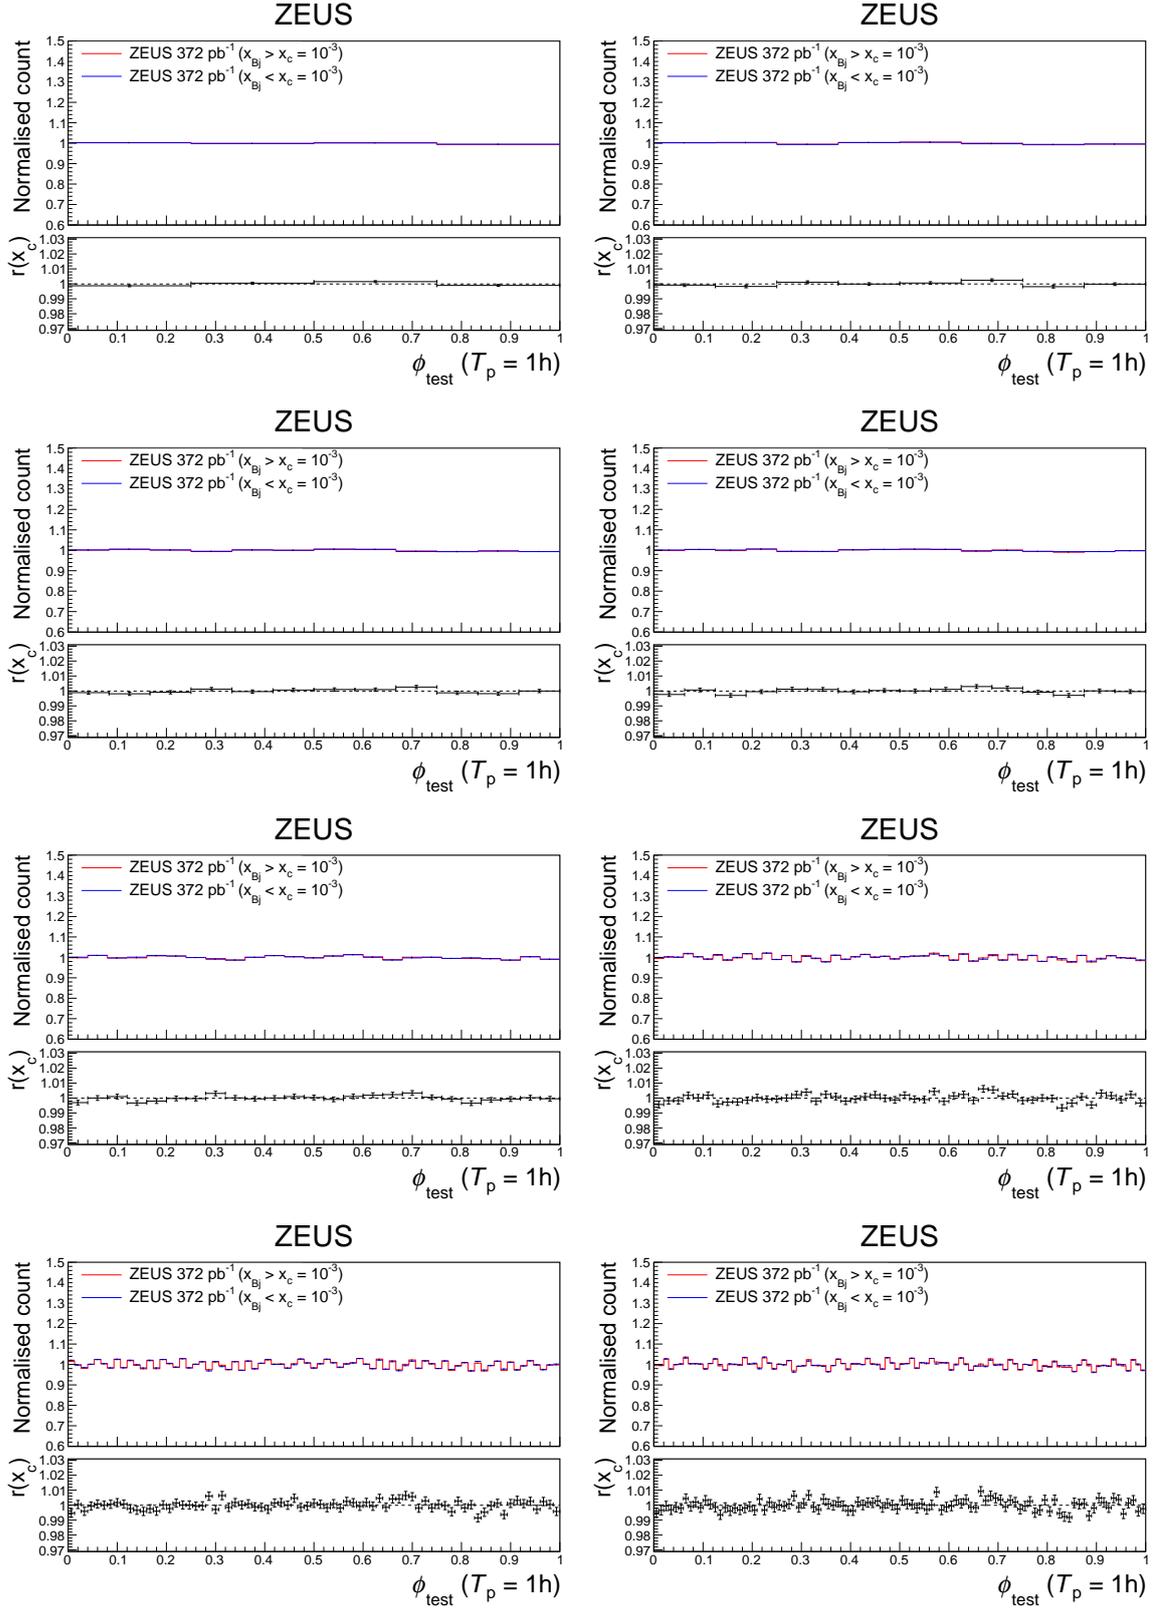

**Figure 19:**  $T_p = 1$  h phase dependence of the normalised counts in 4, 8, 12, 16, 25, 50, 75 and 100 bins with the kinematic region divided by  $x_c = 10^{-3}$ . The vertical axis displays the number of events per bin normalised to the total number of events times the bin width. The ratios of the counts  $r(x_c)$  above and below  $x_c$  are given in the bottom panels. Only statistical uncertainties are displayed.

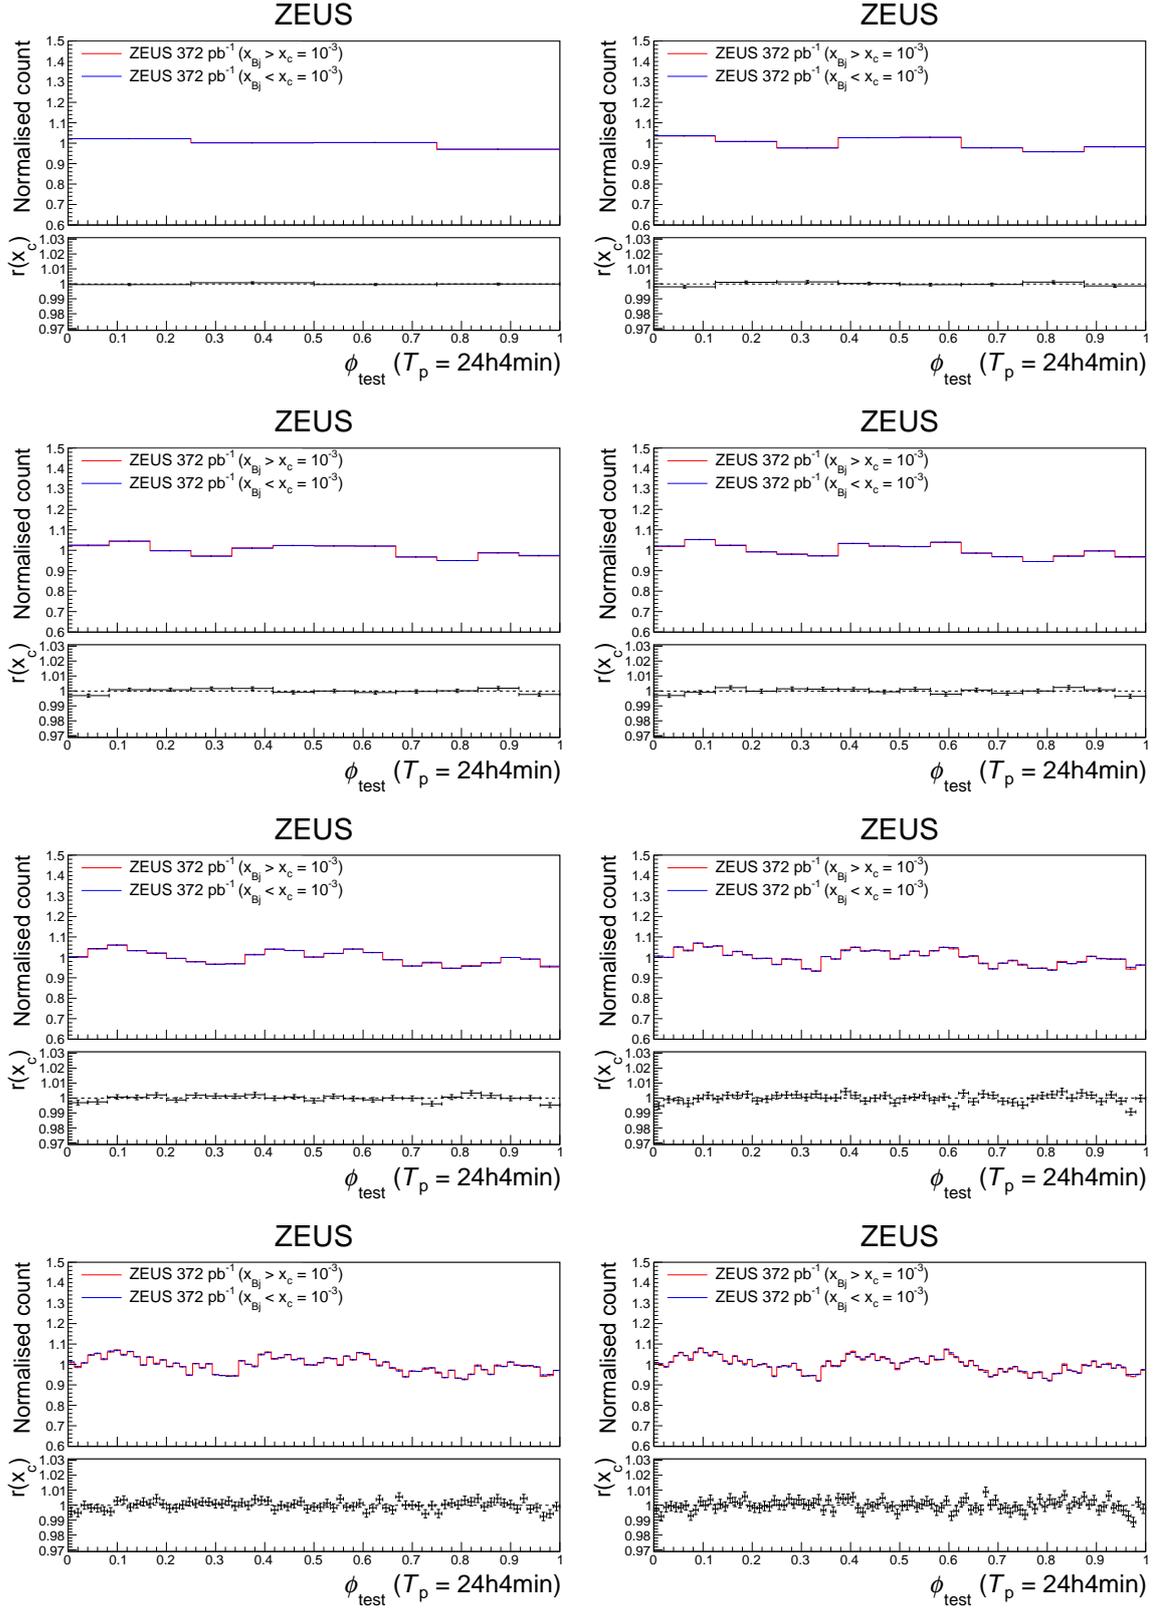

**Figure 20:**  $T_p = 24$  h 4 min phase dependence of the normalised counts in 4, 8, 12, 16, 25, 50, 75 and 100 bins with the kinematic region divided by  $x_c = 10^{-3}$ . The vertical axis displays the number of events per bin normalised to the total number of events times the bin width. The ratios of the counts  $r(x_c)$  above and below  $x_c$  are given in the bottom panels. Only statistical uncertainties are displayed.

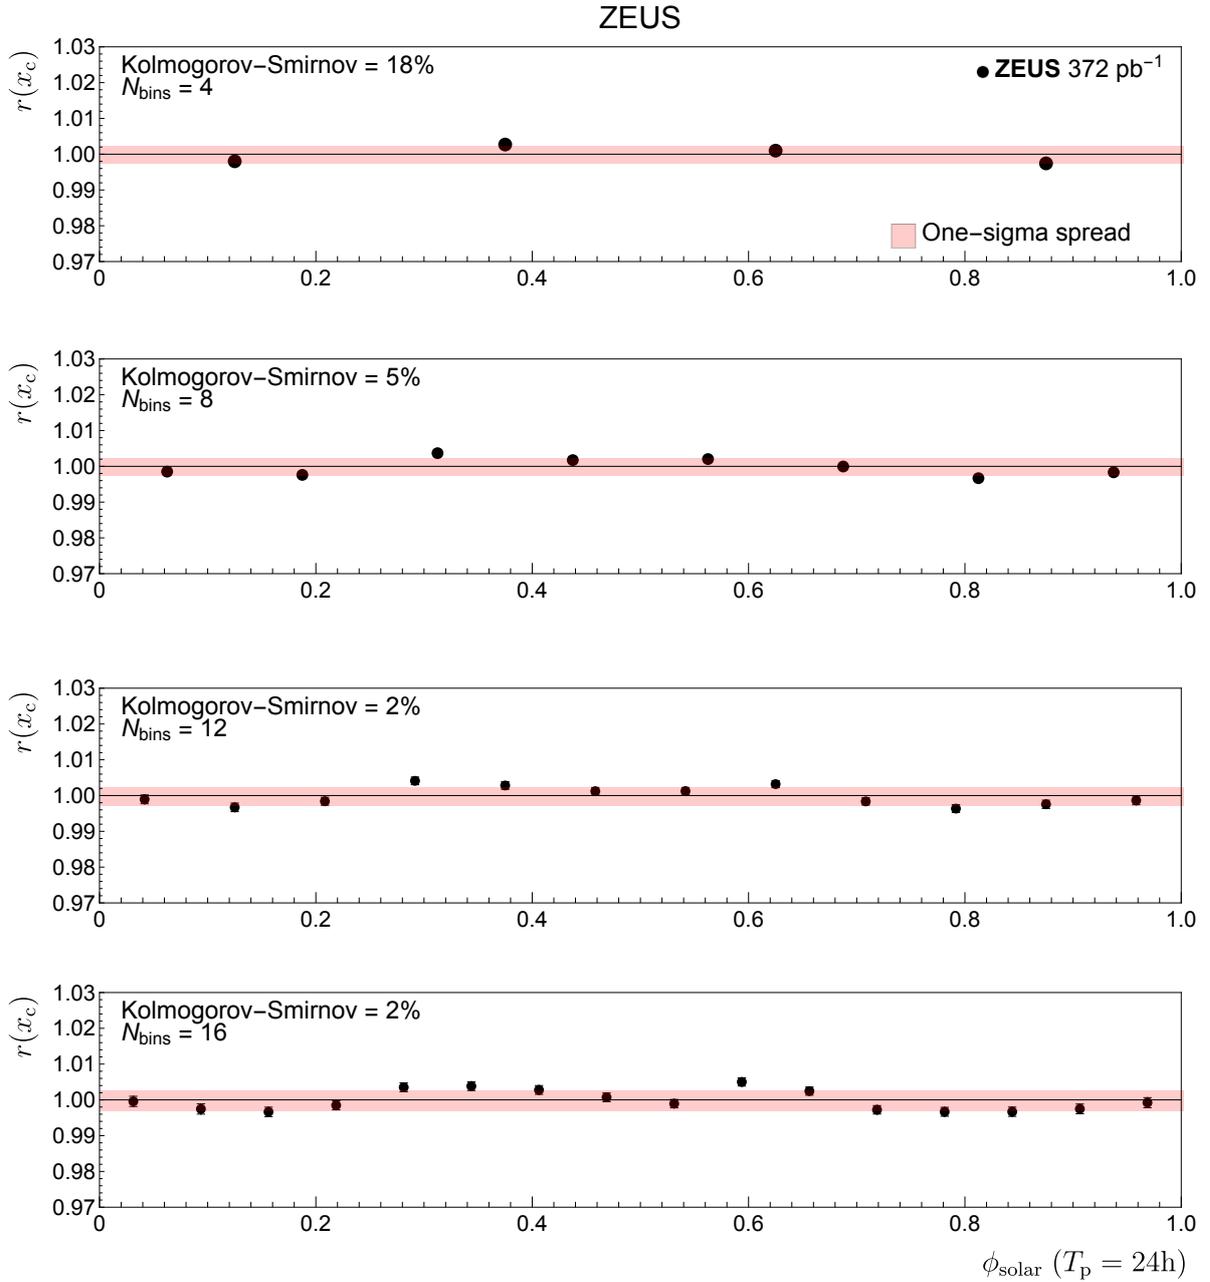

**Figure 21:** Ratio  $r(x_c)$  of normalised counts for  $x_c = 10^{-3}$  binned with the solar phase where  $N_{\text{bins}} = 4, 8, 12$  and  $16$ . The displayed uncertainties include statistical uncertainties only and the one-sigma spreads (bands) are the standard deviations of the central values. The observed distributions are compared to a Gaussian distribution in which only statistical errors are included using a Kolmogorov–Smirnov test.

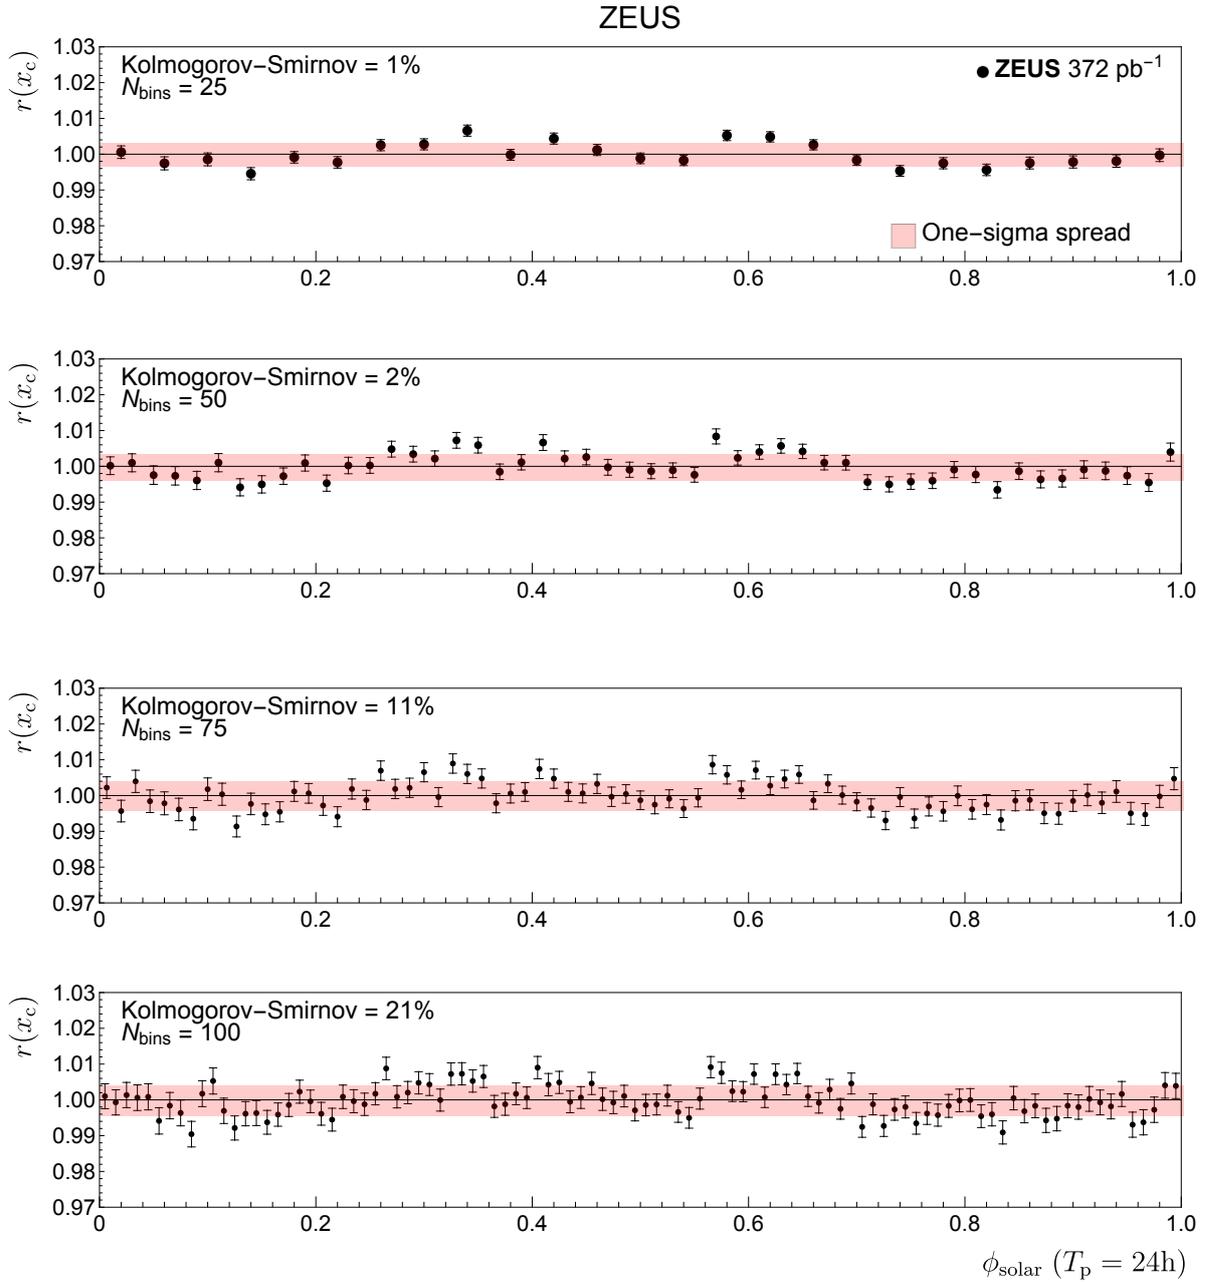

**Figure 22:** Ratio  $r(x_c)$  of normalised counts for  $x_c = 10^{-3}$  binned with the solar phase where  $N_{\text{bins}} = 25, 50, 75$  and  $100$ . The displayed uncertainties include statistical uncertainties only and the one-sigma spreads (bands) are the standard deviations of the central values. The observed distributions are compared to a Gaussian distribution in which only statistical errors are included using a Kolmogorov-Smirnov test.

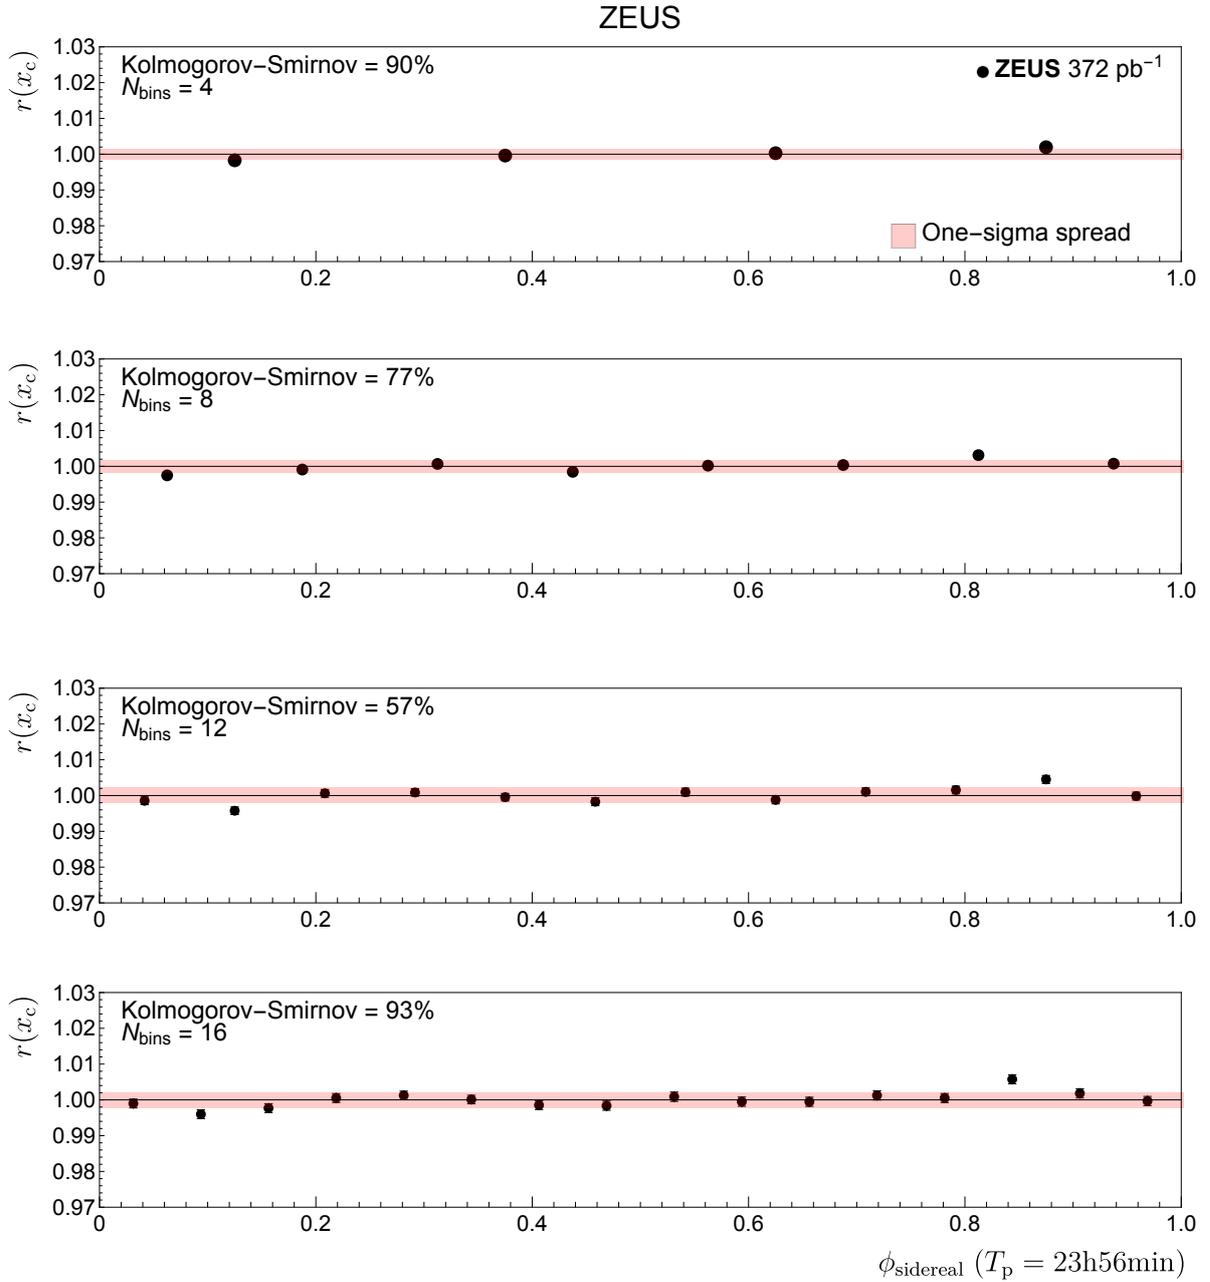

**Figure 23:** Ratio  $r(x_c)$  of normalised counts for  $x_c = 10^{-3}$  binned with the sidereal phase where  $N_{\text{bins}} = 4, 8, 12$  and  $16$ . The displayed uncertainties include statistical uncertainties only and the one-sigma spreads (bands) are the standard deviations of the central values. The observed distributions are compared to a Gaussian distribution in which only statistical errors are included using a Kolmogorov-Smirnov test.

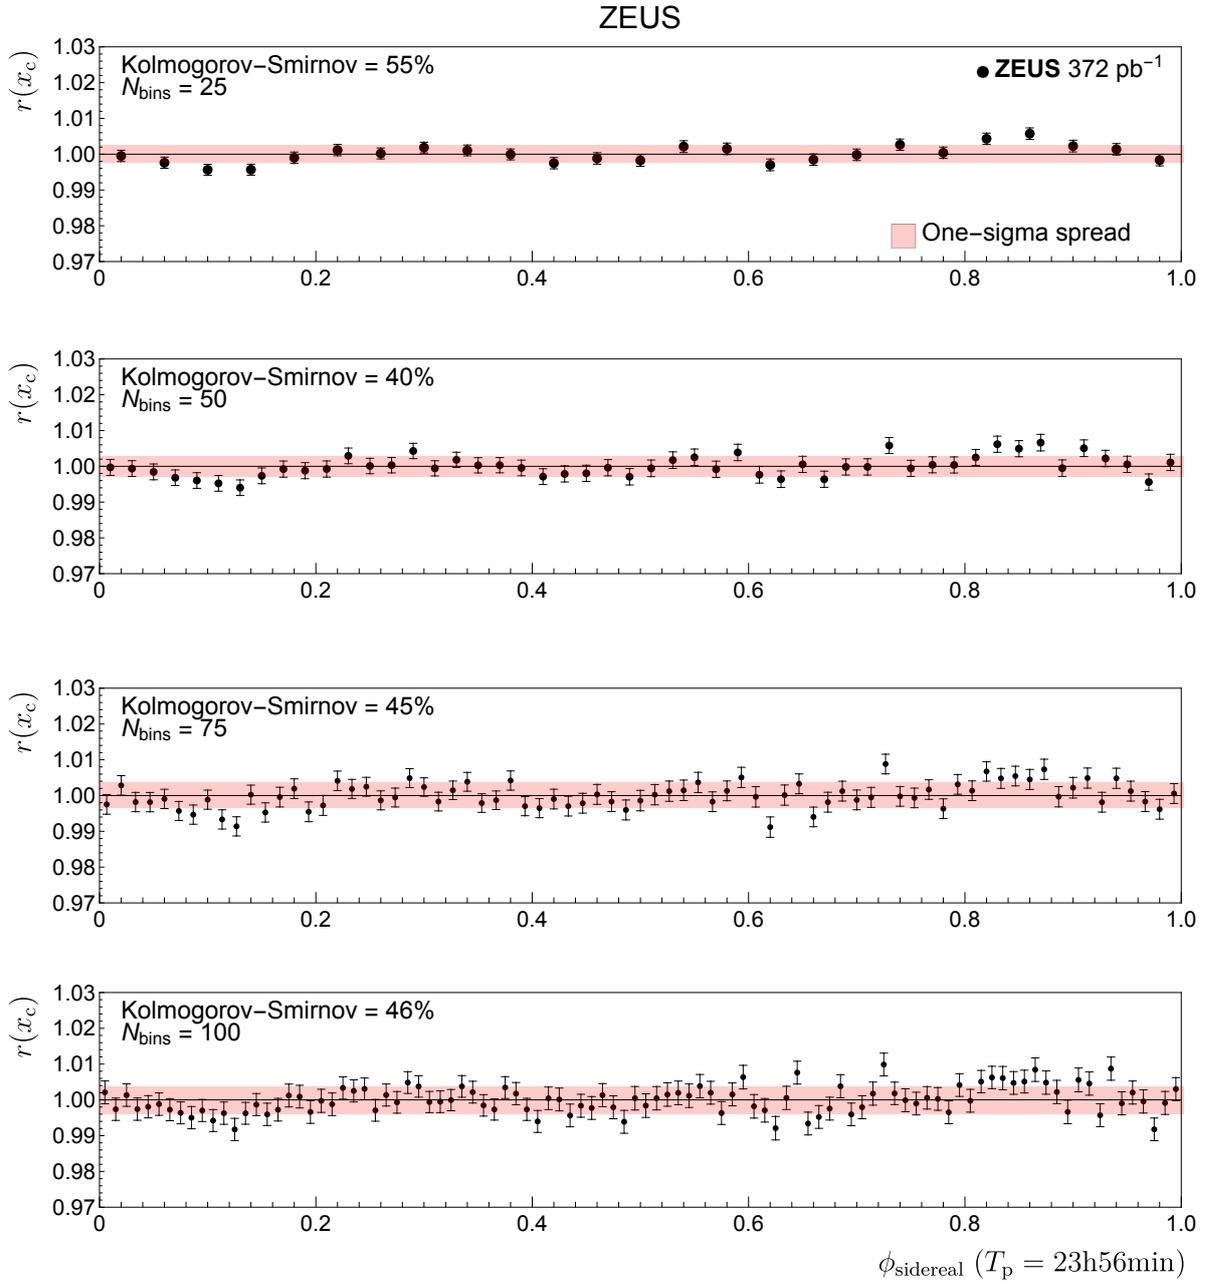

**Figure 24:** Ratio  $r(x_c)$  of normalised counts for  $x_c = 10^{-3}$  binned with the sidereal phase where  $N_{\text{bins}} = 25, 50, 75$  and  $100$ . The displayed uncertainties include statistical uncertainties only and the one-sigma spreads (bands) are the standard deviations of the central values. The observed distributions are compared to a Gaussian distribution in which only statistical errors are included using a Kolmogorov-Smirnov test.

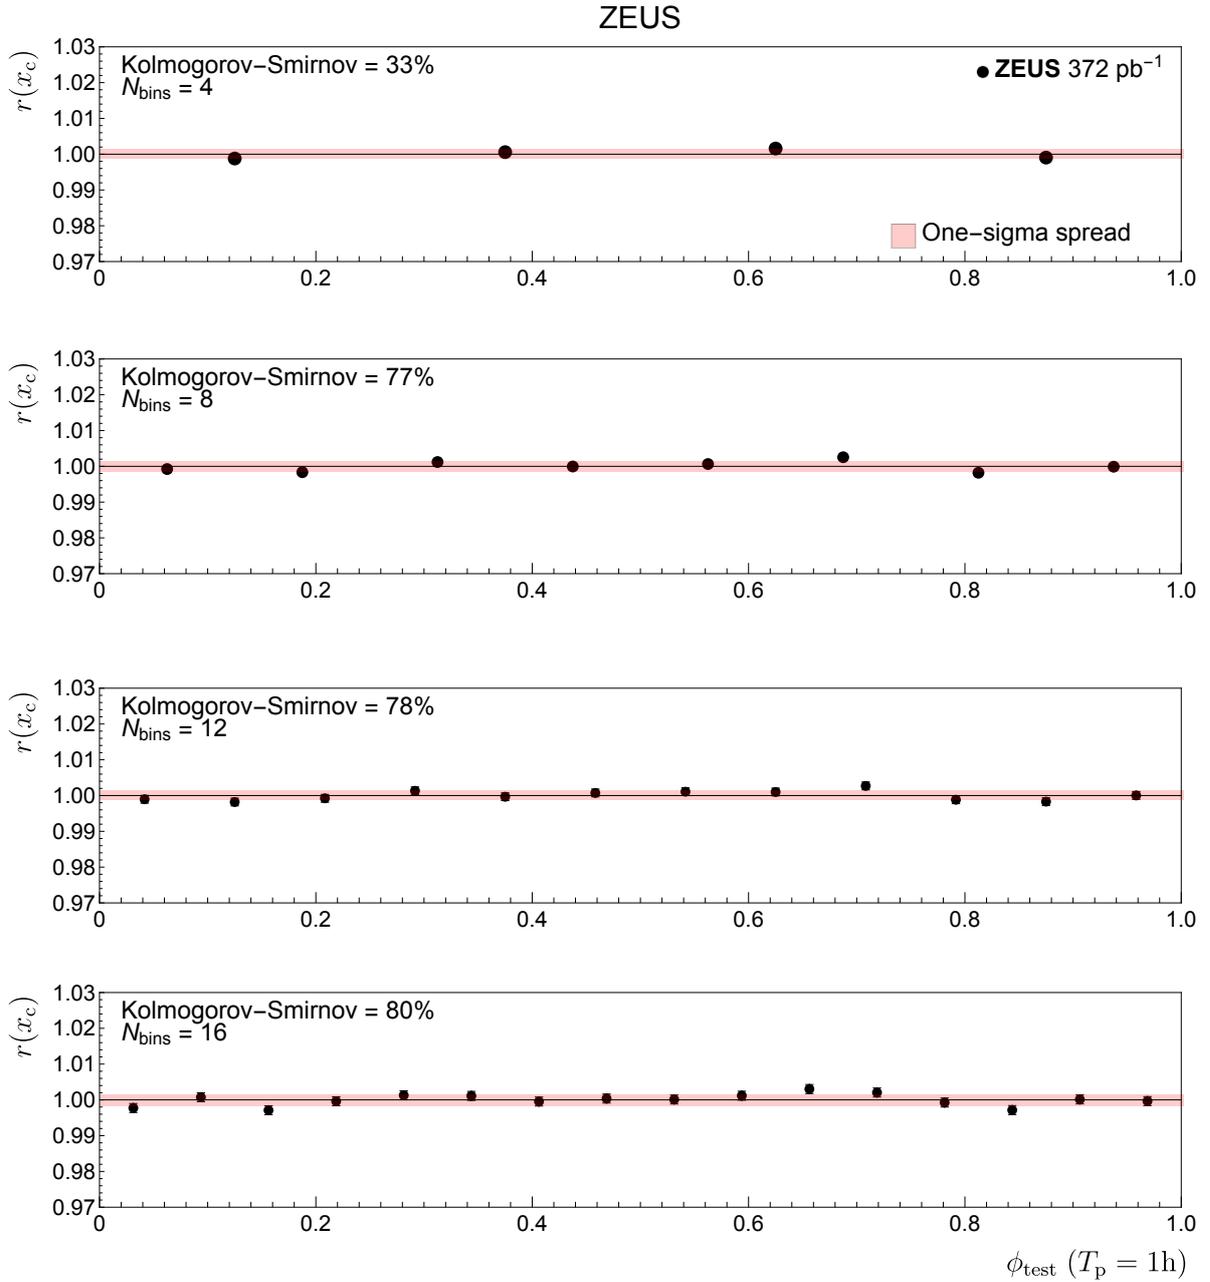

**Figure 25:** Ratio  $r(x_c)$  of normalised counts for  $x_c = 10^{-3}$  binned with the test phase with  $T_p = 1$  h where  $N_{\text{bins}} = 4, 8, 12$  and  $16$ . The displayed uncertainties include statistical uncertainties only and the one-sigma spreads (bands) are the standard deviations of the central values. The observed distributions are compared to a Gaussian distribution in which only statistical errors are included using a Kolmogorov-Smirnov test.

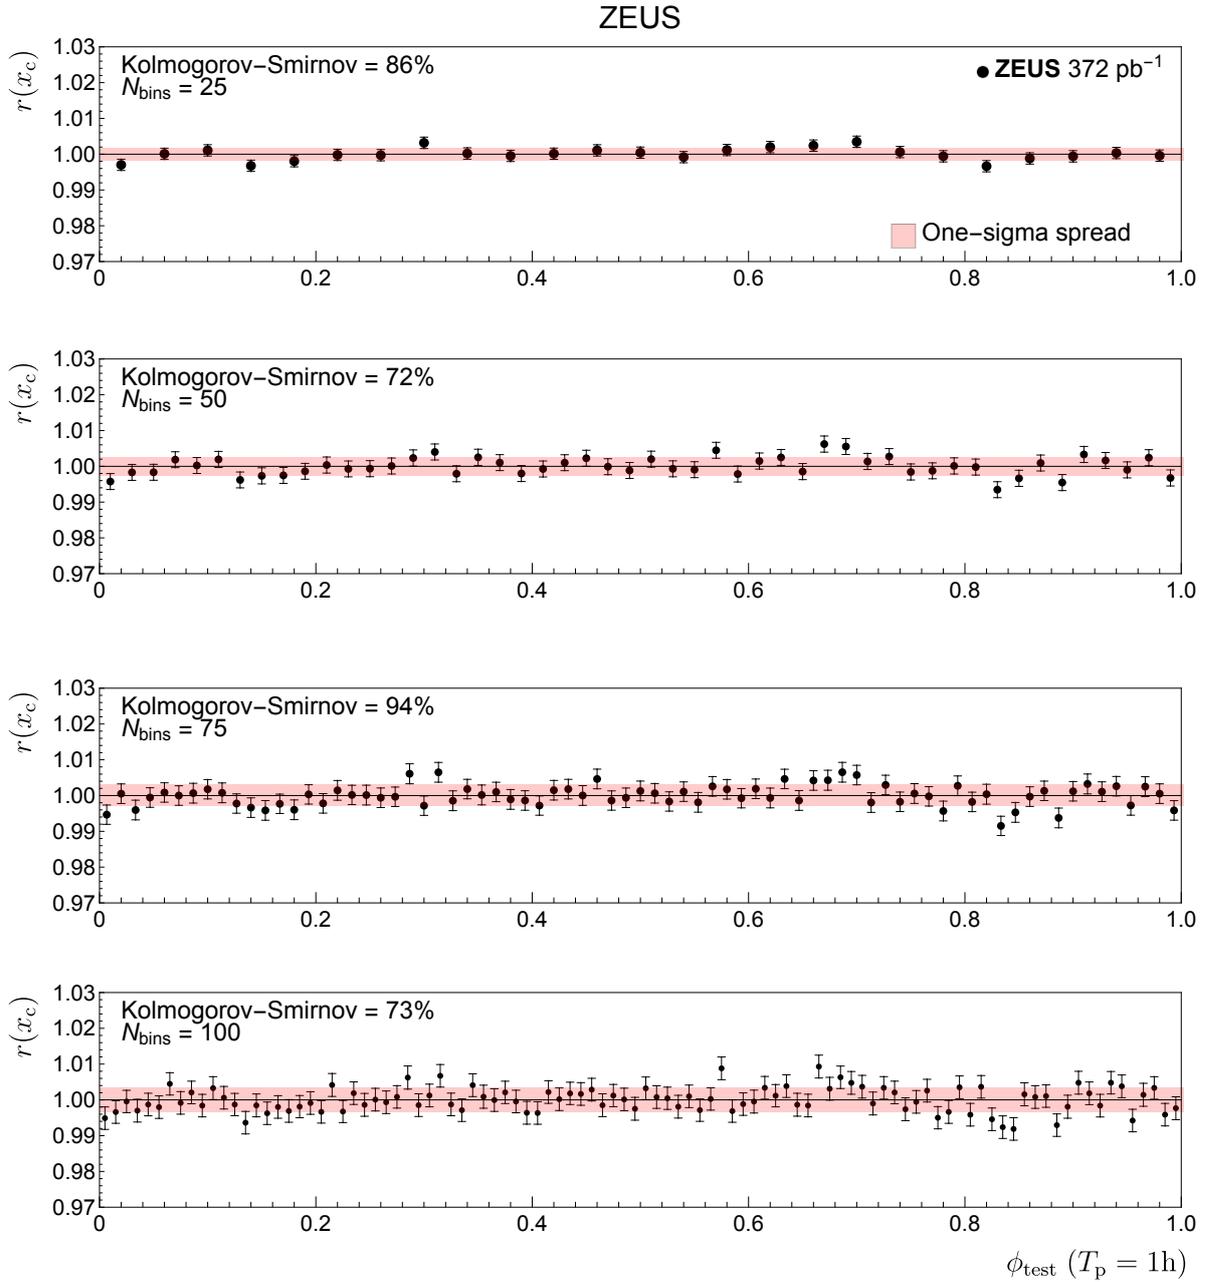

**Figure 26:** Ratio  $r(x_c)$  of normalised counts for  $x_c = 10^{-3}$  binned with the test phase with  $T_p = 1$  h where  $N_{\text{bins}} = 25, 50, 75$  and  $100$ . The displayed uncertainties include statistical uncertainties only and the one-sigma spreads (bands) are the standard deviations of the central values. The observed distributions are compared to a Gaussian distribution in which only statistical errors are included using a Kolmogorov-Smirnov test.

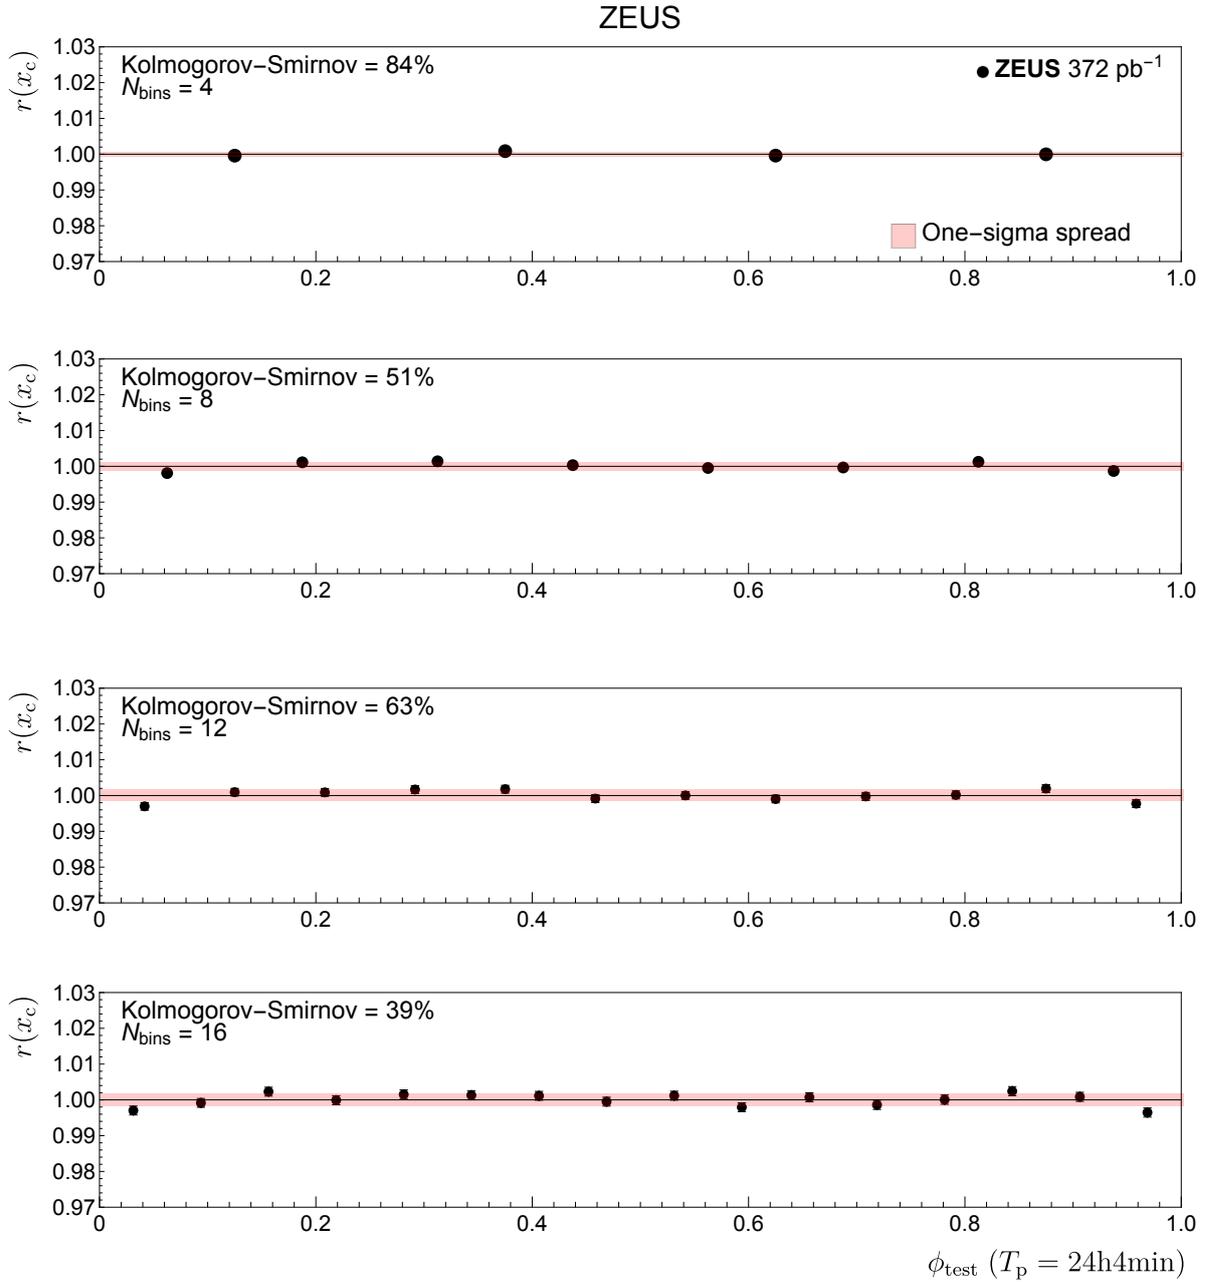

**Figure 27:** Ratio  $r(x_c)$  of normalised counts for  $x_c = 10^{-3}$  binned with the test phase with  $T_p = 24$  h 4 min where  $N_{\text{bins}} = 4, 8, 12$  and  $16$ . The displayed uncertainties include statistical uncertainties only and the one-sigma spreads (bands) are the standard deviations of the central values. The observed distributions are compared to a Gaussian distribution in which only statistical errors are included using a Kolmogorov-Smirnov test.

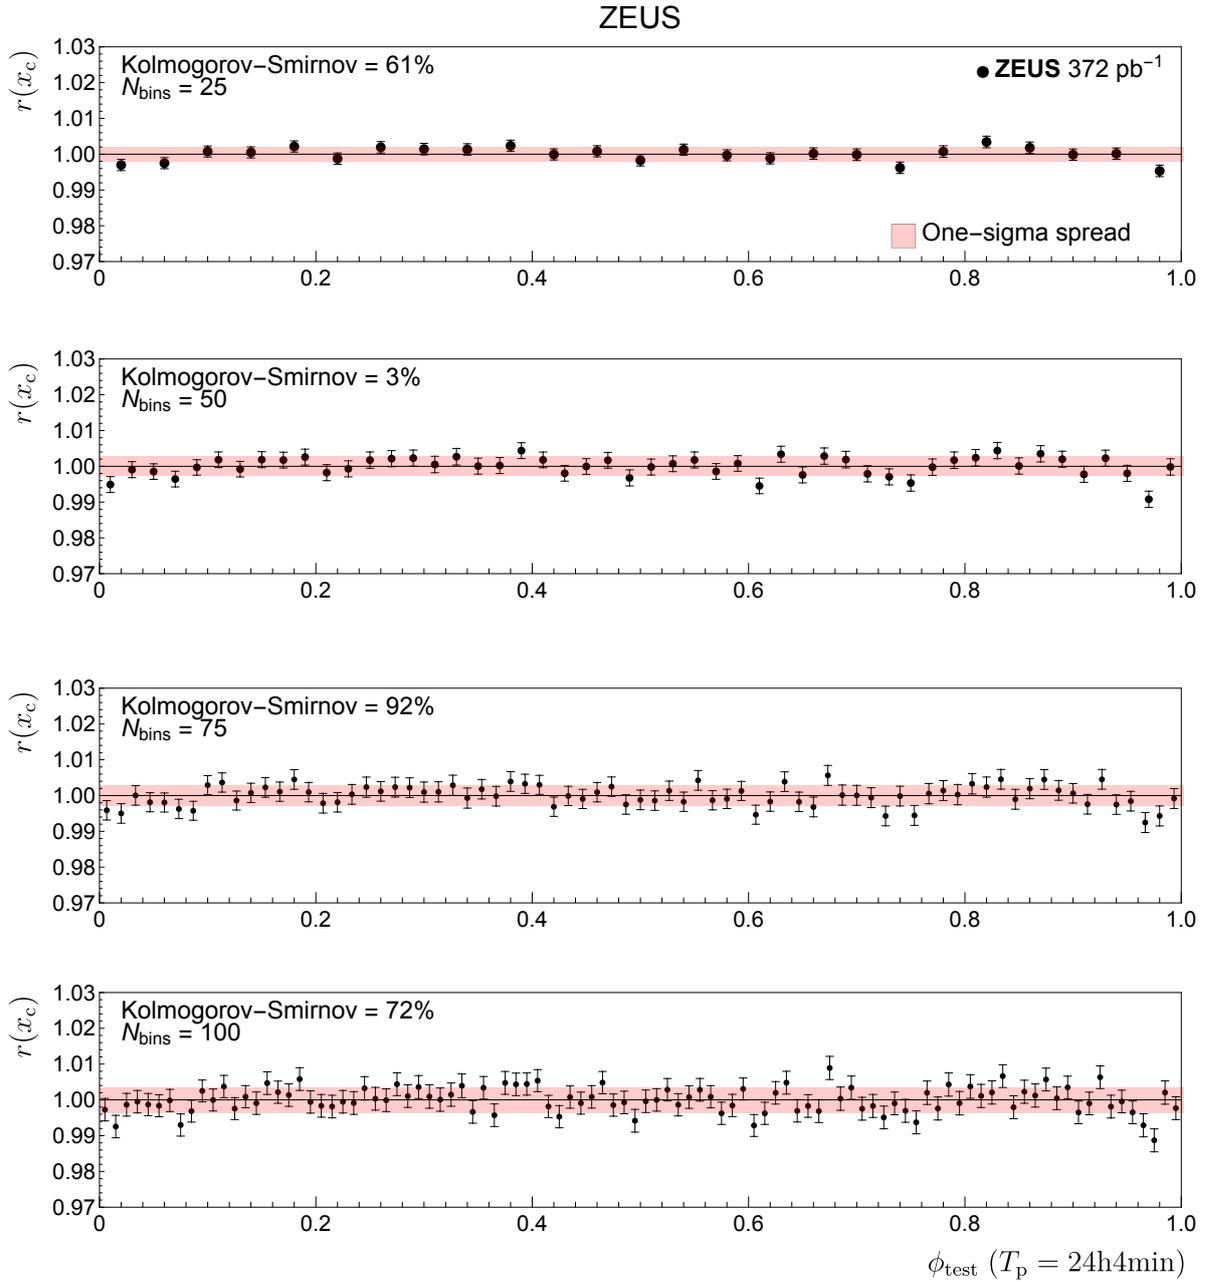

**Figure 28:** Ratio  $r(x_c)$  of normalised counts for  $x_c = 10^{-3}$  binned with the test phase with  $T_p = 24 \text{ h } 4 \text{ min}$  where  $N_{\text{bins}} = 25, 50, 75$  and  $100$ . The displayed uncertainties include statistical uncertainties only and the one-sigma spreads (bands) are the standard deviations of the central values. The observed distributions are compared to a Gaussian distribution in which only statistical errors are included using a Kolmogorov-Smirnov test.

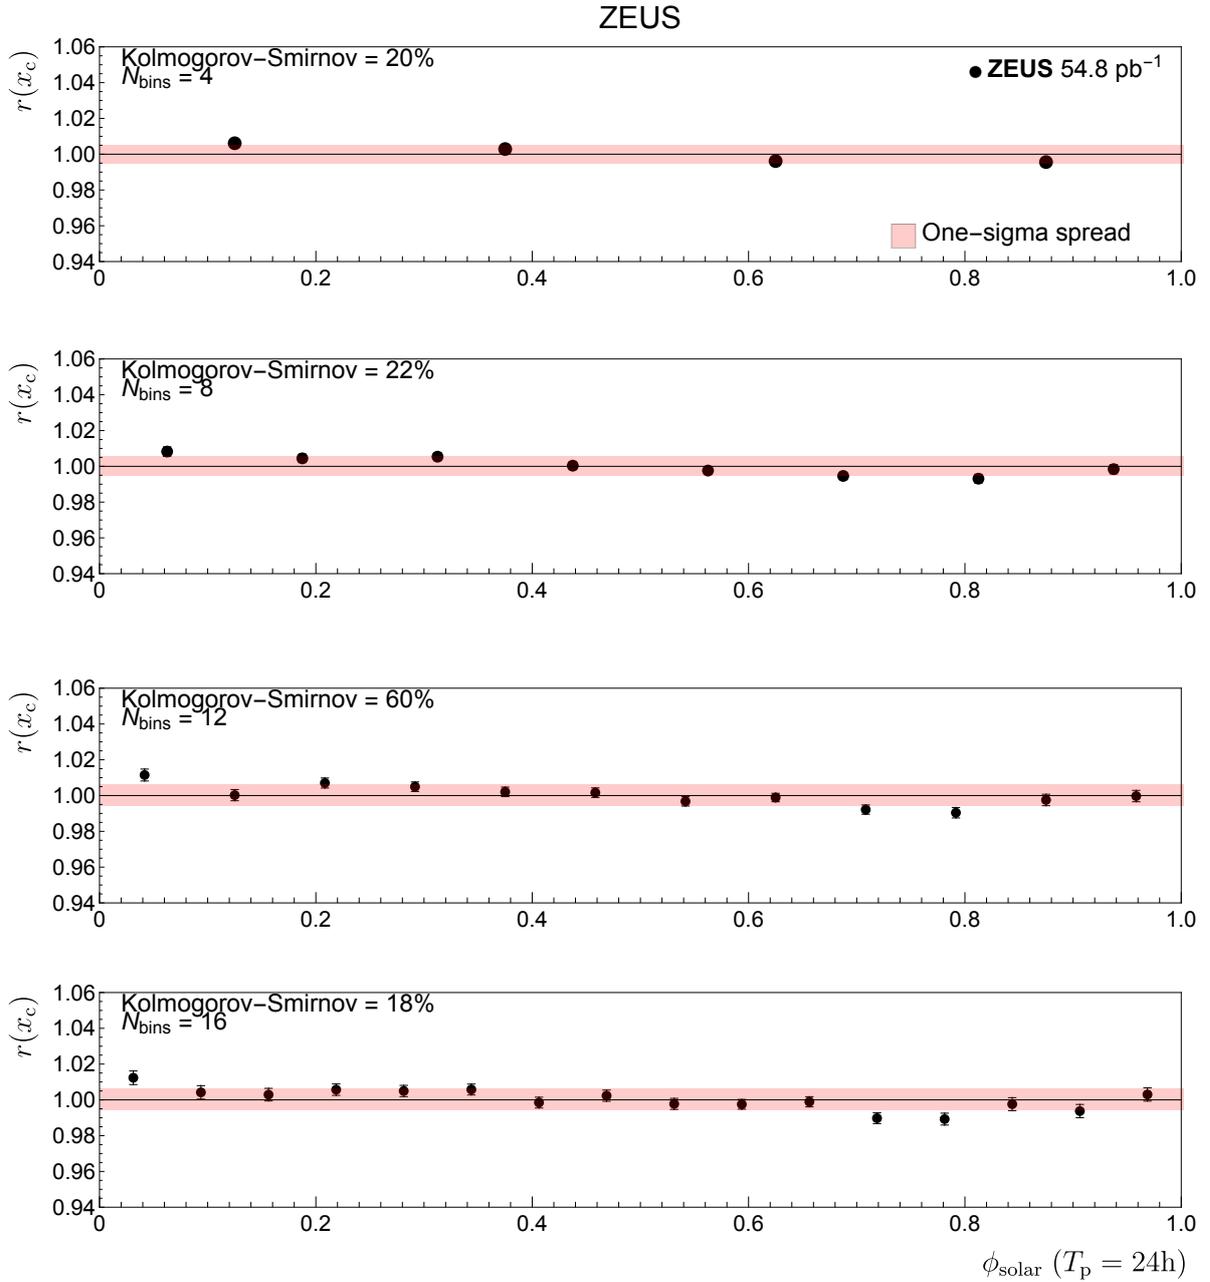

**Figure 29:** Ratio  $r(x_c)$  of normalised counts for  $x_c = 10^{-3}$  binned with the solar phase where  $N_{\text{bins}} = 4, 8, 12$  and  $16$ , using 2006 electron data. The displayed uncertainties include statistical uncertainties only and the one-sigma spreads (bands) are the standard deviations of the central values. The observed distributions are compared to a Gaussian distribution in which only statistical errors are included using a Kolmogorov-Smirnov test.

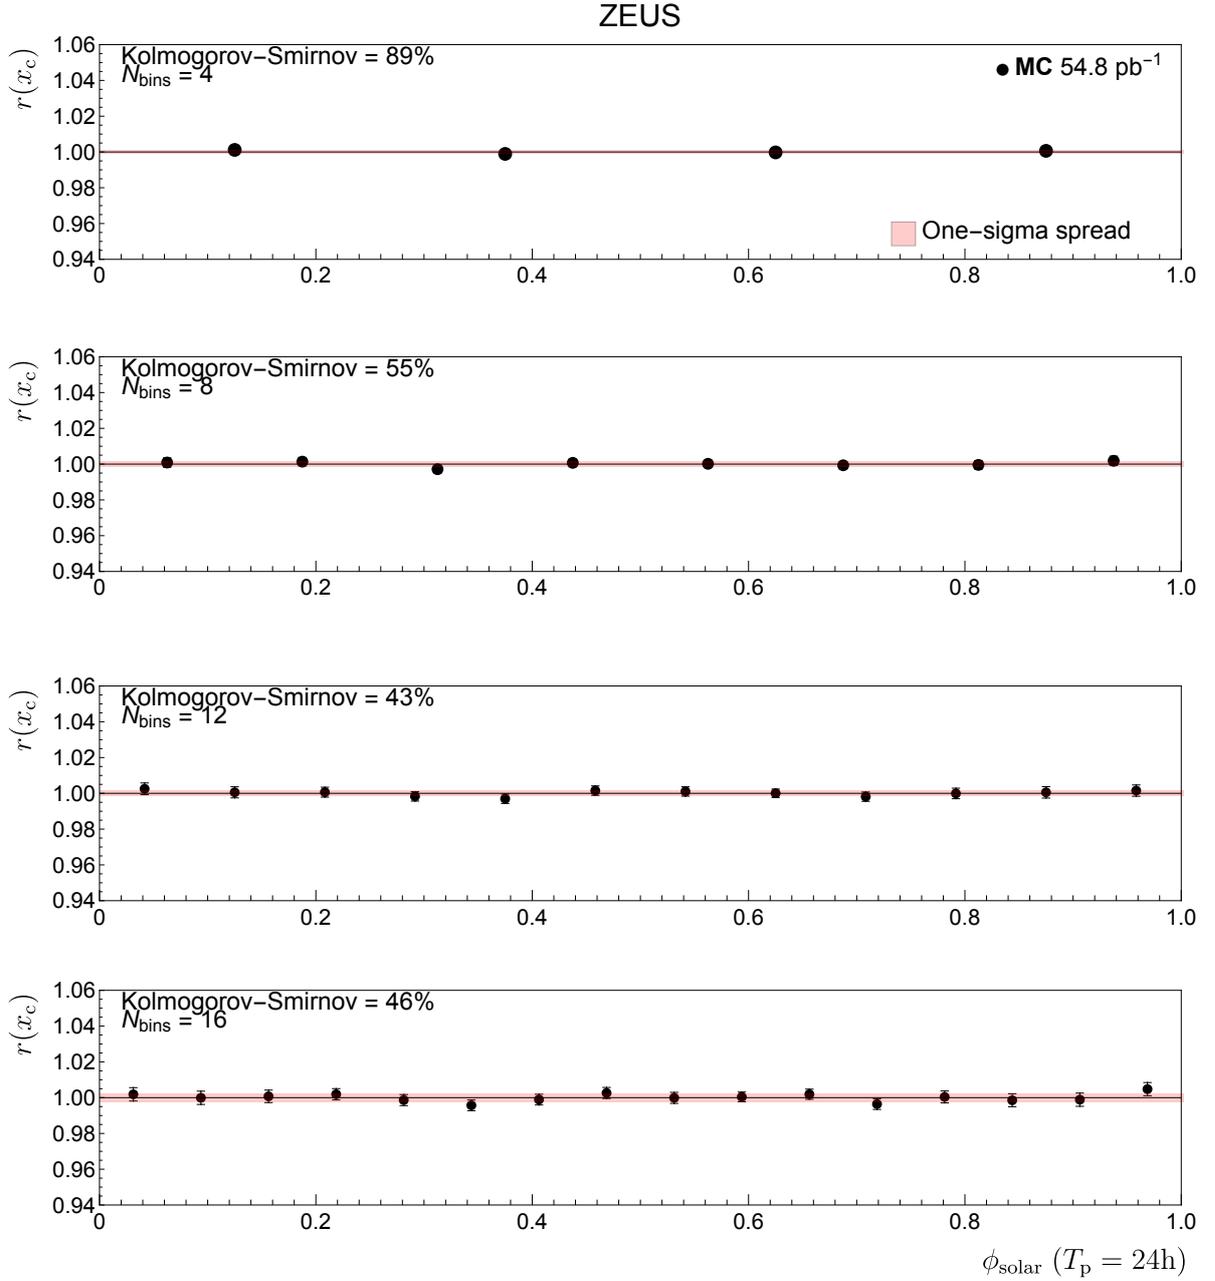

**Figure 30:** Ratio  $r(x_c)$  of normalised counts for  $x_c = 10^{-3}$  binned with the solar phase where  $N_{\text{bins}} = 4, 8, 12$  and  $16$ , obtained using Monte Carlo simulated data that correspond to the 2006 electron data. The displayed uncertainties include statistical uncertainties only and the one-sigma spreads (bands) are the standard deviations of the central values. The observed distributions are compared to a Gaussian distribution in which only statistical errors are included using a Kolmogorov-Smirnov test.

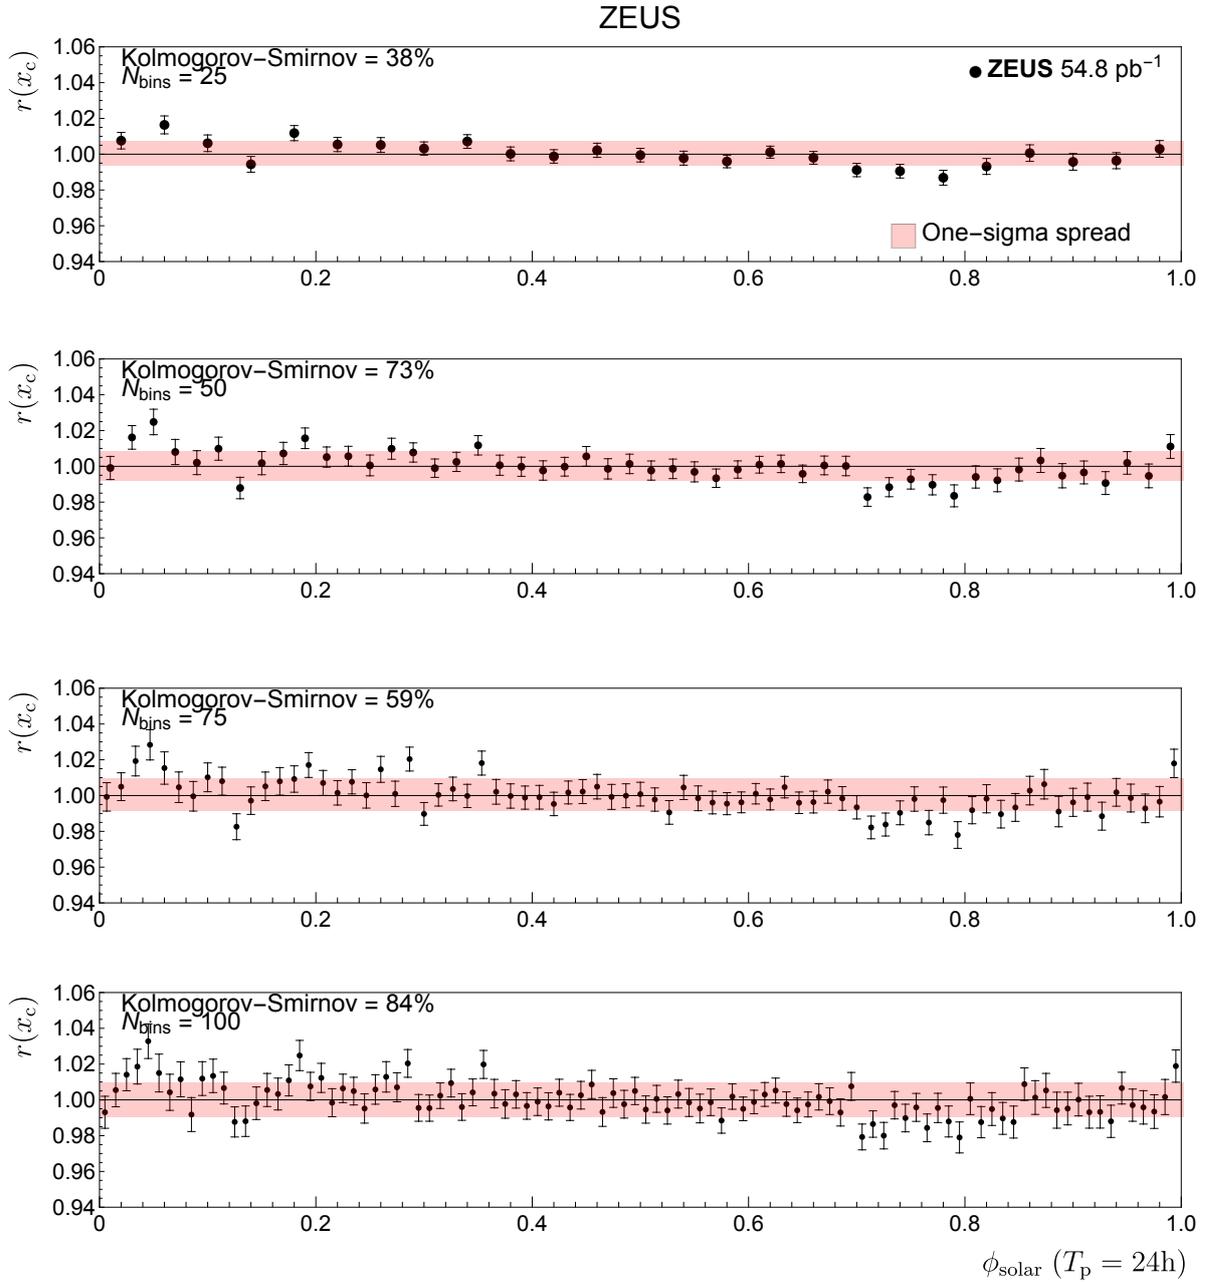

**Figure 31:** Ratio  $r(x_c)$  of normalised counts for  $x_c = 10^{-3}$  binned with the solar phase where  $N_{\text{bins}} = 25, 50, 75$  and  $100$ , using 2006 electron data. The displayed uncertainties include statistical uncertainties only and the one-sigma spreads (bands) are the standard deviations of the central values. The observed distributions are compared to a Gaussian distribution in which only statistical errors are included using a Kolmogorov–Smirnov test.

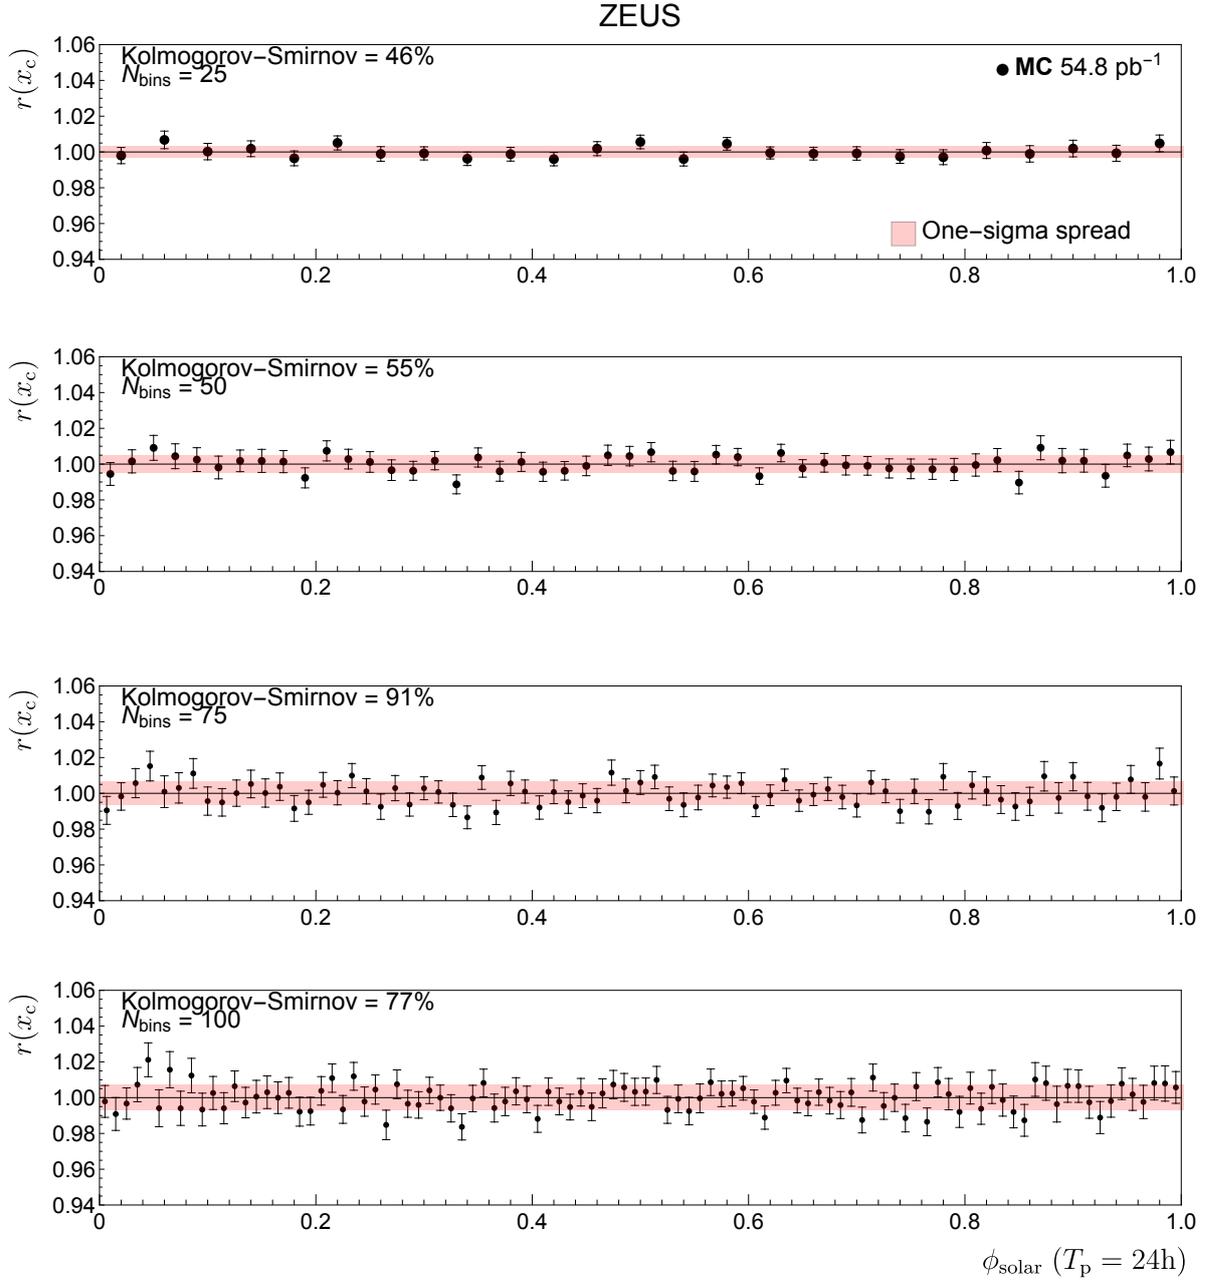

**Figure 32:** Ratio  $r(x_c)$  of normalised counts for  $x_c = 10^{-3}$  binned with the solar phase where  $N_{\text{bins}} = 25, 50, 75$  and  $100$ , obtained using Monte Carlo simulated data that correspond to the 2006 electron data. The displayed uncertainties include statistical uncertainties only and the one-sigma spreads (bands) are the standard deviations of the central values. The observed distributions are compared to a Gaussian distribution in which only statistical errors are included using a Kolmogorov-Smirnov test.

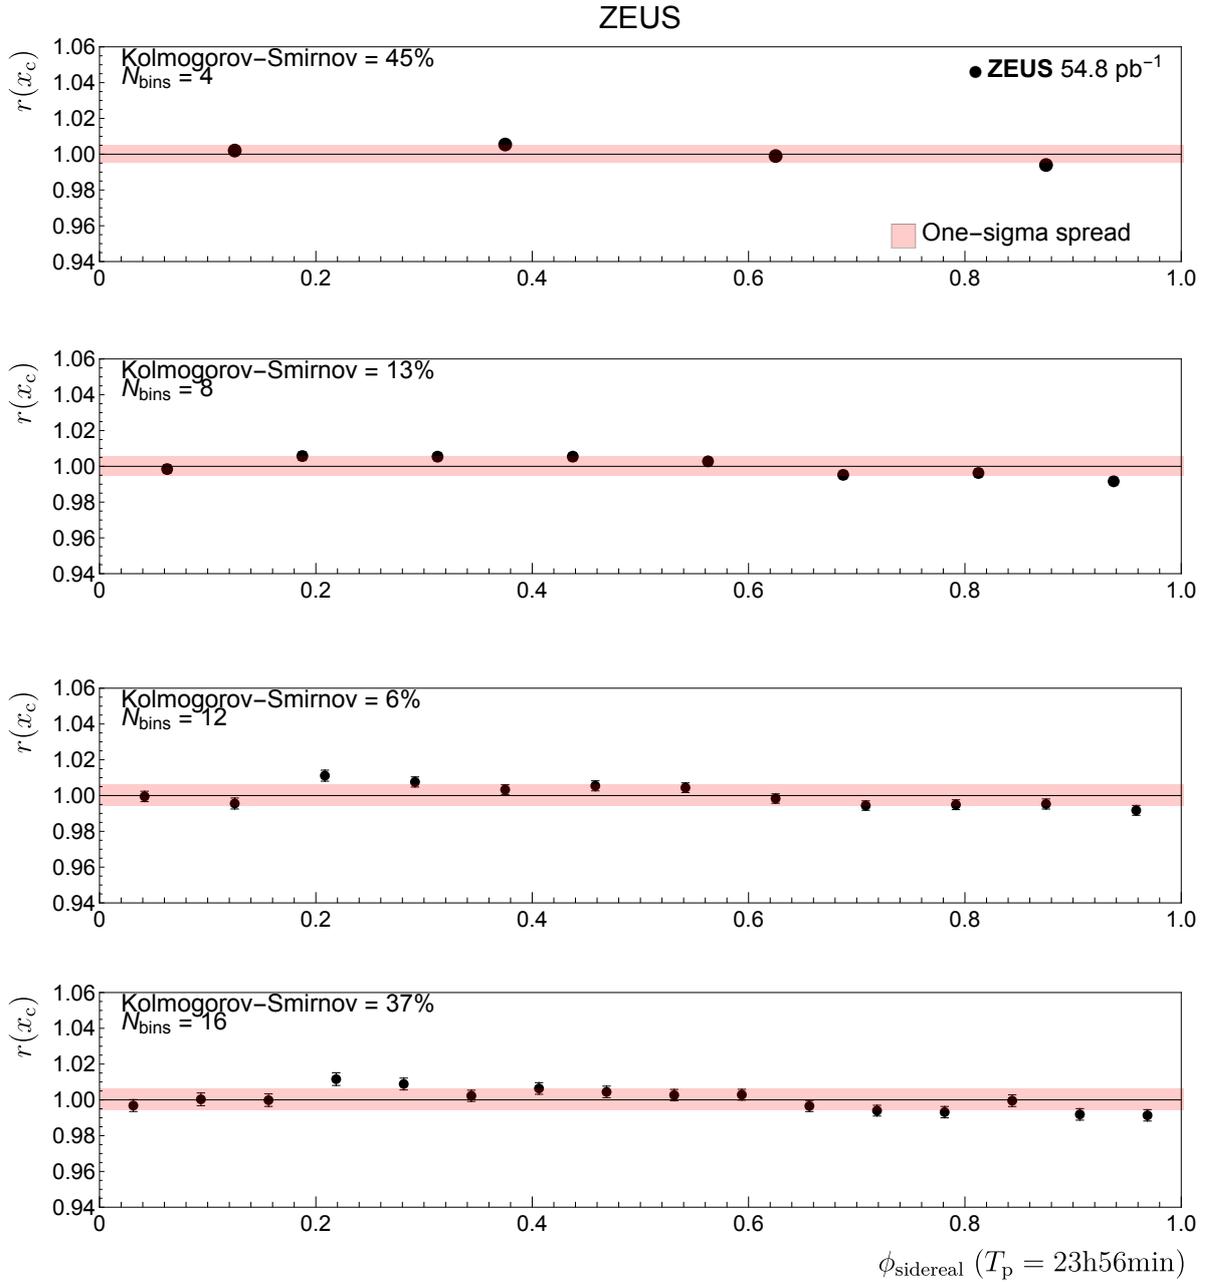

**Figure 33:** Ratio  $r(x_c)$  of normalised counts for  $x_c = 10^{-3}$  binned with the sidereal phase where  $N_{\text{bins}} = 4, 8, 12$  and  $16$ , using 2006 electron data. The displayed uncertainties include statistical uncertainties only and the one-sigma spreads (bands) are the standard deviations of the central values. The observed distributions are compared to a Gaussian distribution in which only statistical errors are included using a Kolmogorov-Smirnov test.

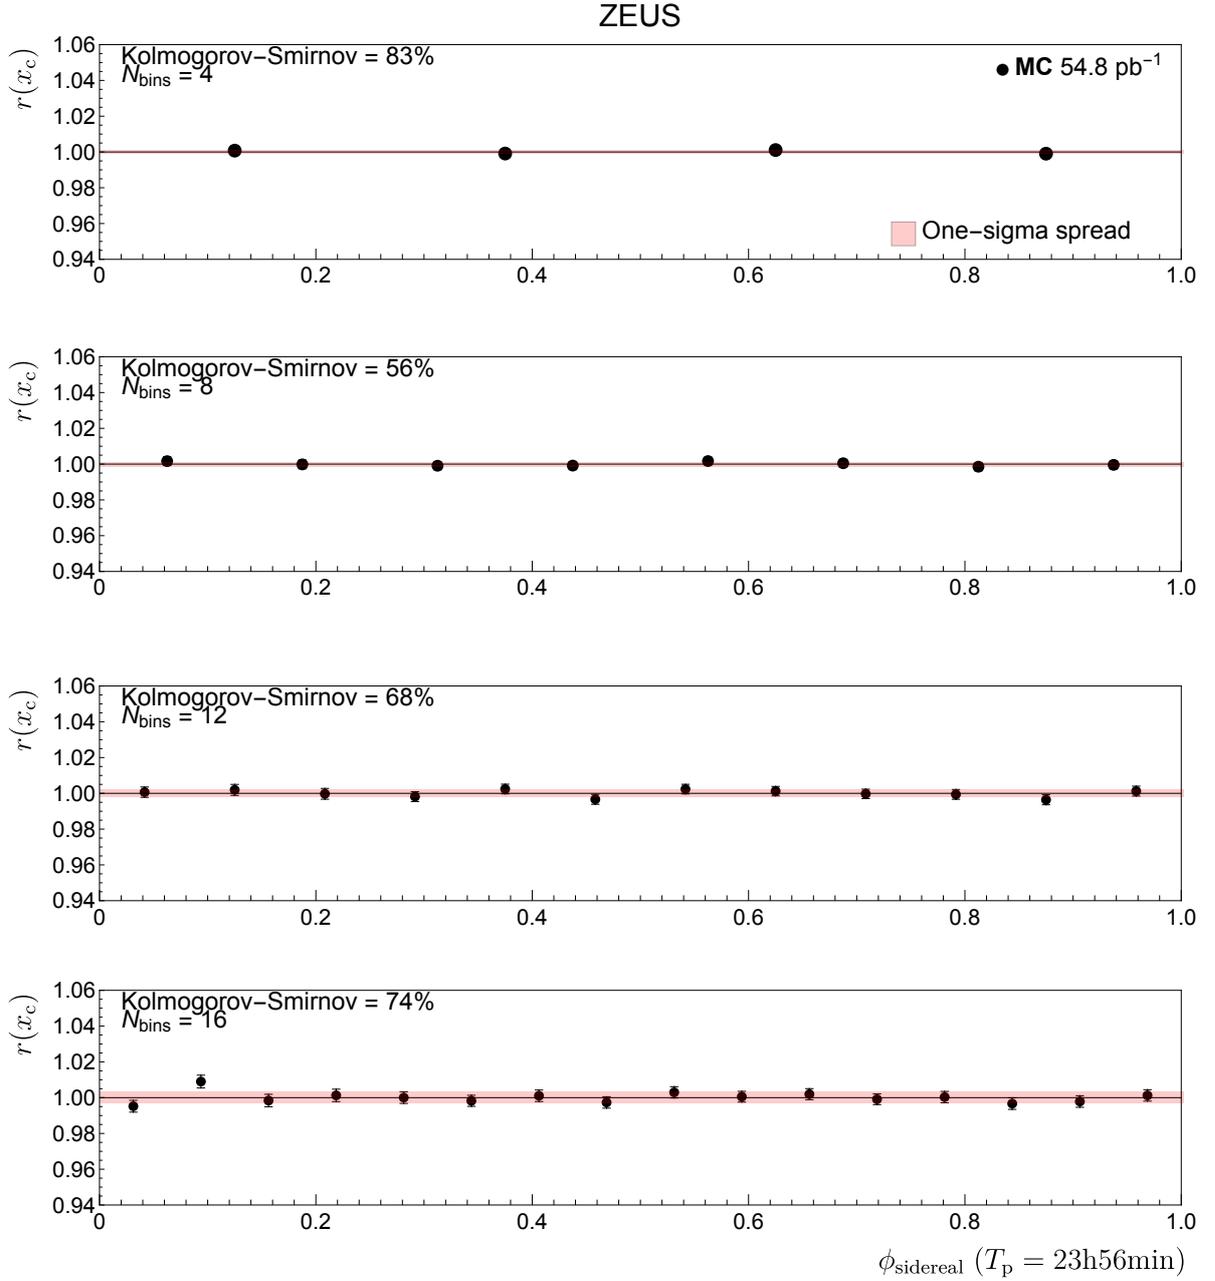

**Figure 34:** Ratio  $r(x_c)$  of normalised counts for  $x_c = 10^{-3}$  binned with the sidereal phase where  $N_{\text{bins}} = 4, 8, 12$  and  $16$ , obtained using Monte Carlo simulated data that correspond to the 2006 electron data. The displayed uncertainties include statistical uncertainties only and the one-sigma spreads (bands) are the standard deviations of the central values. The observed distributions are compared to a Gaussian distribution in which only statistical errors are included using a Kolmogorov-Smirnov test.

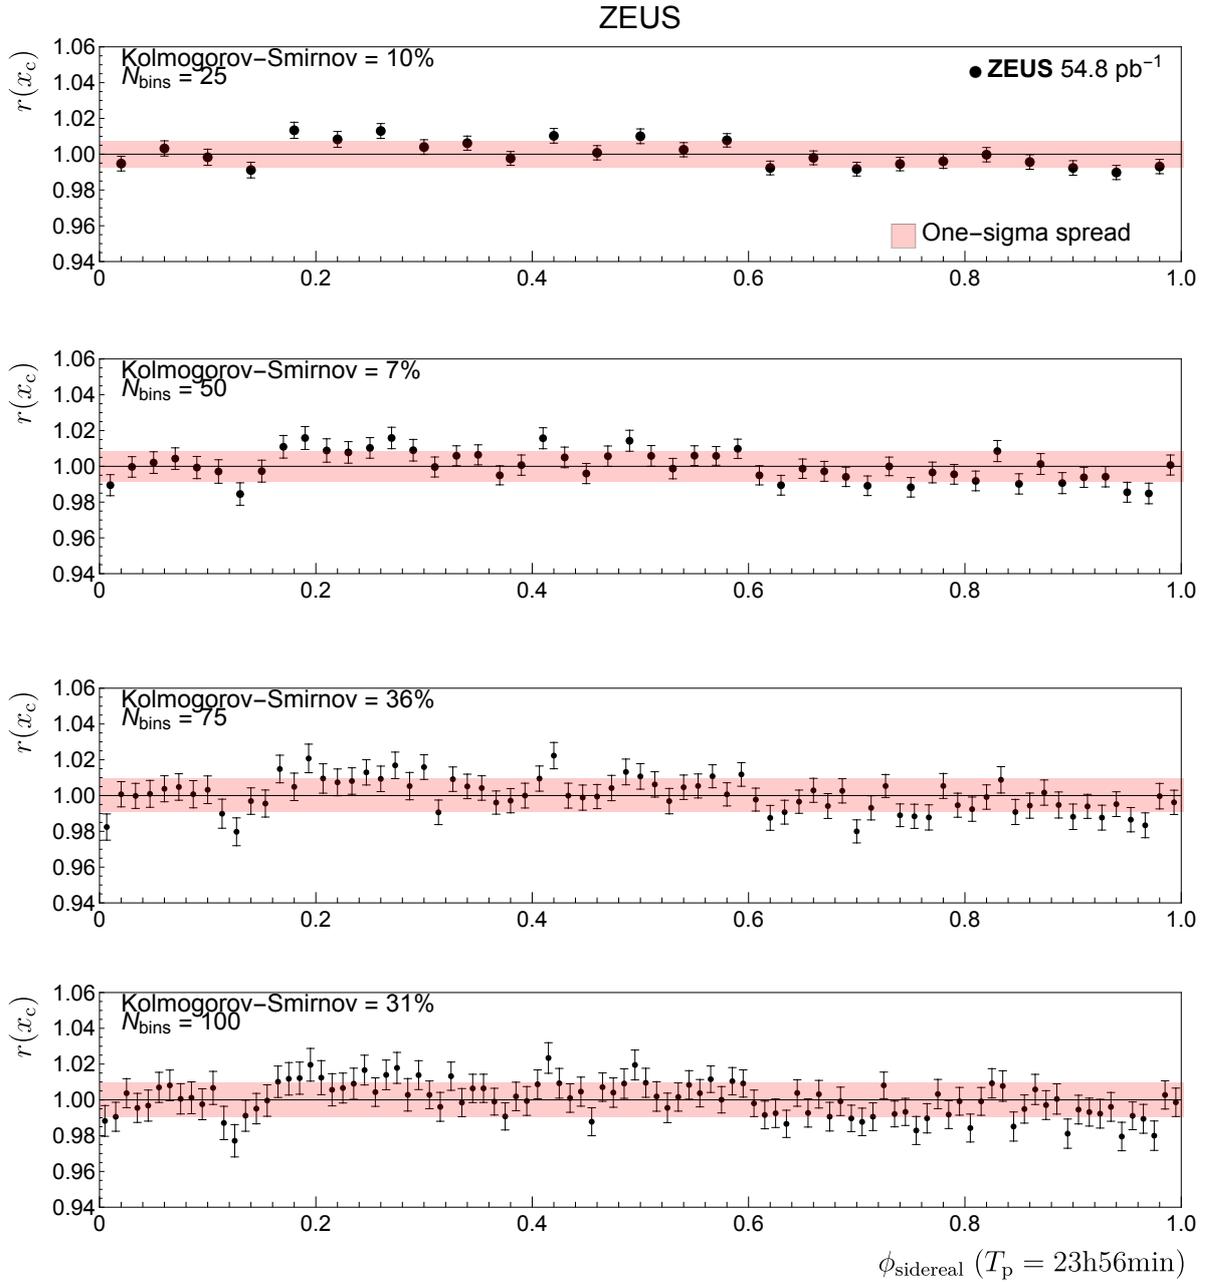

**Figure 35:** Ratio  $r(x_c)$  of normalised counts for  $x_c = 10^{-3}$  binned with the sidereal phase where  $N_{\text{bins}} = 25, 50, 75$  and  $100$ , using 2006 electron data. The displayed uncertainties include statistical uncertainties only and the one-sigma spreads (bands) are the standard deviations of the central values. The observed distributions are compared to a Gaussian distribution in which only statistical errors are included using a Kolmogorov–Smirnov test.

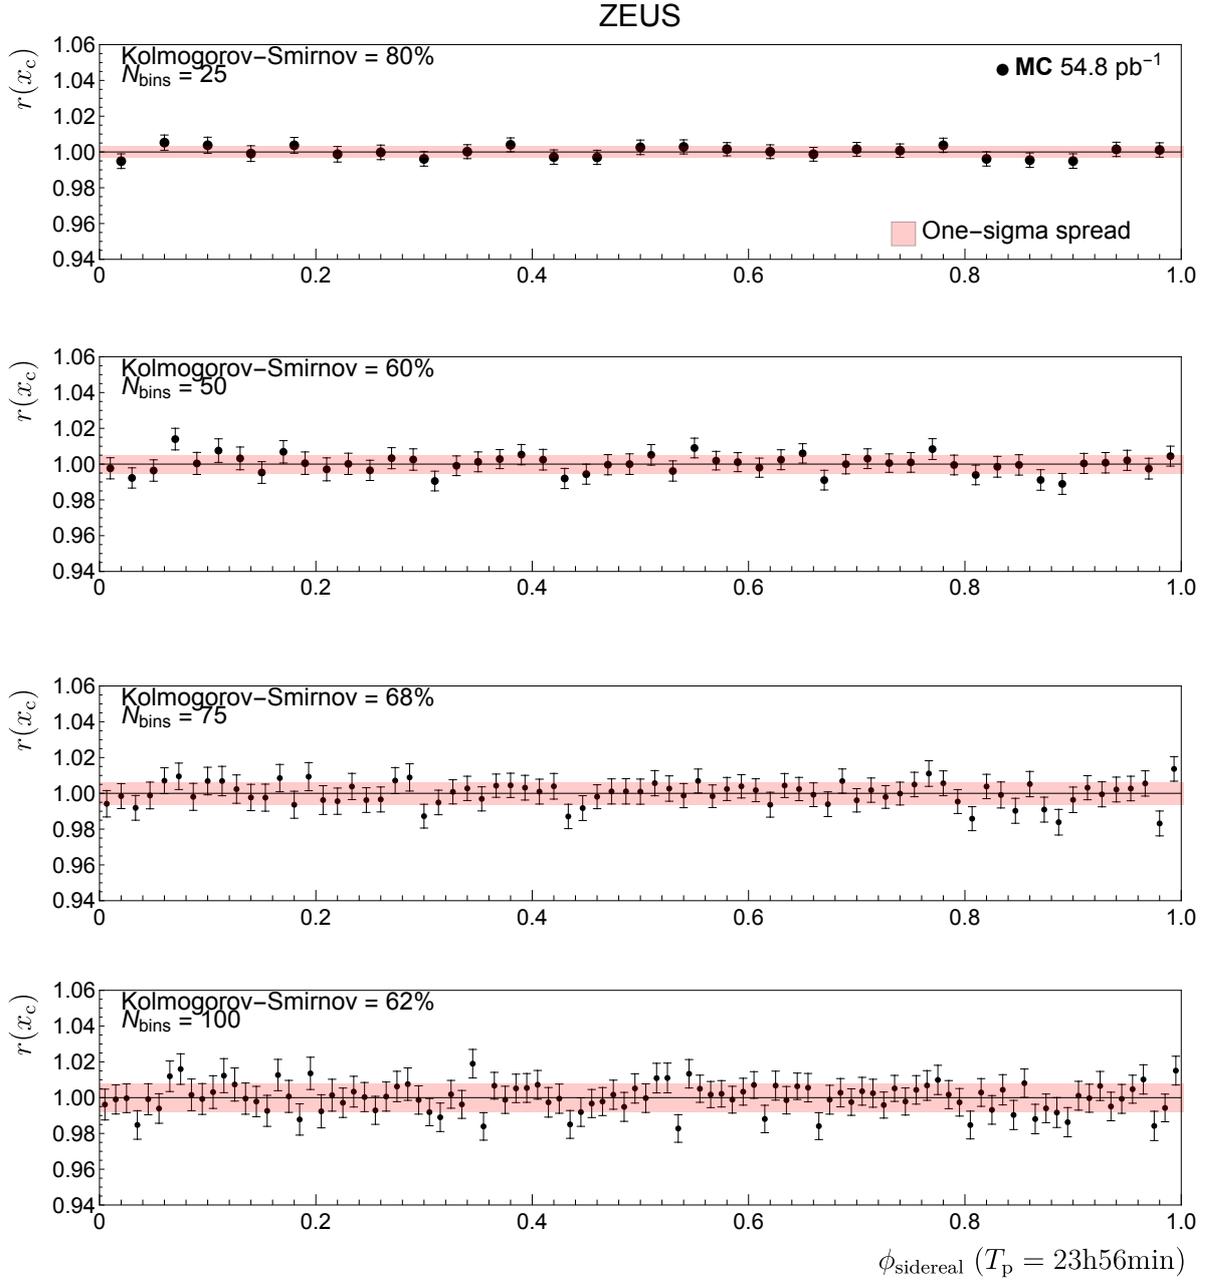

**Figure 36:** Ratio  $r(x_c)$  of normalised counts for  $x_c = 10^{-3}$  binned with the sidereal phase where  $N_{\text{bins}} = 25, 50, 75$  and  $100$ , obtained using Monte Carlo simulated data that correspond to the 2006 electron data. The displayed uncertainties include statistical uncertainties only and the one-sigma spreads (bands) are the standard deviations of the central values. The observed distributions are compared to a Gaussian distribution in which only statistical errors are included using a Kolmogorov-Smirnov test.

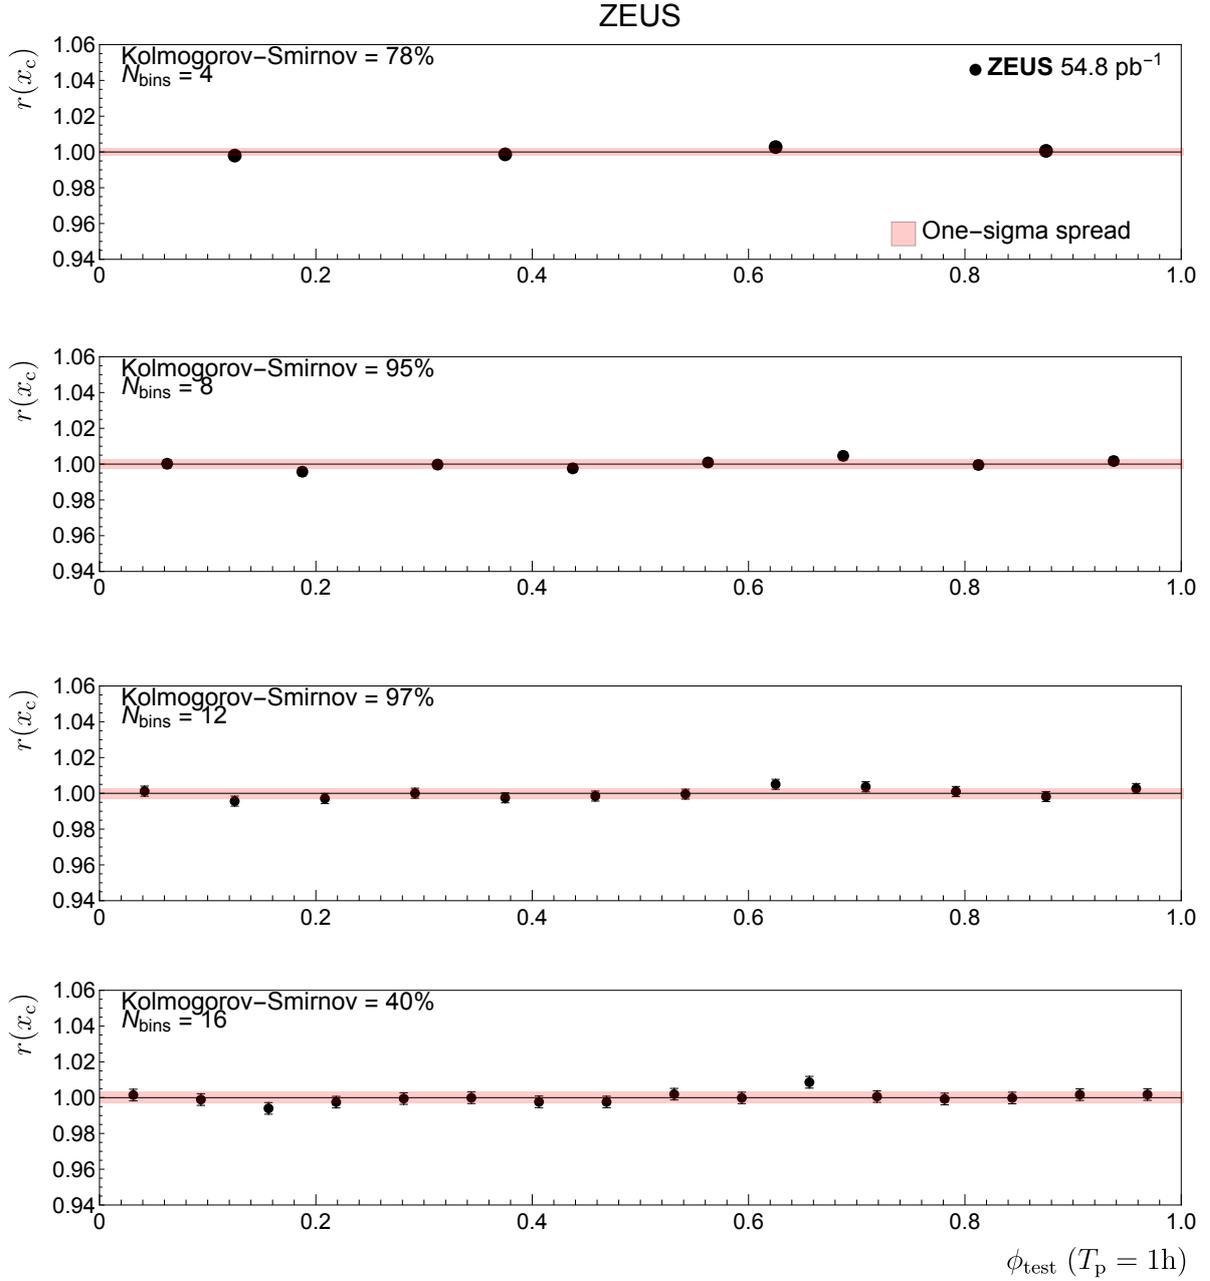

**Figure 37:** Ratio  $r(x_c)$  of normalised counts for  $x_c = 10^{-3}$  binned with the test phase with  $T_p = 1$  h where  $N_{\text{bins}} = 4, 8, 12$  and  $16$ , using 2006 electron data. The displayed uncertainties include statistical uncertainties only and the one-sigma spreads (bands) are the standard deviations of the central values. The observed distributions are compared to a Gaussian distribution in which only statistical errors are included using a Kolmogorov-Smirnov test.

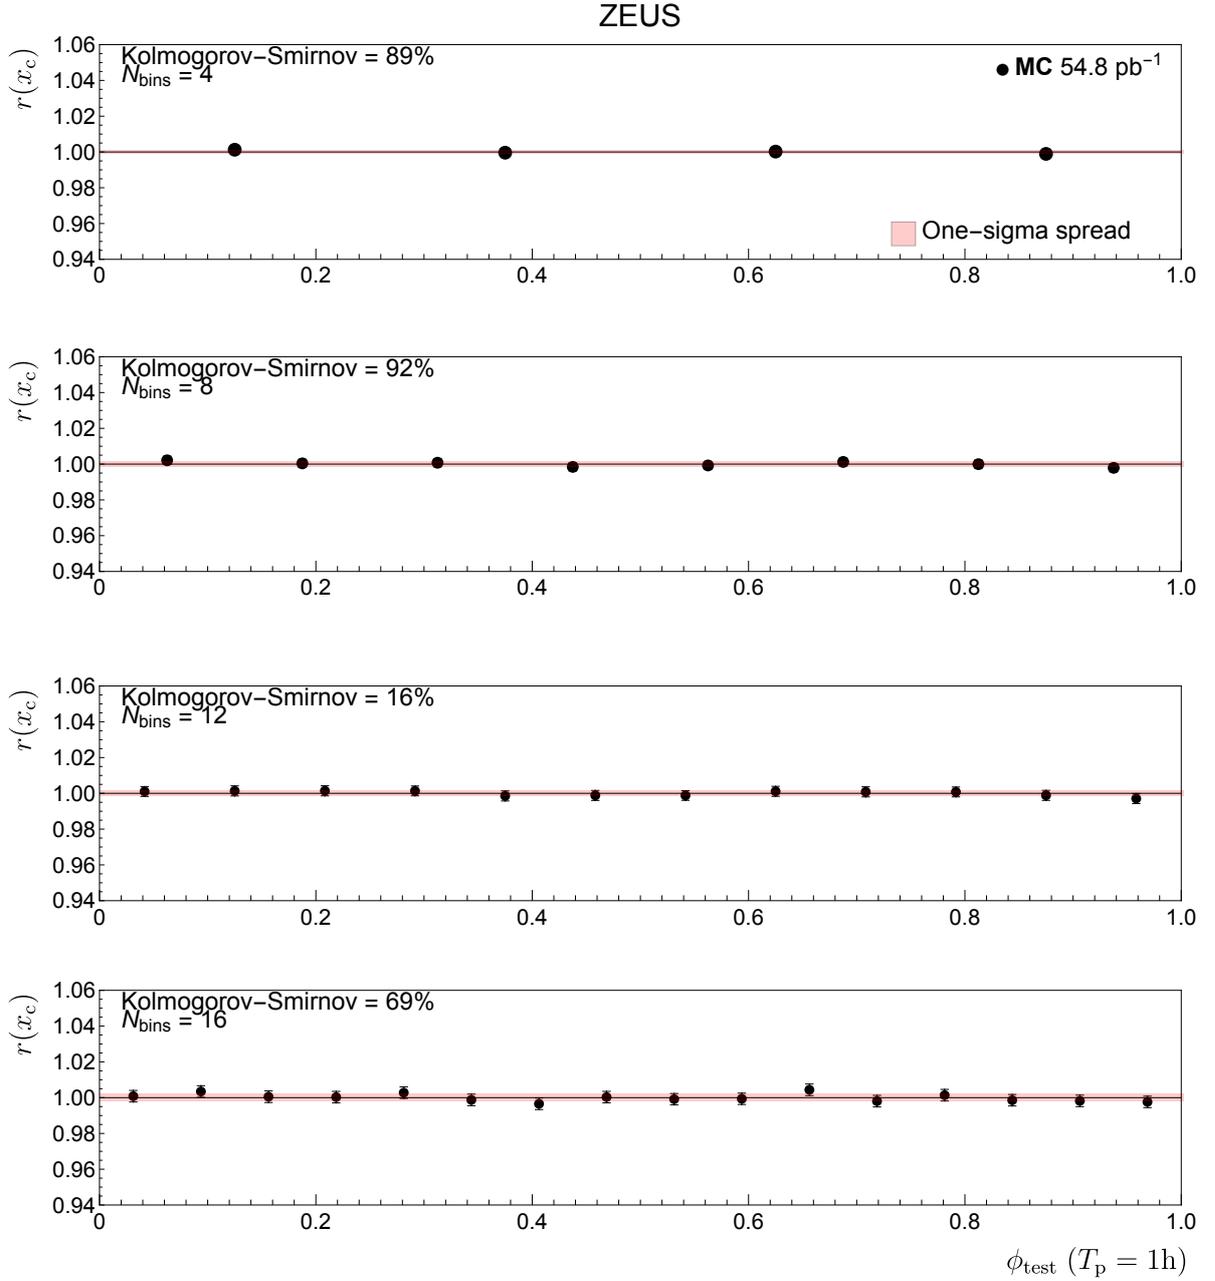

**Figure 38:** Ratio  $r(x_c)$  of normalised counts for  $x_c = 10^{-3}$  binned with the test phase with  $T_p = 1$  h where  $N_{\text{bins}} = 4, 8, 12$  and  $16$ , obtained using Monte Carlo simulated data that correspond to the 2006 electron data. The displayed uncertainties include statistical uncertainties only and the one-sigma spreads (bands) are the standard deviations of the central values. The observed distributions are compared to a Gaussian distribution in which only statistical errors are included using a Kolmogorov-Smirnov test.

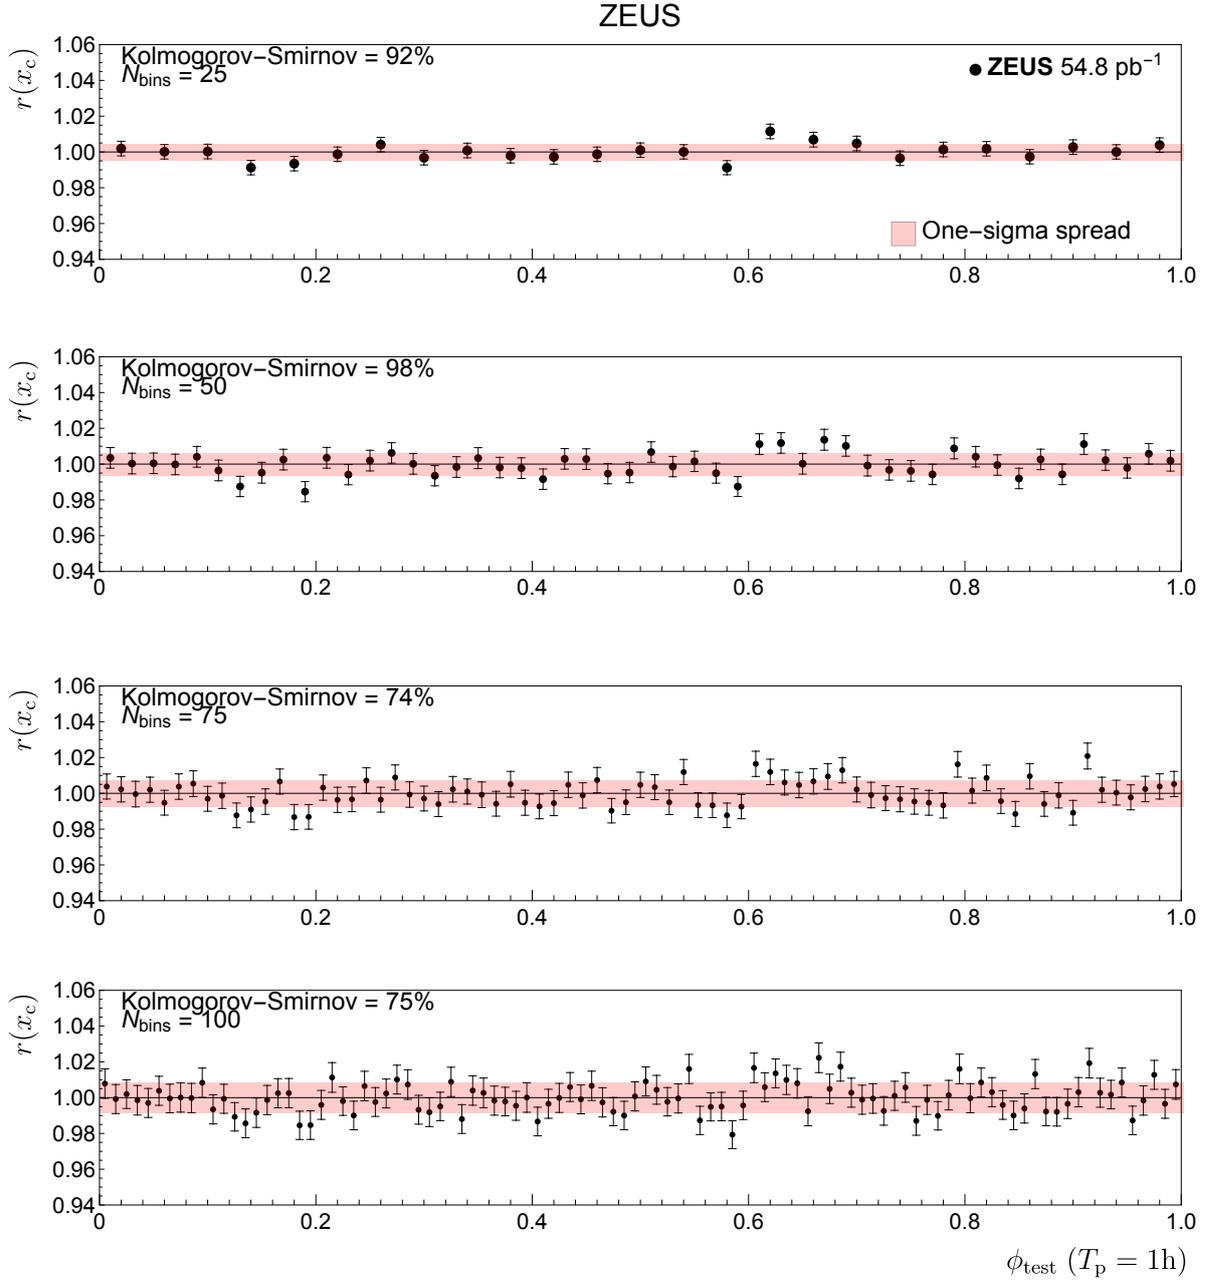

**Figure 39:** Ratio  $r(x_c)$  of normalised counts for  $x_c = 10^{-3}$  binned with the test phase with  $T_p = 1$  h where  $N_{\text{bins}} = 25, 50, 75$  and  $100$ , using 2006 electron data. The displayed uncertainties include statistical uncertainties only and the one-sigma spreads (bands) are the standard deviations of the central values. The observed distributions are compared to a Gaussian distribution in which only statistical errors are included using a Kolmogorov-Smirnov test.

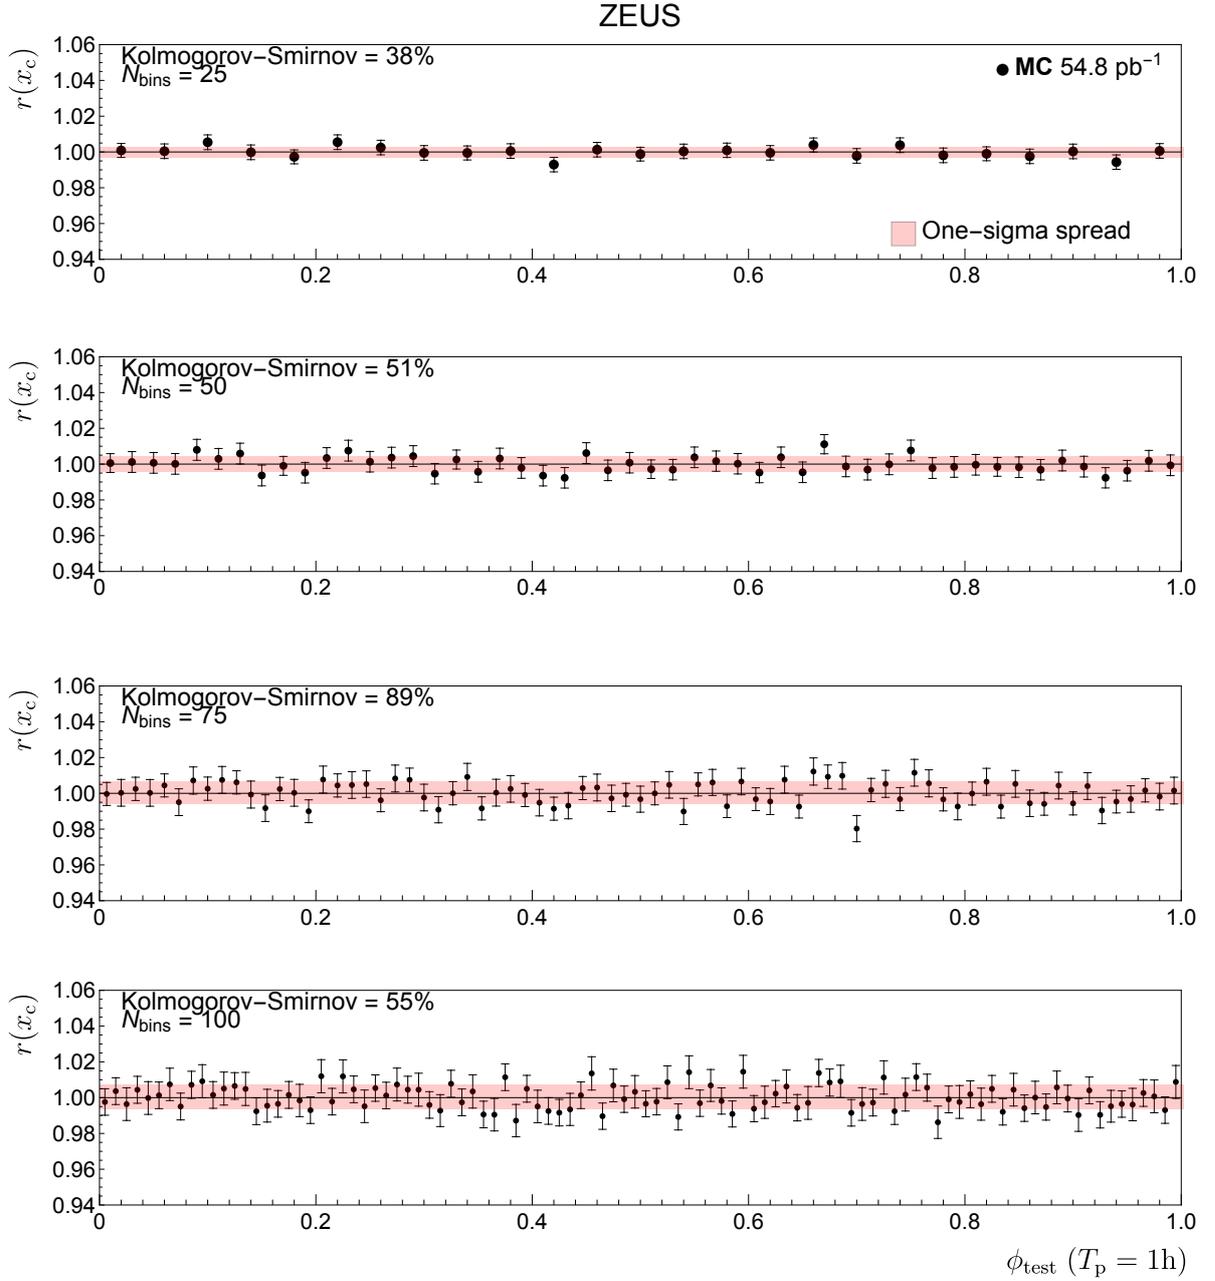

**Figure 40:** Ratio  $r(x_c)$  of normalised counts for  $x_c = 10^{-3}$  binned with the test phase with  $T_p = 1\text{ h}$  where  $N_{\text{bins}} = 25, 50, 75$  and  $100$ , obtained using Monte Carlo simulated data that correspond to the 2006 electron data. The displayed uncertainties include statistical uncertainties only and the one-sigma spreads (bands) are the standard deviations of the central values. The observed distributions are compared to a Gaussian distribution in which only statistical errors are included using a Kolmogorov-Smirnov test.
